# Supplementary material for: Zero Variance Portfolio
Source: arXiv:2602.19462 source file (2026-11-02)
Supplement: Supplementary file 1 [file MVP_RMT_supp.pdf]

# Supplementary file for “Zero Variance Portfolio”

We provide the strengthened versions of the theorems in the main text along with their proofs in the supplementary materials, from which the theorems in the main text naturally follow. In Section S.1, we present these strengthened theorems and illustrate how the main-text theorems can be derived therefrom. Section S.2 outlines the basic expansions of the numerator and denominator of  $\mathbb{V}(\hat{\omega}_\tau)$ , based on which the key objectives of the proofs are clarified. In Sections S.3–S.4, we demonstrate the theoretical proofs in the regime  $N/T \rightarrow \gamma \in (1, \infty)$  and  $N/T \rightarrow \infty$ , while Section S.5 is dedicated to the theoretical proofs in the regime  $N/T \rightarrow \gamma \in (0, 1)$ . Section S.6 discusses the impacts of the difference between  $\mathbf{\Omega}$  and  $\mathbf{I}_N$ . In Section S.7, we establish the theoretical properties of the infeasible estimator  $\tilde{\omega}_\tau^{\text{ifs}}$ , and Section S.8 verifies those of the feasible estimator  $\tilde{\omega}_\tau$ . Finally, Sections S.9–S.10 provide several useful computational results.

## S.1 Strengthened versions for theoretical results

This section presents the strengthened versions of the theorems in the main text. These versions cover more general cases (including the scenario where  $N/T \rightarrow \gamma \in (1, \infty)$ ) and provide more refined expressions, from which the theorems in the main text will naturally follow.

Recall the model of  $r$  factors

$$\mathbf{R} = \mathbf{B}\mathbf{F} + \mathbf{E} = \mathbf{B}\mathbf{F} + \mathbf{\Omega}^{1/2}\mathbf{Z}, \quad (\text{S.1.1})$$

where  $\mathbf{B}$  is the  $N \times r$  matrix,  $\mathbf{F}$  is the  $r \times T$  matrix satisfying  $\mathbb{E}(T^{-1}\mathbf{F}^\top\mathbf{F}) = \mathbf{I}_r$ .

$$\mathbf{B}\mathbf{B}^\top = \mathbf{V} \text{diag}(\lambda_{B,1}, \dots, \lambda_{B,r})\mathbf{V}^\top.$$

Assumptions 1-2 show that

- (i). The idiosyncratic shock  $\mathbf{E} = \mathbf{\Omega}^{1/2}\mathbf{Z}$ , where the minimum eigenvalue and maximum eigenvalue of  $\mathbf{\Omega}$  is bounded away from zero and infinity. Let  $\mathbf{Z}$  be an  $N \times T$  matrix consisting of i.i.d. standard Gaussian entries.
- (ii).  $\lambda_{B,1} \asymp \lambda_{B,r} \asymp N^\delta$  for some  $\delta \in (0, 1]$  and  $N^\delta \gg 1 + N/T$ .
- (iii).  $\|\mathbf{P}_V^\perp \mathbf{1}\|/\sqrt{N} \gg \sqrt{N^{(1-\delta)}/T}$ .
- (iv).  $\tau = o(\|\mathbf{P}_V^\perp \mathbf{1}\|/\sqrt{N})$ .

The population covariance of  $\mathbf{R}$  is

$$\mathbf{\Sigma} = \mathbf{B}\mathbf{B}^\top + \mathbf{\Omega}.$$

**Definition S.1** (*Stieltjes transform*) Let  $\mu(x)$  be the limiting spectral distribution of  $T^{-1}\mathbf{Z}^\top \mathbf{\Omega} \mathbf{Z}$ .

$$m(z) = \int_{\mathbb{R}} \frac{1}{x - z} d\mu(x) \tag{S.1.2}$$

is the Stieltjes transform of  $\mu(x)$ .

We define

$$\tilde{\mathbf{1}}_\tau = (\mathbf{I}_N - \mathbf{P}_{[\mathbf{I}_N + m(-\tau)\mathbf{\Omega}]^{-\frac{1}{2}}\mathbf{V}})[\mathbf{I}_N + m(-\tau)\mathbf{\Omega}]^{-\frac{1}{2}}\mathbf{1} \tag{S.1.3}$$

$$\check{\mathbf{1}}_\tau = [m(-\tau)\mathbf{\Omega} + \mathbf{I}_N]^{-\frac{1}{2}}\mathbf{\Omega}^{\frac{1}{2}}\tilde{\mathbf{1}}_\tau \tag{S.1.4}$$

$$c(\tau) = \frac{1}{1 - T^{-1}m^2(-\tau)\text{tr}\{\mathbf{\Omega}[\mathbf{I}_N + m(-\tau)\mathbf{\Omega}]^{-2}\mathbf{\Omega}\}}, \tag{S.1.5}$$

$$d(\mathbf{\Omega}) = \|[\mathbf{\Omega} - N^{-1}\text{tr}(\mathbf{\Omega})\mathbf{I}_N]\mathbf{P}_V^\perp\|, \tag{S.1.6}$$

The first result is the limiting behavior of the ridgelet estimator in our  $N > T$  asymptotic regime.

**Theorem S.1** *Suppose Assumptions 1 and 2 hold, and  $N, T \rightarrow \infty$ . If  $N/T \rightarrow \gamma \in (1, \infty)$ ,*

$$\mathbb{V}(\hat{\omega}_\tau) = c(\tau) \frac{\tilde{\mathbf{1}}_\tau^\top \tilde{\mathbf{1}}_\tau}{[\tilde{\mathbf{1}}_\tau^\top \tilde{\mathbf{1}}_\tau]^2} [1 + o_p(1)] \quad (\text{S.1.7})$$

and

$$\mathbb{V}(\hat{\omega}_\tau) = N^{-1} \text{tr}(\mathbf{\Omega}) c(\tau) \frac{1 + O_p(d(\mathbf{\Omega})) + o_p(1)}{[\mathbf{1}^\top \mathbf{P}_V^\perp \mathbf{1}]}. \quad (\text{S.1.8})$$

If  $N/T \rightarrow \gamma \in (1, \infty)$  and  $\mathbf{\Omega} = \sigma^2 \mathbf{I}_N$  for  $0 < \sigma^2 < \infty$ ,

$$\mathbb{V}(\hat{\omega}_\tau) = \frac{\gamma}{\gamma - 1} [\mathbf{1}^\top \mathbf{\Sigma}^{-1} \mathbf{1}]^{-1} [1 + o_p(1)]. \quad (\text{S.1.9})$$

If  $N/T \rightarrow \infty$ ,

$$\mathbb{V}(\hat{\omega}_\tau) = \frac{\mathbf{1}^\top \mathbf{P}_V^\perp \mathbf{\Omega} \mathbf{P}_V^\perp \mathbf{1}}{[\mathbf{1}^\top \mathbf{P}_V^\perp \mathbf{1}]^2} [1 + O_p(TN^{-1}) + o_p(1)]. \quad (\text{S.1.10})$$

(S.1.10) implies the results of (iii) in Theorem 1. When  $\mathbf{\Omega} = \mathbf{I}_N$ , (S.1.10) also shows that  $\mathbb{R}\mathbb{V}(\hat{\omega}_\tau) \xrightarrow{p} 1$  due to  $\mathbf{1}^\top \mathbf{\Sigma}^{-1} \mathbf{1} = \mathbf{1}^\top \mathbf{P}_V^\perp \mathbf{1} [1 + o(1)]$  (see (S.2.5)). Thus, we prove (iii) in Theorem 1.

(S.1.7)-(S.1.9) show the results of (ii) in Theorem 1. (S.1.7) is a more accurate asymptotic expression for  $\mathbb{V}(\hat{\omega}_\tau)$  with additional definitions. (S.1.8) implies that the difference between  $\mathbf{\Omega}$  and  $\mathbf{I}_N$  play an important role. (S.1.9) highlights the rapid second descent to the right of  $\gamma = 1$  under the special case  $\mathbf{\Omega} = \sigma^2 \mathbf{I}_N$ .

**Theorem S.2** *Suppose Assumptions 1 and 2 hold, and  $N, T \rightarrow \infty$ . If  $N/T \rightarrow \gamma \in (0, 1)$ ,*

$$\mathbb{V}(\hat{\omega}) = \frac{\mathbf{1}^\top \mathbf{S}_0^{-1} \mathbf{\Sigma} \mathbf{S}_0^{-1} \mathbf{1}}{[\mathbf{1}^\top \mathbf{S}_0^{-1} \mathbf{1}]^2} = \frac{1}{1 - \gamma} (\mathbf{1}^\top \mathbf{\Sigma}^{-1} \mathbf{1})^{-1} [1 + o_p(1)]. \quad (\text{S.1.11})$$

$$\mathbb{V}(\widehat{\omega}_\tau) = \frac{\mathbf{1}^\top \mathbf{S}_\tau^{-1} \boldsymbol{\Sigma} \mathbf{S}_\tau^{-1} \mathbf{1}}{[\mathbf{1}^\top \mathbf{S}_\tau^{-1} \mathbf{1}]^2} = \frac{1}{1 - \gamma} (\mathbf{1}^\top \boldsymbol{\Sigma}^{-1} \mathbf{1})^{-1} [1 + o_p(1)]. \quad (\text{S.1.12})$$

(S.1.11) and (S.1.12) show the results of (i) in Theorem 1 in the main text.

If we replace  $\mathbf{S}_\tau$  by  $\mathbf{S}_{\tau, \Omega} = \tau \boldsymbol{\Omega} + \mathbf{R} \mathbf{R}^\top / T$ , we have the following result.

**Theorem S.3** *Suppose Assumptions 1 and 2 hold, and  $N, T \rightarrow \infty$ . If  $N/T \rightarrow \gamma \in (1, \infty)$ ,*

$$\mathbb{V}(\widetilde{\omega}_\tau^{\text{ifs}}) = \frac{\mathbf{1}^\top \mathbf{S}_{\tau, \Omega}^{-1} \boldsymbol{\Sigma} \mathbf{S}_{\tau, \Omega}^{-1} \mathbf{1}}{[\mathbf{1}^\top \mathbf{S}_{\tau, \Omega}^{-1} \mathbf{1}]^2} = \frac{\gamma[1 + o_p(1)]}{(\gamma - 1) \mathbf{1}^\top \boldsymbol{\Sigma}^{-1} \mathbf{1}}. \quad (\text{S.1.13})$$

If  $N/T \rightarrow \infty$ ,

$$\mathbb{V}(\widetilde{\omega}_\tau^{\text{ifs}}) = \frac{\mathbf{1}^\top \mathbf{S}_{\tau, \Omega}^{-1} \boldsymbol{\Sigma} \mathbf{S}_{\tau, \Omega}^{-1} \mathbf{1}}{[\mathbf{1}^\top \mathbf{S}_{\tau, \Omega}^{-1} \mathbf{1}]^2} = \frac{[1 + O(TN^{-1})][1 + o_p(1)]}{\mathbf{1}^\top \boldsymbol{\Sigma}^{-1} \mathbf{1}}. \quad (\text{S.1.14})$$

(S.1.14) implies the results of (i) of Theorem 2 in the main text.

Let  $\boldsymbol{\Omega}_1 = \widehat{\boldsymbol{\Omega}}^{-1/2} \boldsymbol{\Omega}^{1/2}$ ,  $\tilde{\boldsymbol{\Omega}}_1 = \boldsymbol{\Omega}_1 - [N^{-1} \text{tr}(\boldsymbol{\Omega}_1 \boldsymbol{\Omega}_1^\top)]^{-1/2} \mathbf{I}_N$ .

**Definition S.2** (*Stieltjes transform*) Let  $\mu_1(x)$  and  $\mu_{\boldsymbol{\Omega}_1^\top \boldsymbol{\Omega}_1}(x)$  be the limiting spectral distributions of  $T^{-1} \mathbf{Z}^\top \mathbf{Z}$  and  $T^{-1} \mathbf{Z}^\top \boldsymbol{\Omega}_1^\top \boldsymbol{\Omega}_1 \mathbf{Z}$ . For  $z \in \mathbb{C} \setminus \text{supp}(\mu_{\boldsymbol{\Omega}_1^\top \boldsymbol{\Omega}_1})$ ,

$$m_{\boldsymbol{\Omega}_1}(z) = \int_R \frac{1}{x - z} d\mu_{\boldsymbol{\Omega}_1^\top \boldsymbol{\Omega}_1}(x) \quad (\text{S.1.15})$$

is the Stieltjes transform of  $\mu_{\boldsymbol{\Omega}_1^\top \boldsymbol{\Omega}_1}(x)$ .

For  $z \in \mathbb{C} \setminus \text{supp}(\mu_1)$ ,

$$m_1(z) = \int_R \frac{1}{x - z} d\mu_1(x) \quad (\text{S.1.16})$$

is the Stieltjes transform of  $\mu_1(x)$ .

$$c_{\Omega_1}(\tau) = \frac{1}{1 - T^{-1}m_{\Omega_1}^2(-\tau)\text{tr}\{[\mathbf{I}_N + m_{\Omega_1}(-\tau)\Omega_2]^{-2}\Omega_2^2\}}$$

with  $\Omega_2 = \Omega_1\Omega_1^\top$ .

**Theorem S.4** *Suppose Assumptions 1 and 2 hold, and  $N, T \rightarrow \infty$ . If  $N/T \rightarrow \gamma \in (1, \infty)$ ,  $b = N^{-1}\text{tr}(\Omega_2)$ ,*

$$\mathbb{V}(\tilde{\omega}_\tau) = c_{\Omega_1}(\tau)[\mathbf{1}^\top \Sigma^{-1} \mathbf{1}]^{-1}[1 + O(\|(\Omega - b\hat{\Omega})\mathbf{P}_V^\perp\|) + o_p(1)]. \quad (\text{S.1.17})$$

If  $N/T \rightarrow \infty$ ,

$$\mathbb{V}(\tilde{\omega}_\tau) = [\mathbf{1}^\top \Sigma^{-1} \mathbf{1}]^{-1}[1 + O(\|(\Omega - b\hat{\Omega})\mathbf{P}_V^\perp\|) + o_p(1)]. \quad (\text{S.1.18})$$

(S.1.18) implies the results of (ii) in Theorem 2 in the main text. Moreover, when  $\|\Omega - \hat{\Omega}\| = o_p(1)$ ,

$$\begin{aligned} & \|\Omega - N^{-1}\text{tr}(\hat{\Omega}^{-1}\Omega)\hat{\Omega}\| \\ \leq & \|\Omega - \hat{\Omega}\| + \|\hat{\Omega} - N^{-1}\text{tr}(\hat{\Omega}^{-1}\Omega)\hat{\Omega}\| \\ \leq & \|\Omega - \hat{\Omega}\| + \|\hat{\Omega}\|[1 - N^{-1}\text{tr}(\hat{\Omega}^{-1}\Omega)] \\ = & \|\Omega - \hat{\Omega}\| + \|\hat{\Omega}\|N^{-1}\text{tr}[\hat{\Omega}^{-1}(\hat{\Omega} - \Omega)] \\ = & O(\|\Omega - \hat{\Omega}\|) = o_p(1). \end{aligned}$$

We prove the result of (iii) in Theorem 2.

We note that the above theorems can be extended to the non-Gaussian entries in  $\mathbf{Z}$  by random matrix theory. But it needs more complicated details. One can see [Knowles and Yin \(2017\)](#), [Ding and Yang \(2018\)](#) and [Yang \(2019\)](#).

## S.2 The outline of Proofs for Theorem S.1

We note that

$$\mathbb{V}(\hat{\omega}_\tau) = \frac{\mathbf{1}^\top \mathbf{S}_\tau^{-1} \Sigma \mathbf{S}_\tau^{-1} \mathbf{1}}{[\mathbf{1}^\top \mathbf{S}_\tau^{-1} \mathbf{1}]^2}. \quad (\text{S.2.1})$$

$$\mathbb{V}(\tilde{\omega}_\tau^{\text{ifs}}) = \frac{\mathbf{1}^\top \mathbf{S}_{\tau, \Omega}^{-1} \Sigma \mathbf{S}_{\tau, \Omega}^{-1} \mathbf{1}}{[\mathbf{1}^\top \mathbf{S}_{\tau, \Omega}^{-1} \mathbf{1}]^2}. \quad (\text{S.2.2})$$

$$\mathbb{V}(\tilde{\omega}_\tau) = \frac{\mathbf{1}^\top \mathbf{S}_{\tau, \hat{\Omega}}^{-1} \Sigma \mathbf{S}_{\tau, \hat{\Omega}}^{-1} \mathbf{1}}{[\mathbf{1}^\top \mathbf{S}_{\tau, \hat{\Omega}}^{-1} \mathbf{1}]^2}. \quad (\text{S.2.3})$$

When  $T > N$ ,

$$\mathbb{V}(\hat{\omega}) = \frac{\mathbf{1}^\top \mathbf{S}_0^{-1} \Sigma \mathbf{S}_0^{-1} \mathbf{1}}{[\mathbf{1}^\top \mathbf{S}_0^{-1} \mathbf{1}]^2}. \quad (\text{S.2.4})$$

We recall (S.2.1). Thus, we study the limit of  $\mathbf{1}^\top \mathbf{S}_\tau^{-1} \Sigma \mathbf{S}_\tau^{-1} \mathbf{1}$  and  $\mathbf{1}^\top \mathbf{S}_\tau^{-1} \mathbf{1}$ .

**Lemma S.1** *(The expansion of  $\mathbf{a}^\top \Sigma^{-1} \mathbf{a}$ )* For any  $N$  – dimensional unit vector  $\mathbf{a}$ ,

$$\mathbf{a}^\top \Sigma^{-1} \mathbf{a} = \mathbf{a}^\top \Omega^{-1/2} (\mathbf{I}_N - \mathbf{P}_{\Omega^{-1/2} \mathbf{V}}) \Omega^{-1/2} \mathbf{a} + O(N^{-\delta} \|\mathbf{V}^\top \Omega^{-1} \mathbf{a}\|^2). \quad (\text{S.2.5})$$

**Lemma S.2** *(Schur Complements)* When  $\mathbf{D}$  and  $\mathbf{A} - \mathbf{B}\mathbf{D}^{-1}\mathbf{C}$  is invertible,

$$\begin{pmatrix} \mathbf{A} & \mathbf{B} \\ \mathbf{C} & \mathbf{D} \end{pmatrix}^{-1} = \begin{pmatrix} (\mathbf{A} - \mathbf{B}\mathbf{D}^{-1}\mathbf{C})^{-1} & -(\mathbf{A} - \mathbf{B}\mathbf{D}^{-1}\mathbf{C})^{-1}\mathbf{B}\mathbf{D}^{-1} \\ -\mathbf{D}^{-1}\mathbf{C}(\mathbf{A} - \mathbf{B}\mathbf{D}^{-1}\mathbf{C})^{-1} & \mathbf{D}^{-1} + \mathbf{D}^{-1}\mathbf{C}(\mathbf{A} - \mathbf{B}\mathbf{D}^{-1}\mathbf{C})^{-1}\mathbf{B}\mathbf{D}^{-1} \end{pmatrix}. \quad (\text{S.2.6})$$

Thus, we have

$$\begin{aligned} & \begin{pmatrix} \tau \mathbf{I}_N & T^{-1/2} \mathbf{R} \\ T^{-1/2} \mathbf{R}^\top & -\mathbf{I}_T \end{pmatrix}^{-1} \\ = & \begin{pmatrix} (\tau \mathbf{I}_N + T^{-1} \mathbf{R} \mathbf{R}^\top)^{-1} & T^{-1/2} (\tau \mathbf{I}_N + T^{-1} \mathbf{R} \mathbf{R}^\top)^{-1} \mathbf{R} \\ T^{-1/2} \mathbf{R}^\top (\tau \mathbf{I}_N + T^{-1} \mathbf{R} \mathbf{R}^\top)^{-1} & -\mathbf{I}_T + T^{-1} \mathbf{R}^\top (\tau \mathbf{I}_N + T^{-1} \mathbf{R} \mathbf{R}^\top)^{-1} \mathbf{R} \end{pmatrix}. \end{aligned} \quad (\text{S.2.7})$$

Then for any unit vector  $\mathbf{a}$ , we can study  $\mathbf{a}^\top \mathbf{S}_\tau^{-1} \mathbf{a}$  by

$$(\mathbf{a}^\top, \mathbf{0}_{1 \times T}) \begin{pmatrix} \tau \mathbf{I}_N & T^{-1/2} \mathbf{R} \\ T^{-1/2} \mathbf{R}^\top & -\mathbf{I}_T \end{pmatrix}^{-1} \begin{pmatrix} \mathbf{a} \\ \mathbf{0}_{T \times 1} \end{pmatrix}. \quad (\text{S.2.8})$$

Recalling (S.1.1), we rewrite  $\mathbf{B}$  and  $\mathbf{F}$  as

$$\mathbf{B} = \mathbf{V} \mathbf{B}_1, \quad \mathbf{F} = \mathbf{F}_1 \mathbf{V}_1^\top,$$

where  $\mathbf{V}$  is a  $N \times r$  matrix and  $\mathbf{V}_1$  is a  $T \times r$  matrix satisfying  $\mathbf{V}^\top \mathbf{V} = \mathbf{V}_1^\top \mathbf{V}_1 = \mathbf{I}_r$

Now we define

$$\mathbf{G}_1(\tau) = \begin{pmatrix} \tau \mathbf{I}_N & T^{-1/2} \mathbf{E} \\ T^{-1/2} \mathbf{E}^\top & -\mathbf{I}_T \end{pmatrix}^{-1}, \quad (\text{S.2.9})$$

$$\mathbf{U}_1 = \begin{pmatrix} \mathbf{V} & \mathbf{0} \\ \mathbf{0} & \mathbf{V}_1 \end{pmatrix}, \quad \mathbf{P}_{U_1}^\perp = \mathbf{I}_{N+T} - \mathbf{U}_1 \mathbf{U}_1^\top \quad (\text{S.2.10})$$

$$\mathbf{D}_1 = \begin{pmatrix} \mathbf{0} & T^{-1/2} \mathbf{B}_1 \mathbf{F}_1 \\ T^{-1/2} \mathbf{F}_1^\top \mathbf{B}_1^\top & \mathbf{0} \end{pmatrix}. \quad (\text{S.2.11})$$

and

$$\mathbf{G}_2(\tau) = \begin{pmatrix} \tau \mathbf{I}_N & T^{-1/2} \mathbf{R} \\ T^{-1/2} \mathbf{R}^\top & -\mathbf{I}_T \end{pmatrix}^{-1} \quad (\text{S.2.12})$$

**Lemma S.3** (*The Woodbury matrix identity*) When  $\mathbf{A}$  and  $\mathbf{C}$  are invertible,

$$(\mathbf{A} + \mathbf{BCD})^{-1} = \mathbf{A}^{-1} - \mathbf{A}^{-1} \mathbf{B} (\mathbf{C}^{-1} + \mathbf{DA}^{-1} \mathbf{B})^{-1} \mathbf{DA}^{-1} \quad (\text{S.2.13})$$

We have

**Lemma S.4** (*The expansion of  $\mathbf{a}^\top \mathbf{S}_\tau^{-1} \mathbf{a}$* )

$$\mathbf{G}_2(\tau) = \mathbf{G}_1(\tau) - \mathbf{G}_1(\tau) \mathbf{U}_1 [\mathbf{D}_1^{-1} + \mathbf{U}_1^\top \mathbf{G}_1(\tau) \mathbf{U}_1]^{-1} \mathbf{U}_1^\top \mathbf{G}_1(\tau). \quad (\text{S.2.14})$$

$$\begin{aligned} \mathbf{a}^\top \mathbf{S}_\tau^{-1} \mathbf{a} &= (\mathbf{a}^\top, \mathbf{0}_{1 \times T}) \mathbf{G}_2(\tau) (\mathbf{a}^\top, \mathbf{0}_{1 \times T})^\top \\ &= (\mathbf{a}^\top, \mathbf{0}_{1 \times T}) \mathbf{P}_{U_1}^\perp \mathbf{G}_1(\tau) \mathbf{P}_{U_1}^\perp (\mathbf{a}^\top, \mathbf{0}_{1 \times T})^\top \\ &\quad - (\mathbf{a}^\top, \mathbf{0}_{1 \times T}) \mathbf{P}_{U_1}^\perp \mathbf{G}_1(\tau) \mathbf{U}_1 \left[ \mathbf{D}_1^{-1} + \mathbf{U}_1^\top \mathbf{G}_1(\tau) \mathbf{U}_1 \right]^{-1} \mathbf{U}_1^\top \mathbf{G}_1(\tau) \mathbf{P}_{U_1}^\perp (\mathbf{a}^\top, \mathbf{0}_{1 \times T})^\top \\ &\quad + 2(\mathbf{a}^\top, \mathbf{0}_{1 \times T}) \mathbf{U}_1 \mathbf{D}_1^{-1} [\mathbf{D}_1^{-1} + \mathbf{U}_1^\top \mathbf{G}_1(\tau) \mathbf{U}_1]^{-1} \mathbf{U}_1^\top \mathbf{G}_1(\tau) \mathbf{P}_{U_1}^\perp (\mathbf{a}^\top, \mathbf{0}_{1 \times T})^\top \\ &\quad - (\mathbf{a}^\top, \mathbf{0}_{1 \times n}) \mathbf{U}_1 \mathbf{D}_1^{-1} [\mathbf{D}_1^{-1} + \mathbf{U}_1^\top \mathbf{G}_1(\tau) \mathbf{U}_1]^{-1} \mathbf{D}_1^{-1} \mathbf{U}_1^\top (\mathbf{a}^\top, \mathbf{0}_{1 \times t})^\top. \end{aligned} \quad (\text{S.2.15})$$

Note that the dimensions of  $(\mathbf{a}^\top, \mathbf{0}_{1 \times T}) \mathbf{P}_{U_1}^\perp \mathbf{G}_1(\tau) \mathbf{U}_1$ ,  $\mathbf{D}_1^{-1} + \mathbf{U}_1^\top \mathbf{G}_1(\tau) \mathbf{U}_1$  and  $\mathbf{U}_1^\top \mathbf{G}_1(\tau) \mathbf{P}_{U_1}^\perp (\mathbf{a}^\top, \mathbf{0}_{1 \times T})^\top$  are  $2r$  which is finite.

If we obtain the limit of  $\mathbf{b}^\top \mathbf{G}_1(\tau) \mathbf{c}$  for any unit vector  $\mathbf{b}$  and  $\mathbf{c}$ , we can obtain the limit of (S.2.15).

For  $\mathbf{a}^\top \mathbf{S}_\tau^{-1} \Sigma \mathbf{S}_\tau^{-1} \mathbf{a}$ , we have

**Lemma S.5** (*The expansion of  $\mathbf{a}^\top \mathbf{S}_\tau^{-1} \Sigma \mathbf{S}_\tau^{-1} \mathbf{a}$* )

$$\begin{aligned} &\mathbf{a}^\top \mathbf{S}_\tau^{-1} \Sigma \mathbf{S}_\tau^{-1} \mathbf{a} \\ &= (\mathbf{a}^\top, \mathbf{0}_{1 \times T}) \mathbf{P}_{U_1}^\perp \mathbf{G}_2(\tau) \tilde{\Omega} \mathbf{G}_2(\tau) \mathbf{P}_{U_1}^\perp (\mathbf{a}^\top, \mathbf{0}_{1 \times T})^\top \\ &\quad + 2(\mathbf{a}^\top, \mathbf{0}_{1 \times T}) \mathbf{U}_1 \mathbf{D}_1^{-1} [\mathbf{D}_1^{-1} + \mathbf{U}_1^\top \mathbf{G}_1(\tau) \mathbf{U}_1]^{-1} \mathbf{U}_1^\top \mathbf{G}_1(\tau) \tilde{\Omega} \mathbf{G}_2(\tau) \mathbf{P}_{U_1}^\perp (\mathbf{a}^\top, \mathbf{0}_{1 \times T})^\top \\ &\quad + (\mathbf{a}^\top, \mathbf{0}_{1 \times T}) \mathbf{U}_1 \mathbf{D}_1^{-1} [\mathbf{D}_1^{-1} + \mathbf{U}_1^\top \mathbf{G}_1(\tau) \mathbf{U}_1]^{-1} \mathbf{U}_1^\top \mathbf{G}_1(\tau) \tilde{\Omega} \mathbf{G}_1(\tau) \mathbf{U}_1 [\mathbf{D}_1^{-1} + \mathbf{U}_1^\top \mathbf{G}_1(\tau) \mathbf{U}_1]^{-1} \\ &\quad \mathbf{D}_1^{-1} \mathbf{U}_1^\top (\mathbf{a}^\top, \mathbf{0}_{1 \times T})^\top + (\mathbf{a}^\top, \mathbf{0}_{1 \times T}) \mathbf{G}_2(\tau) \begin{pmatrix} \mathbf{B} \mathbf{B}^\top & \mathbf{0} \\ \mathbf{0}^\top & \mathbf{0} \end{pmatrix} \mathbf{G}_2(\tau) (\mathbf{a}^\top, \mathbf{0}_{1 \times T})^\top, \end{aligned} \quad (\text{S.2.16})$$

where

$$\tilde{\Omega} = \begin{pmatrix} \Omega & 0 \\ 0 & 0 \end{pmatrix}.$$

Note that the dimensions of  $(\mathbf{a}^\top, \mathbf{0}_{1 \times T}) \mathbf{P}_{U_1}^\perp \mathbf{G}_1(\tau) \tilde{\Omega} \mathbf{G}_1(\tau) \mathbf{U}_1$ ,  $\mathbf{U}_1^\top \mathbf{G}_1(\tau) \mathbf{P}_{U_1}^\perp (\mathbf{a}^\top, \mathbf{0}_{1 \times T})^\top$ ,  $\mathbf{D}_1^{-1} + \mathbf{U}_1^\top \mathbf{G}_1(\tau) \mathbf{U}_1$  and  $\mathbf{U}_1^\top \mathbf{G}_1(\tau) \tilde{\Omega} \mathbf{G}_1(\tau) \mathbf{U}_1$  are  $2r$  which is finite. We need to ob-

tain the limits of  $\mathbf{b}^\top \mathbf{G}_1(\tau) \tilde{\boldsymbol{\Omega}} \mathbf{G}_1(\tau) \mathbf{c}$  where  $\mathbf{b}$  and  $\mathbf{c}$  are any  $(T + N)$ -dimensional unit vectors with the first  $N$  entries or the last  $T$  entries being 0.

Thus, we focus on the limit of  $\mathbf{b}^\top \mathbf{G}_1(\tau) \mathbf{c}$  and  $\mathbf{b}^\top \mathbf{G}_1(\tau) \tilde{\boldsymbol{\Omega}} \mathbf{G}_1(\tau) \mathbf{c}$  for any unit vectors  $\mathbf{b}$  and  $\mathbf{c}$ .

**Lemma S.6** *For any unit unit vector  $\mathbf{a}$  and  $c > 0$ ,*

$$\|(\mathbf{I}_N - \mathbf{P}_{\boldsymbol{\Omega}^{-1/2}\mathbf{V}})\boldsymbol{\Omega}^{-1/2}\mathbf{a}\| \asymp \|\mathbf{P}_V^\perp \mathbf{a}\| \quad (\text{S.2.17})$$

and

$$\|(\mathbf{I}_N - \mathbf{P}_{[\mathbf{I}_N + c\boldsymbol{\Omega}]^{-1/2}\mathbf{V}})[\mathbf{I}_N + c\boldsymbol{\Omega}]^{-1/2}\mathbf{a}\| \asymp \|\mathbf{P}_V^\perp \mathbf{a}\|. \quad (\text{S.2.18})$$

Thus we define

$$\tilde{\mathbf{a}} = (\mathbf{I}_N - \mathbf{P}_{\boldsymbol{\Omega}^{-1/2}\mathbf{V}})\boldsymbol{\Omega}^{-1/2}\mathbf{a} \quad (\text{S.2.19})$$

$$\tilde{\mathbf{a}}_\tau = (\mathbf{I}_N - \mathbf{P}_{[\mathbf{I}_N + m(-\tau)\boldsymbol{\Omega}]^{-1/2}\mathbf{V}})[\mathbf{I}_N + m(-\tau)\boldsymbol{\Omega}]^{-1/2}\mathbf{a} \quad (\text{S.2.20})$$

for any unit vector  $\mathbf{a}$ . When we assume that  $\|\mathbf{P}_V^\perp \mathbf{a}\| \gg N^{(1-\delta)/2}T^{-1/2}$ ,  $\|\tilde{\mathbf{a}}\| \gg N^{(1-\delta)/2}T^{-1/2}$  and  $\|\tilde{\mathbf{a}}_\tau\| \gg N^{(1-\delta)/2}T^{-1/2}$ .

When  $\mathbf{a} = \mathbf{1}/\sqrt{N}$ ,  $N^{-1/2}\|\mathbf{P}_V^\perp \mathbf{1}\| \gg N^{(1-\delta)/2}T^{-1/2}$  in Assumption 2 implies that

$$\min\{\|\mathbf{P}_V^\perp \mathbf{a}\|, \|\tilde{\mathbf{a}}\|, \|\tilde{\mathbf{a}}_\tau\|\} \gg N^{(1-\delta)/2}T^{-1/2}. \quad (\text{S.2.21})$$

Thus, we assume that (S.2.21) holds in Section S.3-S.8.

### S.2.1 Proof of Lemma S.6

$$\mathbf{P}_{\boldsymbol{\Omega}^{-1/2}\mathbf{V}}^\perp \boldsymbol{\Omega}^{-1/2}\mathbf{V} = \mathbf{0}. \quad (\text{S.2.22})$$

The rank of  $(\mathbf{I}_N - \mathbf{P}_{\Omega^{-1/2}\mathbf{V}})\Omega^{-1/2}$  is  $N - r$ . Thus, we can rewrite it as

$$(\mathbf{I}_N - \mathbf{P}_{\Omega^{-1/2}\mathbf{V}})\Omega^{-1/2} = \mathbf{W}_1 \mathbf{\Lambda} \mathbf{W}_2^\top,$$

where  $\mathbf{W}_1$  and  $\mathbf{W}_2$  are  $N \times (N - r)$  orthogonal matrices and  $\mathbf{\Lambda}$  is a  $(N - r) \times (N - r)$  diagonal matrix with  $\|\mathbf{\Lambda}\| \asymp \|\mathbf{\Lambda}\| \asymp 1$ . On the other hand,

$$\mathbf{W}_1 \mathbf{\Lambda} \mathbf{W}_2^\top \mathbf{V} = (\mathbf{I}_N - \mathbf{P}_{\Omega^{-1/2}\mathbf{V}})\Omega^{-1/2}\mathbf{V} = \mathbf{0}.$$

Thus,  $\mathbf{W}_2^\top \mathbf{V} = \mathbf{0}_{(N-r) \times r}$  and  $\mathbf{W}_2^\top \mathbf{P}_V^\perp \mathbf{W}_2^\top = \mathbf{I}_{N-r}$ . Thus,

$$\begin{aligned} & \|(\mathbf{I}_N - \mathbf{P}_{\Omega^{-1/2}\mathbf{V}})\Omega^{-1/2}\mathbf{a}\| \\ &= \|(\mathbf{I}_N - \mathbf{P}_{\Omega^{-1/2}\mathbf{V}})\Omega^{-1/2}\mathbf{P}_V^\perp \mathbf{a}\| \\ &= \|\mathbf{W}_1 \mathbf{\Lambda} \mathbf{W}_2^\top \mathbf{P}_V^\perp \mathbf{a}\| \\ &\asymp \|\mathbf{W}_2^\top \mathbf{P}_V^\perp \mathbf{a}\| = \|\mathbf{P}_V^\perp \mathbf{a}\|. \end{aligned}$$

We prove (S.2.17).

Moreover,

$$(\mathbf{I}_N - \mathbf{P}_{[\mathbf{I}_N + c\Omega]^{-1/2}\mathbf{V}})[\mathbf{I}_N + c\Omega]^{-1/2}\mathbf{V} = \mathbf{0}.$$

We can prove (S.2.18) by the same discussion.

## S.2.2 Proof of Lemma S.1

From (S.1.1) and (S.2.13),

$$\begin{aligned} & \mathbf{a}^\top \Sigma^{-1} \mathbf{a} = \mathbf{a}^\top [\mathbf{V} \mathbf{B}_1 \mathbf{B}_1^\top \mathbf{V}^\top + \Omega]^{-1} \mathbf{a} \\ &= \mathbf{a}^\top \Omega^{-1} \mathbf{a} - \mathbf{a}^\top \Omega^{-1} \mathbf{V} [(\mathbf{B}_1 \mathbf{B}_1^\top)^{-1} + \mathbf{V}^\top \Omega^{-1} \mathbf{V}]^{-1} \mathbf{V}^\top \Omega^{-1} \mathbf{a} \\ &= \mathbf{a}^\top \Omega^{-1} \mathbf{a} - \mathbf{a}^\top \Omega^{-1} \mathbf{V} [\mathbf{V}^\top \Omega^{-1} \mathbf{V}]^{-1} \mathbf{V}^\top \Omega^{-1} \mathbf{a} + O(N^{-\delta} \|\mathbf{V}^\top \Omega^{-1} \mathbf{a}\|^2) \\ &= \mathbf{a}^\top \Omega^{-1/2} (\mathbf{I}_N - \mathbf{P}_{\Omega^{-1/2}\mathbf{V}}) \Omega^{-1/2} \mathbf{a} + O(N^{-\delta} \|\mathbf{V}^\top \Omega^{-1} \mathbf{a}\|^2). \end{aligned}$$

### S.2.3 Proof of Lemma S.4

From (S.1.1) and (S.2.9)-(S.2.12)

$$\begin{aligned} \mathbf{G}_2(\tau) &= \begin{pmatrix} \tau \mathbf{I}_N & T^{-1/2} \mathbf{R} \\ T^{-1/2} \mathbf{R}^\top & -\mathbf{I}_T \end{pmatrix}^{-1} \\ &= \left[ \begin{pmatrix} \tau \mathbf{I}_N & T^{-1/2} \mathbf{E} \\ T^{-1/2} \mathbf{E}^\top & -\mathbf{I}_T \end{pmatrix} + \begin{pmatrix} \mathbf{V} & \mathbf{0} \\ \mathbf{0} & \mathbf{V}_1 \end{pmatrix} \begin{pmatrix} \mathbf{0} & T^{-1/2} \mathbf{B}_1 \mathbf{F}_1 \\ T^{-1/2} \mathbf{F}_1^\top \mathbf{B}_1^\top & \mathbf{0} \end{pmatrix} \begin{pmatrix} \mathbf{V}^\top & \mathbf{0} \\ \mathbf{0} & \mathbf{V}_1^\top \end{pmatrix} \right]^{-1}. \end{aligned}$$

Since

$$\begin{pmatrix} \tau \mathbf{I}_N & T^{-1/2} \mathbf{E} \\ T^{-1/2} \mathbf{E}^\top & -\mathbf{I}_T \end{pmatrix}$$

and

$$\begin{pmatrix} \mathbf{0} & T^{-1/2} \mathbf{B}_1 \mathbf{F}_1 \\ T^{-1/2} \mathbf{F}_1^\top \mathbf{B}_1^\top & \mathbf{0} \end{pmatrix}$$

are invertible, (S.2.13) implies that

$$\begin{aligned} \mathbf{G}_2(\tau) &= \begin{pmatrix} \tau \mathbf{I}_N & T^{-1/2} \mathbf{R} \\ T^{-1/2} \mathbf{R}^\top & -\mathbf{I}_T \end{pmatrix}^{-1} \\ &= \left[ \begin{pmatrix} \tau \mathbf{I}_N & T^{-1/2} \mathbf{E} \\ T^{-1/2} \mathbf{E}^\top & -\mathbf{I}_T \end{pmatrix} + \begin{pmatrix} \mathbf{V} & \mathbf{0} \\ \mathbf{0} & \mathbf{V}_1 \end{pmatrix} \begin{pmatrix} \mathbf{0} & T^{-1/2} \mathbf{B}_1 \mathbf{F}_1 \\ T^{-1/2} \mathbf{F}_1^\top \mathbf{B}_1^\top & \mathbf{0} \end{pmatrix} \begin{pmatrix} \mathbf{V}^\top & \mathbf{0} \\ \mathbf{0} & \mathbf{V}_1^\top \end{pmatrix} \right]^{-1} \\ &= \begin{pmatrix} \tau \mathbf{I}_N & T^{-1/2} \mathbf{E} \\ T^{-1/2} \mathbf{E}^\top & -\mathbf{I}_T \end{pmatrix}^{-1} - \begin{pmatrix} \tau \mathbf{I}_N & T^{-1/2} \mathbf{E} \\ T^{-1/2} \mathbf{E}^\top & -\mathbf{I}_T \end{pmatrix}^{-1} \begin{pmatrix} \mathbf{V} & \mathbf{0} \\ \mathbf{0} & \mathbf{V}_1 \end{pmatrix} \\ &\quad \left[ \begin{pmatrix} \mathbf{0} & T^{-1/2} \mathbf{B}_1 \mathbf{F}_1 \\ T^{-1/2} \mathbf{F}_1^\top \mathbf{B}_1^\top & \mathbf{0} \end{pmatrix}^{-1} + \mathbf{U}_1^\top \begin{pmatrix} \tau \mathbf{I}_N & T^{-1/2} \mathbf{E} \\ T^{-1/2} \mathbf{E}^\top & -\mathbf{I}_T \end{pmatrix}^{-1} \mathbf{U}_1 \right]^{-1} \\ &\quad \begin{pmatrix} \mathbf{V}^\top & \mathbf{0} \\ \mathbf{0} & \mathbf{V}_1^\top \end{pmatrix} \begin{pmatrix} \tau \mathbf{I}_N & T^{-1/2} \mathbf{E} \\ T^{-1/2} \mathbf{E}^\top & -\mathbf{I}_T \end{pmatrix}^{-1} \\ &= \mathbf{G}_1(\tau) - \mathbf{G}_1(\tau) \mathbf{U}_1 [\mathbf{D}_1^{-1} + \mathbf{U}_1^\top \mathbf{G}_1(\tau) \mathbf{U}_1]^{-1} \mathbf{U}_1^\top \mathbf{G}_1(\tau). \end{aligned}$$

Thus, we prove (S.2.14).

Then, for any  $N$ -dimensional unit vector  $\mathbf{a}$ , (S.2.7) and (S.2.14) imply that

$$\begin{aligned}
& \mathbf{a}^\top \mathbf{S}_\tau^{-1} \mathbf{a} = (\mathbf{a}^\top, \mathbf{0}_{1 \times T}) \mathbf{G}_2(\tau) (\mathbf{a}^\top, \mathbf{0}_{1 \times T})^\top \\
= & \mathbf{a}^\top (\tau \mathbf{I}_N + T^{-1} \mathbf{E} \mathbf{E}^\top)^{-1} \mathbf{a} \\
& - (\mathbf{a}^\top, \mathbf{0}_{1 \times T}) \mathbf{G}_1(\tau) \mathbf{U}_1 [\mathbf{D}_1^{-1} + \mathbf{U}_1^\top \mathbf{G}_1(\tau) \mathbf{U}_1]^{-1} \mathbf{U}_1^\top \mathbf{G}_1(\tau) (\mathbf{a}^\top, \mathbf{0}_{1 \times T})^\top.
\end{aligned}$$

Recall definitions in (S.2.9)-(S.2.14),

$$\begin{aligned}
& \mathbf{U}_1 \mathbf{U}_1^\top \mathbf{G}_2(\tau) = \mathbf{U}_1 \mathbf{U}_1^\top \mathbf{G}_1(\tau) - \mathbf{U}_1 \mathbf{U}_1^\top \mathbf{G}_1(\tau) \mathbf{U}_1 [\mathbf{D}_1^{-1} + \mathbf{U}_1^\top \mathbf{G}_1(\tau) \mathbf{U}_1]^{-1} \mathbf{U}_1^\top \mathbf{G}_1(\tau) \\
= & \mathbf{U}_1 \mathbf{D}_1^{-1} [\mathbf{D}_1^{-1} + \mathbf{U}_1^\top \mathbf{G}_1(\tau) \mathbf{U}_1]^{-1} \mathbf{U}_1^\top \mathbf{G}_1(\tau).
\end{aligned}$$

$$(\mathbf{a}^\top, \mathbf{0}_{1 \times n}) \mathbf{U}_1 \mathbf{D}_1^{-1} \mathbf{U}_1^\top (\mathbf{a}^\top, \mathbf{0}_{1 \times t})^\top = 0.$$

$$\begin{aligned}
& (\mathbf{a}^\top, \mathbf{0}_{1 \times n}) \mathbf{U}_1 \mathbf{D}_1^{-1} [\mathbf{D}_1^{-1} + \mathbf{U}_1^\top \mathbf{G}_1(\tau) \mathbf{U}_1]^{-1} \mathbf{U}_1^\top \mathbf{G}_1(\tau) \mathbf{U}_1 \mathbf{U}_1^\top (\mathbf{a}^\top, \mathbf{0}_{1 \times t})^\top \\
= & (\mathbf{a}^\top, \mathbf{0}_{1 \times n}) \mathbf{U}_1 \mathbf{D}_1^{-1} \mathbf{U}_1^\top (\mathbf{a}^\top, \mathbf{0}_{1 \times t})^\top \\
& - (\mathbf{a}^\top, \mathbf{0}_{1 \times n}) \mathbf{U}_1 \mathbf{D}_1^{-1} [\mathbf{D}_1^{-1} + \mathbf{U}_1^\top \mathbf{G}_1(\tau) \mathbf{U}_1]^{-1} \mathbf{D}_1^{-1} \mathbf{U}_1^\top (\mathbf{a}^\top, \mathbf{0}_{1 \times t})^\top \\
= & - (\mathbf{a}^\top, \mathbf{0}_{1 \times n}) \mathbf{U}_1 \mathbf{D}_1^{-1} [\mathbf{D}_1^{-1} + \mathbf{U}_1^\top \mathbf{G}_1(\tau) \mathbf{U}_1]^{-1} \mathbf{D}_1^{-1} \mathbf{U}_1^\top (\mathbf{a}^\top, \mathbf{0}_{1 \times T})^\top.
\end{aligned}$$

$$\begin{aligned}
& \mathbf{a}^\top \mathbf{S}_\tau^{-1} \mathbf{a} = (\mathbf{a}^\top, \mathbf{0}_{1 \times T}) \mathbf{G}_2(\tau) (\mathbf{a}^\top, \mathbf{0}_{1 \times T})^\top \\
= & (\mathbf{a}^\top, \mathbf{0}_{1 \times T}) \mathbf{P}_{U_1}^\perp \mathbf{G}_2(\tau) \mathbf{P}_{U_1}^\perp (\mathbf{a}^\top, \mathbf{0}_{1 \times T})^\top \\
& + 2(\mathbf{a}^\top, \mathbf{0}_{1 \times T}) \mathbf{U}_1 \mathbf{U}_1^\top \mathbf{G}_2(\tau) \mathbf{P}_{U_1}^\perp (\mathbf{a}^\top, \mathbf{0}_{1 \times T})^\top \\
& + (\mathbf{a}^\top, \mathbf{0}_{1 \times T}) \mathbf{U}_1 \mathbf{U}_1^\top \mathbf{G}_2(\tau) \mathbf{U}_1 \mathbf{U}_1^\top (\mathbf{a}^\top, \mathbf{0}_{1 \times T})^\top \\
= & (\mathbf{a}^\top, \mathbf{0}_{1 \times T}) \mathbf{P}_{U_1}^\perp \mathbf{G}_2(\tau) \mathbf{P}_{U_1}^\perp (\mathbf{a}^\top, \mathbf{0}_{1 \times T})^\top \\
& + 2(\mathbf{a}^\top, \mathbf{0}_{1 \times T}) \mathbf{U}_1 \mathbf{D}_1^{-1} [\mathbf{D}_1^{-1} + \mathbf{U}_1^\top \mathbf{G}_1(\tau) \mathbf{U}_1]^{-1} \mathbf{U}_1^\top \mathbf{G}_1(\tau) \mathbf{P}_{U_1}^\perp (\mathbf{a}^\top, \mathbf{0}_{1 \times T})^\top \\
& + (\mathbf{a}^\top, \mathbf{0}_{1 \times T}) \mathbf{U}_1 \mathbf{D}_1^{-1} [\mathbf{D}_1^{-1} + \mathbf{U}_1^\top \mathbf{G}_1(\tau) \mathbf{U}_1]^{-1} \mathbf{U}_1^\top \mathbf{G}_1(\tau) \mathbf{U}_1 \mathbf{U}_1^\top (\mathbf{a}^\top, \mathbf{0}_{1 \times T})^\top \\
= & (\mathbf{a}^\top, \mathbf{0}_{1 \times T}) \mathbf{P}_{U_1}^\perp \mathbf{G}_1(\tau) \mathbf{P}_{U_1}^\perp (\mathbf{a}^\top, \mathbf{0}_{1 \times T})^\top \\
& - (\mathbf{a}^\top, \mathbf{0}_{1 \times T}) \mathbf{P}_{U_1}^\perp \mathbf{G}_1(\tau) \mathbf{U}_1 \left[ \mathbf{D}_1^{-1} + \mathbf{U}_1^\top \mathbf{G}_1(\tau) \mathbf{U}_1 \right]^{-1} \mathbf{U}_1^\top \mathbf{G}_1(\tau) \mathbf{P}_{U_1}^\perp (\mathbf{a}^\top, \mathbf{0}_{1 \times T})^\top \\
& + 2(\mathbf{a}^\top, \mathbf{0}_{1 \times T}) \mathbf{U}_1 \mathbf{D}_1^{-1} [\mathbf{D}_1^{-1} + \mathbf{U}_1^\top \mathbf{G}_1(\tau) \mathbf{U}_1]^{-1} \mathbf{U}_1^\top \mathbf{G}_1(\tau) \mathbf{P}_{U_1}^\perp (\mathbf{a}^\top, \mathbf{0}_{1 \times T})^\top \\
& - (\mathbf{a}^\top, \mathbf{0}_{1 \times n}) \mathbf{U}_1 \mathbf{D}_1^{-1} [\mathbf{D}_1^{-1} + \mathbf{U}_1^\top \mathbf{G}_1(\tau) \mathbf{U}_1]^{-1} \mathbf{D}_1^{-1} \mathbf{U}_1^\top (\mathbf{a}^\top, \mathbf{0}_{1 \times T})^\top.
\end{aligned}$$

#### S.2.4 Proof of Lemma S.5

$$\begin{aligned}
& \mathbf{a}^\top \mathbf{S}_\tau^{-1} \Sigma \mathbf{S}_\tau^{-1} \mathbf{a} \\
= & (\mathbf{a}^\top, \mathbf{0}_{1 \times T}) \begin{pmatrix} \tau \mathbf{I}_N & T^{-1/2} \mathbf{R} \\ T^{-1/2} \mathbf{R}^\top & -\mathbf{I}_T \end{pmatrix}^{-1} \begin{pmatrix} \Sigma & \mathbf{0} \\ \mathbf{0} & \mathbf{0} \end{pmatrix} \begin{pmatrix} \tau \mathbf{I}_N & T^{-1/2} \mathbf{R} \\ T^{-1/2} \mathbf{R}^\top & -\mathbf{I}_T \end{pmatrix}^{-1} (\mathbf{a}^\top, \mathbf{0}_{1 \times T})^\top \\
= & (\mathbf{a}^\top, \mathbf{0}_{1 \times T}) \mathbf{G}_2(\tau) \tilde{\Omega}_0 \mathbf{G}_2(\tau) (\mathbf{a}^\top, \mathbf{0}_{1 \times T})^\top.
\end{aligned}$$

Rewrite  $\tilde{\Omega}_0$  as

$$\tilde{\Omega}_0 = \begin{pmatrix} \mathbf{B} \mathbf{B}^\top & \mathbf{0} \\ \mathbf{0}^\top & \mathbf{0} \end{pmatrix} + \begin{pmatrix} \Omega & \mathbf{0} \\ \mathbf{0} & \mathbf{0} \end{pmatrix} = \begin{pmatrix} \mathbf{B} \mathbf{B}^\top & \mathbf{0} \\ \mathbf{0}^\top & \mathbf{0} \end{pmatrix} + \tilde{\Omega}.$$

$$\begin{aligned}
& \left\{ \mathbf{G}_1(\tau) - \mathbf{G}_1(\tau) \mathbf{U}_1 [\mathbf{D}_1^{-1} + \mathbf{U}_1^\top \mathbf{G}_1(\tau) \mathbf{U}_1]^{-1} \mathbf{U}_1^\top \mathbf{G}_1(\tau) \right\} \mathbf{U}_1 \\
= & \mathbf{G}_1(\tau) \mathbf{U}_1 [\mathbf{D}_1^{-1} + \mathbf{U}_1^\top \mathbf{G}_1(\tau) \mathbf{U}_1]^{-1} [\mathbf{D}_1^{-1} + \mathbf{U}_1^\top \mathbf{G}_1(\tau) \mathbf{U}_1] \\
& - \mathbf{G}_1(\tau) \mathbf{U}_1 [\mathbf{D}_1^{-1} + \mathbf{U}_1^\top \mathbf{G}_1(\tau) \mathbf{U}_1]^{-1} \mathbf{U}_1^\top \mathbf{G}_1(\tau) \mathbf{U}_1 \\
= & \mathbf{G}_1(\tau) \mathbf{U}_1 [\mathbf{D}_1^{-1} + \mathbf{U}_1^\top \mathbf{G}_1(\tau) \mathbf{U}_1]^{-1} \mathbf{D}_1^{-1}.
\end{aligned}$$

$$\mathbf{a}^\top \mathbf{S}_\tau^{-1} \Sigma \mathbf{S}_\tau^{-1} \mathbf{a} = (\mathbf{a}^\top, \mathbf{0}_{1 \times T}) \mathbf{G}_2(\tau) \tilde{\Omega}_0 \mathbf{G}_2(\tau) (\mathbf{a}^\top, \mathbf{0}_{1 \times T})^\top \quad (\text{S.2.23})$$

$$\begin{aligned} &= (\mathbf{a}^\top, \mathbf{0}_{1 \times T}) \mathbf{G}_2(\tau) \begin{pmatrix} \mathbf{B}\mathbf{B}^\top & \mathbf{0} \\ \mathbf{0}^\top & \mathbf{0} \end{pmatrix} \mathbf{G}_2(\tau) (\mathbf{a}^\top, \mathbf{0}_{1 \times T})^\top \\ &\quad + (\mathbf{a}^\top, \mathbf{0}_{1 \times T}) \mathbf{G}_2(\tau) \tilde{\Omega} \mathbf{G}_2(\tau) (\mathbf{a}^\top, \mathbf{0}_{1 \times T})^\top. \end{aligned} \quad (\text{S.2.24})$$

(S.2.14) implies that

$$\begin{aligned} \mathbf{U}_1^\top \mathbf{G}_2(\tau) &= \mathbf{U}_1^\top \mathbf{G}_1(\tau) - \mathbf{U}_1^\top \mathbf{G}_1(\tau) \mathbf{U}_1 [\mathbf{D}_1^{-1} + \mathbf{U}_1^\top \mathbf{G}_1(\tau) \mathbf{U}_1]^{-1} \mathbf{U}_1^\top \mathbf{G}_1(\tau) \\ &= \mathbf{D}_1^{-1} [\mathbf{D}_1^{-1} + \mathbf{U}_1^\top \mathbf{G}_1(\tau) \mathbf{U}_1]^{-1} \mathbf{U}_1^\top \mathbf{G}_1(\tau) \end{aligned} \quad (\text{S.2.25})$$

$$\begin{aligned} &(\mathbf{a}^\top, \mathbf{0}_{1 \times T}) \mathbf{G}_2(\tau) \tilde{\Omega} \mathbf{G}_2(\tau) (\mathbf{a}^\top, \mathbf{0}_{1 \times T})^\top \\ &= (\mathbf{a}^\top, \mathbf{0}_{1 \times T}) \mathbf{P}_{U_1}^\perp \mathbf{G}_2(\tau) \tilde{\Omega} \mathbf{G}_2(\tau) \mathbf{P}_{U_1}^\perp (\mathbf{a}^\top, \mathbf{0}_{1 \times T})^\top \\ &\quad + 2(\mathbf{a}^\top, \mathbf{0}_{1 \times T}) \mathbf{U}_1 \mathbf{U}_1^\top \mathbf{G}_2(\tau) \tilde{\Omega} \mathbf{G}_2(\tau) \mathbf{P}_{U_1}^\perp (\mathbf{a}^\top, \mathbf{0}_{1 \times T})^\top \\ &\quad + (\mathbf{a}^\top, \mathbf{0}_{1 \times T}) \mathbf{U}_1 \mathbf{U}_1^\top \mathbf{G}_2(\tau) \tilde{\Omega} \mathbf{G}_2(\tau) \mathbf{U}_1 \mathbf{U}_1^\top (\mathbf{a}^\top, \mathbf{0}_{1 \times T})^\top \\ &= (\mathbf{a}^\top, \mathbf{0}_{1 \times T}) \mathbf{P}_{U_1}^\perp \mathbf{G}_2(\tau) \tilde{\Omega} \mathbf{G}_2(\tau) \mathbf{P}_{U_1}^\perp (\mathbf{a}^\top, \mathbf{0}_{1 \times T})^\top \\ &\quad + 2(\mathbf{a}^\top, \mathbf{0}_{1 \times T}) \mathbf{U}_1 \mathbf{D}_1^{-1} [\mathbf{D}_1^{-1} + \mathbf{U}_1^\top \mathbf{G}_1(\tau) \mathbf{U}_1]^{-1} \mathbf{U}_1^\top \mathbf{G}_1(\tau) \tilde{\Omega} \mathbf{G}_2(\tau) \mathbf{P}_{U_1}^\perp (\mathbf{a}^\top, \mathbf{0}_{1 \times T})^\top \\ &\quad + (\mathbf{a}^\top, \mathbf{0}_{1 \times T}) \mathbf{U}_1 \mathbf{D}_1^{-1} [\mathbf{D}_1^{-1} + \mathbf{U}_1^\top \mathbf{G}_1(\tau) \mathbf{U}_1]^{-1} \mathbf{U}_1^\top \mathbf{G}_1(\tau) \tilde{\Omega} \mathbf{G}_1(\tau) \mathbf{U}_1 \\ &\quad [\mathbf{D}_1^{-1} + \mathbf{U}_1^\top \mathbf{G}_1(\tau) \mathbf{U}_1]^{-1} \mathbf{D}_1^{-1} \mathbf{U}_1^\top (\mathbf{a}^\top, \mathbf{0}_{1 \times T})^\top \end{aligned}$$

This, together with (S.2.23), completes the proof.

### S.3 The limit of $\mathbf{a}^\top \mathbf{S}_\tau^{-1} \mathbf{a}$

Since  $\mathbf{E} = \Omega^{1/2} \mathbf{Z}$ , for a set  $S \subset \{1, 2, \dots, n+p\} = S_0$ , we define  $\mathbf{G}^{(S)}$  as

$$\left\{ \left[ \begin{pmatrix} \tau \Omega^{-1} & T^{-1/2} \mathbf{Z} \\ T^{-1/2} \mathbf{Z}^\top & -\mathbf{I}_T \end{pmatrix} \right]_{s,t \in S_0 \setminus S} \right\}^{-1}. \quad (\text{S.3.1})$$

Then we define

$$\mathbf{H}^{-1} = \mathbf{G}^{(\emptyset)} = \begin{pmatrix} \boldsymbol{\Omega}^{1/2} & \mathbf{0} \\ \mathbf{0} & \mathbf{I}_T \end{pmatrix} \mathbf{G}_1(\tau) \begin{pmatrix} \boldsymbol{\Omega}^{1/2} & \mathbf{0} \\ \mathbf{0} & \mathbf{I}_T \end{pmatrix}.$$

Let  $G_{st}$  be the  $(s, t)$ th entry of  $\mathbf{G}^{(\emptyset)}$ .

$$\begin{aligned} & \mathbf{G}^{(\emptyset)} \tag{S.3.2} \\ = & \begin{pmatrix} (\tau \boldsymbol{\Omega}^{-1} + T^{-1} \mathbf{Z} \mathbf{Z}^\top)^{-1} & T^{-1/2} (\tau \boldsymbol{\Omega}^{-1} + T^{-1} \mathbf{Z} \mathbf{Z}^\top)^{-1} \mathbf{Z} \\ T^{-1/2} \mathbf{Z}^\top (\tau \boldsymbol{\Omega}^{-1} + T^{-1} \mathbf{Z} \mathbf{Z}^\top)^{-1} & -\mathbf{I}_T + T^{-1} \mathbf{Z}^\top (\tau \boldsymbol{\Omega}^{-1} + T^{-1} \mathbf{Z} \mathbf{Z}^\top)^{-1} \mathbf{Z} \end{pmatrix}. \end{aligned}$$

The Schur complement also implies that

$$\begin{aligned} & \mathbf{G}^{(\emptyset)} \tag{S.3.3} \\ = & \begin{pmatrix} (\tau \boldsymbol{\Omega}^{-1} + T^{-1} \mathbf{Z} \mathbf{Z}^\top)^{-1} & T^{-1/2} (\tau \boldsymbol{\Omega}^{-1} + T^{-1} \mathbf{Z} \mathbf{Z}^\top)^{-1} \mathbf{Z} \\ T^{-1/2} \tau^{-1} (\mathbf{I}_T + T^{-1} \tau^{-1} \mathbf{Z}^\top \boldsymbol{\Omega} \mathbf{Z})^{-1} \mathbf{Z}^\top \boldsymbol{\Omega} & -(\mathbf{I}_T + T^{-1} \tau^{-1} \mathbf{Z}^\top \boldsymbol{\Omega} \mathbf{Z})^{-1} \end{pmatrix}. \end{aligned}$$

### S.3.1 The asymptotic results for elements of $\mathbf{G}^{(\emptyset)}$ when $N \asymp T$

**Definition S.3** We can define the following matrix

$$\begin{aligned} & \mathbf{Q}(\tau) \tag{S.3.4} \\ = & \begin{pmatrix} \tau^{1/2} \mathbf{I}_N & \mathbf{0} \\ \mathbf{0} & \tau^{-1/2} \mathbf{I}_T \end{pmatrix} \mathbf{G}^{(\emptyset)} \begin{pmatrix} \tau^{1/2} \mathbf{I}_N & \mathbf{0} \\ \mathbf{0} & \tau^{-1/2} \mathbf{I}_T \end{pmatrix} - \begin{pmatrix} [\mathbf{I}_N + m(-\tau) \boldsymbol{\Omega}]^{-1} \boldsymbol{\Omega} & \mathbf{0} \\ \mathbf{0} & -m(-\tau) \mathbf{I}_T \end{pmatrix}. \end{aligned}$$

**Lemma S.7** Assume that  $z_{ij}$  follows the standard normal distribution, for any  $(N + T) \times (N + T)$  orthogonal matrix  $\mathbf{U}_2$ ,

$$[\mathbf{U}_2 \mathbf{Q}(\tau) \mathbf{U}_2^\top]_{st} = O_p(T^{-1/2}). \tag{S.3.5}$$

### S.3.2 Proofs of Lemma S.7

**Lemma S.8** (A weak result) When  $\tau > 0$ ,  $[\mathbf{Q}(\tau)]_{st} = O_p(T^{-1/2})$  for any  $1 \leq s, t \leq T + N$ .

**Proof.**

Since  $z_{ij}$  follows the standard normal distribution, Without loss of generality, we can assume that  $\mathbf{\Omega} = \text{diag}(\theta_1, \dots, \theta_N)$  is a diagonal matrix.

Now we give an important lemma in random matrix theory.

**Lemma S.9** (*Resolvent identities*) Let  $h_{ij}$  be the  $(i, j)$ th entry of  $\mathbf{H}$ . If  $i, j, k \in S_0 \setminus S$  and  $i, j \neq k$ , then

$$G_{ij}^{(S)} = G_{ij}^{(Sk)} + \frac{G_{ik}^{(S)} G_{kj}^{(S)}}{G_{kk}^{(S)}}$$

and

$$\frac{1}{G_{ii}^{(S)}} = \frac{1}{G_{ii}^{(Sk)}} - \frac{G_{ik}^{(S)} G_{ki}^{(S)}}{G_{ii}^{(S)} G_{ii}^{(Sk)} G_{kk}^{(S)}}.$$

Moreover, if  $i \neq j$ ,

$$G_{ij}^{(S)} = -G_{ii}^{(S)} \sum_{k \in S_0 \setminus S \cup \{i\}} h_{ik} G_{kj}^{(Si)} = -G_{jj}^{(S)} \sum_{k \in S_0 \setminus S \cup \{j\}} G_{ik}^{(Si)} h_{kj},$$

for

Let  $\mathbf{z}_i$  be the  $i$ th row of  $\mathbf{Z}$  and  $\tilde{\mathbf{z}}_i^\top = (\mathbf{0}_{1 \times (N-1)}, \mathbf{z}_i^\top)$ . From the Schur Complements, we have that for  $1 \leq s \leq N$ ,

$$\frac{1}{G_{ss}} = \tau \theta_s^{-1} - T^{-1} \tilde{\mathbf{z}}_s^\top \mathbf{G}^{(s)} \tilde{\mathbf{z}}_s. \quad (\text{S.3.6})$$

Let  $\check{\mathbf{z}}_i^\top$  be the  $i$ th column of  $\mathbf{Z}$  and  $\check{\mathbf{z}}_i^\top = (\check{\mathbf{z}}_i^\top, \mathbf{0}_{1 \times (T-1)})$ . For  $N+1 \leq s \leq N+T$ ,

$$\frac{1}{G_{ss}} = -1 - T^{-1} \check{\mathbf{z}}_s^\top \mathbf{G}^{(s)} \check{\mathbf{z}}_s. \quad (\text{S.3.7})$$

Lemma S.9 implies that, for  $1 \leq s \neq t \leq N$ ,

$$G_{st} = -G_{ss} \sum_{k \neq s} h_{sk} G_{kt}^{(s)} = -T^{-1/2} G_{ss} (\tilde{\mathbf{z}}_s^\top \mathbf{G}^{(s)})_t, \quad (\text{S.3.8})$$

for  $N + 1 \leq s \neq t \leq T + N$ ,

$$G_{st} = -G_{ss} \sum_{k \neq s} h_{sk} G_{kt}^{(s)} = -T^{-1/2} G_{ss} (\tilde{\mathbf{z}}_{s-p}^\top \mathbf{G}^{(s)})_t, \quad (\text{S.3.9})$$

for  $1 \leq s \leq N < t < T + N$ ,

$$\begin{aligned} G_{st} &= -G_{ss} \sum_{k \neq s} h_{sk} \mathbf{G}_{kt}^{(s)} = -T^{-1/2} G_{ss} (\tilde{\mathbf{z}}_s^\top \mathbf{G}^{(s)})_t \\ &= -T^{-1/2} G_{ss} \sum_{k=N+1}^{T+N} z_{k-N,s} G_{kt}^{(s)} \\ &= G_{ss} G_{tt}^{(s)} [-T^{-1/2} z_{t-N,s} + T^{-1} (\tilde{\mathbf{z}}_s^{(t)})^\top \mathbf{G}^{(st)} \tilde{\mathbf{z}}_{t-N}^{(s)}] \end{aligned} \quad (\text{S.3.10})$$

Here we delete the  $t$ th element of  $\tilde{\mathbf{z}}_s^\top$  to get  $(\tilde{\mathbf{z}}_s^{(t)})^\top$ .

Note that  $\tilde{\mathbf{z}}_s$  is independent of  $\mathbf{G}^{(s)}$ , (S.3.6) implies that for  $1 \leq s \leq N$ ,

$$\frac{1}{G_{ss}} = \tau \theta_s^{-1} - T^{-1} \sum_{i=N}^{T+N-1} G_{ii}^{(s)} + O_p(T^{-1} \{ \sum_{i,j=N}^{T+N-1} [G_{ij}^{(s)}]^2 \}^{1/2}). \quad (\text{S.3.11})$$

(S.3.3) implies that  $\sum_{i,j=N}^{T+N-1} [G_{ij}^{(s)}]^2 = O_p(\tau^2 T)$ . Moreover, (S.3.3) implies that

$$\begin{aligned} \sum_{i=N}^{T+N-1} G_{ii}^{(s)} &= -\text{tr}[(\mathbf{I}_T + T^{-1} \tau^{-1} \mathbf{Z} \mathbf{\Omega} \mathbf{Z}^\top)^{-1}] + O_p(1) \\ &= -\tau \text{tr}[(\tau \mathbf{I}_T + T^{-1} \mathbf{Z} \mathbf{\Omega} \mathbf{Z}^\top)^{-1}] + O_p(1) = -\tau T m(-\tau) + O_p(1). \end{aligned}$$

Then for  $1 \leq s \leq N$ ,

$$\frac{1}{G_{ss}} = \tau [\theta_s^{-1} + m(-\tau)] + O_p(\tau T^{-1/2}) = \tau \frac{1 + \theta_s m(-\tau)}{\theta_s} [1 + O_p(T^{-1/2})]. \quad (\text{S.3.12})$$

Similarly, for  $N + 1 \leq s \leq T + N$ ,

$$\begin{aligned}
\frac{1}{G_{ss}} &= -1 - T^{-1} \mathbf{z}_s^\top \mathbf{G}^{(s)} \mathbf{z}_s \\
&= -1 - T^{-1} \sum_{i=1}^N G_{ii}^{(s)} + O_p(\tau^{-1} T^{-1/2}) \\
&= -1 - T^{-1} \sum_{i=1}^N G_{ii} + O_p(\tau^{-1} T^{-1/2}) \\
&= -1 - T^{-1} \tau^{-1} \sum_{i=1}^N [\theta_s^{-1} + m(-\tau)]^{-1} + O_p(\tau^{-1} T^{-1/2}) \\
&= -1 - T^{-1} \tau^{-1} \sum_{i=1}^N \frac{\theta_s}{1 + \theta_s m(-\tau)} + O_p(\tau^{-1} T^{-1/2}) \\
&= -1 - \tau^{-1} \left[ \frac{1}{m(-\tau)} - \tau \right] + O_p(\tau^{-1} T^{-1/2}) \\
&= -\tau^{-1} \frac{1}{m(-\tau)} [1 + O_p(T^{-1/2})] \tag{S.3.13}
\end{aligned}$$

Thus, for  $1 \leq s \leq T + N$ ,  $G_{ss} = O_p(1)$ . (S.3.10) implies that  $G_{st} = O_p(T^{-1/2})$  for  $1 \leq s \leq N < t < T + N$ . Other off-diagonal elements can be controlled by the same method as (S.3.10).

Based on Lemma S.8, we can follow section 6 in Knowles and Yin (2017) to prove for any  $(T + N) \times (T + N)$  orthogonal matrix  $U_2$ , (S.3.5) holds.

### S.3.3 The limit of $\mathbf{a}^\top \mathbf{S}_\tau^{-1} \mathbf{a}$ when $N/T \rightarrow \gamma \in (1, \infty)$

Recalling (S.2.15),

$$\begin{aligned}
\mathbf{a}^\top \mathbf{S}_\tau^{-1} \mathbf{a} &= (\mathbf{a}^\top, \mathbf{0}_{1 \times T}) \mathbf{G}_2(\tau) (\mathbf{a}^\top, \mathbf{0}_{1 \times T})^\top \\
&= (\mathbf{a}^\top, \mathbf{0}_{1 \times T}) \mathbf{P}_{U_1}^\perp \mathbf{G}_1(\tau) \mathbf{P}_{U_1}^\perp (\mathbf{a}^\top, \mathbf{0}_{1 \times T})^\top \\
&\quad - (\mathbf{a}^\top, \mathbf{0}_{1 \times T}) \mathbf{P}_{U_1}^\perp \mathbf{G}_1(\tau) \mathbf{U}_1 \left[ \mathbf{D}_1^{-1} + \mathbf{U}_1^\top \mathbf{G}_1(\tau) \mathbf{U}_1 \right]^{-1} \mathbf{U}_1^\top \mathbf{G}_1(\tau) \mathbf{P}_{U_1}^\perp (\mathbf{a}^\top, \mathbf{0}_{1 \times T})^\top \\
&\quad + 2(\mathbf{a}^\top, \mathbf{0}_{1 \times T}) \mathbf{U}_1 \mathbf{D}_1^{-1} [\mathbf{D}_1^{-1} + \mathbf{U}_1^\top \mathbf{G}_1(\tau) \mathbf{U}_1]^{-1} \mathbf{U}_1^\top \mathbf{G}_1(\tau) \mathbf{P}_{U_1}^\perp (\mathbf{a}^\top, \mathbf{0}_{1 \times T})^\top \\
&\quad - (\mathbf{a}^\top, \mathbf{0}_{1 \times T}) \mathbf{U}_1 \mathbf{D}_1^{-1} [\mathbf{D}_1^{-1} + \mathbf{U}_1^\top \mathbf{G}_1(\tau) \mathbf{U}_1]^{-1} \mathbf{D}_1^{-1} \mathbf{U}_1^\top (\mathbf{a}^\top, \mathbf{0}_{1 \times T})^\top.
\end{aligned}$$

From (S.3.5),

$$\begin{aligned} & (\mathbf{a}^\top, \mathbf{0}_{1 \times T}) \mathbf{P}_{U_1}^\perp \mathbf{G}_1(\tau) \mathbf{P}_{U_1}^\perp (\mathbf{a}^\top, \mathbf{0}_{1 \times T})^\top \\ &= \tau^{-1} \mathbf{a}^\top \mathbf{P}_V^\perp [\mathbf{I}_N + m(-\tau) \boldsymbol{\Omega}]^{-1} \mathbf{P}_V^\perp \mathbf{a} [1 + o_p(1)]. \end{aligned}$$

Note that

$$\begin{aligned} & \mathbf{U}_1^\top \mathbf{G}_1(\tau) \mathbf{U}_1 \\ &= \begin{pmatrix} \mathbf{V}^\top & \mathbf{0} \\ \mathbf{0} & \mathbf{V}_1^\top \end{pmatrix} \begin{pmatrix} \boldsymbol{\Omega}^{-1/2} & \mathbf{0} \\ \mathbf{0} & \mathbf{I}_T \end{pmatrix} \mathbf{G}^{(\emptyset)} \begin{pmatrix} \boldsymbol{\Omega}^{-1/2} & \mathbf{0} \\ \mathbf{0} & \mathbf{I}_T \end{pmatrix} \begin{pmatrix} \mathbf{V}^\top & \mathbf{0} \\ \mathbf{0} & \mathbf{V}_1^\top \end{pmatrix} \\ &= \begin{pmatrix} \tau^{-1/2} \mathbf{V}^\top \boldsymbol{\Omega}^{-1/2} & \mathbf{0} \\ \mathbf{0} & \tau^{1/2} \mathbf{V}_1^\top \end{pmatrix} \begin{pmatrix} \tau^{1/2} \mathbf{I}_N & \mathbf{0} \\ \mathbf{0} & \tau^{-1/2} \mathbf{I}_T \end{pmatrix} \mathbf{G}^{(\emptyset)} \\ & \quad \begin{pmatrix} \tau^{1/2} \mathbf{I}_N & \mathbf{0} \\ \mathbf{0} & \tau^{-1/2} \mathbf{I}_T \end{pmatrix} \begin{pmatrix} \tau^{-1/2} \boldsymbol{\Omega}^{-1/2} \mathbf{V}^\top & \mathbf{0} \\ \mathbf{0} & \tau^{1/2} \mathbf{V}_1^\top \end{pmatrix} \\ &= \begin{pmatrix} \tau^{-1/2} \mathbf{V}^\top \boldsymbol{\Omega}^{-1/2} & \mathbf{0} \\ \mathbf{0} & \tau^{1/2} \mathbf{V}_1^\top \end{pmatrix} \left\{ \begin{pmatrix} [\mathbf{I}_N + m(-\tau) \boldsymbol{\Omega}]^{-1} \boldsymbol{\Omega} & \mathbf{0} \\ \mathbf{0} & -m(-\tau) \mathbf{I}_T \end{pmatrix} + \mathbf{Q}(\tau) \right\} \\ & \quad \begin{pmatrix} \tau^{-1/2} \boldsymbol{\Omega}^{-1/2} \mathbf{V}^\top & \mathbf{0} \\ \mathbf{0} & \tau^{1/2} \mathbf{V}_1^\top \end{pmatrix} \\ &= \begin{pmatrix} \tau^{-1/2} \mathbf{I}_r & \mathbf{0} \\ \mathbf{0} & \tau^{1/2} \mathbf{I}_r \end{pmatrix} \begin{pmatrix} \mathbf{V}^\top [\mathbf{I}_N + m(-\tau) \boldsymbol{\Omega}]^{-1} \mathbf{V} & \mathbf{0} \\ \mathbf{0} & -m(-\tau) \mathbf{I}_r \end{pmatrix} \begin{pmatrix} \tau^{-1/2} \mathbf{I}_r & \mathbf{0} \\ \mathbf{0} & \tau^{1/2} \mathbf{I}_r \end{pmatrix} \\ &+ \begin{pmatrix} \tau^{-1/2} \mathbf{V}^\top \boldsymbol{\Omega}^{-1/2} & \mathbf{0} \\ \mathbf{0} & \tau^{1/2} \mathbf{V}_1^\top \end{pmatrix} \mathbf{Q}(\tau) \begin{pmatrix} \tau^{-1/2} \boldsymbol{\Omega}^{-1/2} \mathbf{V}^\top & \mathbf{0} \\ \mathbf{0} & \tau^{1/2} \mathbf{V}_1^\top \end{pmatrix}. \end{aligned}$$

Moreover, recall (S.2.11), non-zero elements of  $\mathbf{D}_1$  and  $\mathbf{D}_1^{-1}$  are in the off-diagonal blocks.

$$\begin{aligned} & \mathbf{D}_1^{-1} + \begin{pmatrix} \tau^{-1/2} \mathbf{I}_r & \mathbf{0} \\ \mathbf{0} & \tau^{1/2} \mathbf{I}_r \end{pmatrix} \begin{pmatrix} \mathbf{V}^\top [\mathbf{I}_N + m(-\tau) \boldsymbol{\Omega}]^{-1} \mathbf{V} & \mathbf{0} \\ \mathbf{0} & -m(-\tau) \mathbf{I}_r \end{pmatrix} \begin{pmatrix} \tau^{-1/2} \mathbf{I}_r & \mathbf{0} \\ \mathbf{0} & \tau^{1/2} \mathbf{I}_r \end{pmatrix} \\ &= \begin{pmatrix} \tau^{-1/2} \mathbf{I}_r & \mathbf{0} \\ \mathbf{0} & \tau^{1/2} \mathbf{I}_r \end{pmatrix} \left\{ \mathbf{D}_1^{-1} + \begin{pmatrix} \mathbf{V}^\top [\mathbf{I}_N + m(-\tau) \boldsymbol{\Omega}]^{-1} \mathbf{V} & \mathbf{0} \\ \mathbf{0} & -m(-\tau) \mathbf{I}_r \end{pmatrix} \right\} \begin{pmatrix} \tau^{-1/2} \mathbf{I}_r & \mathbf{0} \\ \mathbf{0} & \tau^{1/2} \mathbf{I}_r \end{pmatrix}. \end{aligned}$$

Then  $\mathbf{D}_1^{-1}$  can be a negligible term.

The leading term of  $\mathbf{D}_1^{-1}[\mathbf{D}_1^{-1} + \mathbf{U}_1^\top \mathbf{G}_1(\tau) \mathbf{U}_1]^{-1} \mathbf{U}_1^\top \mathbf{G}_1(\tau)$  is

$$\begin{aligned}
& \mathbf{D}_1^{-1} \begin{pmatrix} \tau^{1/2} \mathbf{I}_r & \mathbf{0} \\ \mathbf{0} & \tau^{-1/2} \mathbf{I}_r \end{pmatrix} \begin{pmatrix} \{\mathbf{V}^\top [\mathbf{I}_N + m(-\tau) \mathbf{\Omega}]^{-1} \mathbf{V}\}^{-1} & \mathbf{0} \\ \mathbf{0} & -[m(-\tau)]^{-1} \mathbf{I}_r \end{pmatrix} \\
& \begin{pmatrix} \tau^{1/2} \mathbf{I}_r & \mathbf{0} \\ \mathbf{0} & \tau^{-1/2} \mathbf{I}_r \end{pmatrix} \mathbf{U}_1^\top \mathbf{G}_1(\tau) \\
= & \begin{pmatrix} \tau^{-1/2} \mathbf{I}_r & \mathbf{0} \\ \mathbf{0} & \tau^{1/2} \mathbf{I}_r \end{pmatrix} \mathbf{D}_1^{-1} \begin{pmatrix} \{\mathbf{V}^\top [\mathbf{I}_N + m(-\tau) \mathbf{\Omega}]^{-1} \mathbf{V}\}^{-1} & \mathbf{0} \\ \mathbf{0} & -[m(-\tau)]^{-1} \mathbf{I}_r \end{pmatrix} \\
& \begin{pmatrix} \mathbf{V}^\top [\mathbf{I}_N + m(-\tau) \mathbf{\Omega}]^{-1} & \mathbf{0} \\ \mathbf{0} & -m(-\tau) \mathbf{V}_1^\top \end{pmatrix} \begin{pmatrix} \tau^{-1/2} \mathbf{I}_N & \mathbf{0} \\ \mathbf{0} & \tau^{1/2} \mathbf{I}_T \end{pmatrix}.
\end{aligned}$$

Since non-zero elements of

$$\mathbf{D}_1^{-1} \begin{pmatrix} \{\mathbf{V}^\top [\mathbf{I}_N + m(-\tau) \mathbf{\Omega}]^{-1} \mathbf{V}\}^{-1} & \mathbf{0} \\ \mathbf{0} & -[m(-\tau)]^{-1} \mathbf{I}_r \end{pmatrix} \begin{pmatrix} \mathbf{V}^\top [\mathbf{I}_N + m(-\tau) \mathbf{\Omega}]^{-1} & \mathbf{0} \\ \mathbf{0} & -m(-\tau) \mathbf{V}_1^\top \end{pmatrix}$$

are in the off-diagonal blocks. Thus,

$$\begin{aligned}
& \mathbf{D}_1^{-1} \begin{pmatrix} \tau^{1/2} \mathbf{I}_r & \mathbf{0} \\ \mathbf{0} & \tau^{-1/2} \mathbf{I}_r \end{pmatrix} \begin{pmatrix} \{\mathbf{V}^\top [\mathbf{I}_N + m(-\tau) \mathbf{\Omega}]^{-1} \mathbf{V}\}^{-1} & \mathbf{0} \\ \mathbf{0} & -[m(-\tau)]^{-1} \mathbf{I}_r \end{pmatrix} \\
& \begin{pmatrix} \tau^{1/2} \mathbf{I}_r & \mathbf{0} \\ \mathbf{0} & \tau^{-1/2} \mathbf{I}_r \end{pmatrix} \mathbf{U}_1^\top \mathbf{G}_1(\tau) \\
= & \begin{pmatrix} \tau^{-1/2} \mathbf{I}_r & \mathbf{0} \\ \mathbf{0} & \tau^{1/2} \mathbf{I}_r \end{pmatrix} \mathbf{D}_1^{-1} \begin{pmatrix} \{\mathbf{V}^\top [\mathbf{I}_N + m(-\tau) \mathbf{\Omega}]^{-1} \mathbf{V}\}^{-1} & \mathbf{0} \\ \mathbf{0} & -[m(-\tau)]^{-1} \mathbf{I}_r \end{pmatrix} \\
& \begin{pmatrix} \mathbf{V}^\top [\mathbf{I}_N + m(-\tau) \mathbf{\Omega}]^{-1} & \mathbf{0} \\ \mathbf{0} & -m(-\tau) \mathbf{V}_1^\top \end{pmatrix} \begin{pmatrix} \tau^{-1/2} \mathbf{I}_N & \mathbf{0} \\ \mathbf{0} & \tau^{1/2} \mathbf{I}_T \end{pmatrix} \\
= & \mathbf{D}_1^{-1} \begin{pmatrix} \{\mathbf{V}^\top [\mathbf{I}_N + m(-\tau) \mathbf{\Omega}]^{-1} \mathbf{V}\}^{-1} & \mathbf{0} \\ \mathbf{0} & -[m(-\tau)]^{-1} \mathbf{I}_r \end{pmatrix} \\
& \begin{pmatrix} \mathbf{V}^\top [\mathbf{I}_N + m(-\tau) \mathbf{\Omega}]^{-1} & \mathbf{0} \\ \mathbf{0} & -m(-\tau) \mathbf{V}_1^\top \end{pmatrix}.
\end{aligned}$$

Thus,

$$\|\mathbf{D}_1^{-1}[\mathbf{D}_1^{-1} + \mathbf{U}_1^\top \mathbf{G}_1(\tau) \mathbf{U}_1]^{-1} \mathbf{U}_1^\top \mathbf{G}_1(\tau)\| = O_p(\|\mathbf{D}_1^{-1}\|). \quad (\text{S.3.14})$$

The leading term of  $\mathbf{D}_1^{-1}[\mathbf{D}_1^{-1} + \mathbf{U}_1^\top \mathbf{G}_1(\tau) \mathbf{U}_1]^{-1} \mathbf{D}_1^{-1}$  is

$$\begin{aligned}
& \mathbf{D}_1^{-1} \begin{pmatrix} \tau^{1/2} \mathbf{I}_r & \mathbf{0} \\ \mathbf{0} & \tau^{-1/2} \mathbf{I}_r \end{pmatrix} \begin{pmatrix} \{\mathbf{V}^\top [\mathbf{I}_N + m(-\tau) \mathbf{\Omega}]^{-1} \mathbf{V}\}^{-1} & \mathbf{0} \\ \mathbf{0} & -[m(-\tau)]^{-1} \mathbf{I}_r \end{pmatrix} \\
& \begin{pmatrix} \tau^{1/2} \mathbf{I}_r & \mathbf{0} \\ \mathbf{0} & \tau^{-1/2} \mathbf{I}_r \end{pmatrix} \mathbf{D}_1^{-1} \\
= & \begin{pmatrix} \tau^{-1/2} \mathbf{I}_r & \mathbf{0} \\ \mathbf{0} & \tau^{1/2} \mathbf{I}_r \end{pmatrix} \mathbf{D}_1^{-1} \begin{pmatrix} \{\mathbf{V}^\top [\mathbf{I}_N + m(-\tau) \mathbf{\Omega}]^{-1} \mathbf{V}\}^{-1} & \mathbf{0} \\ \mathbf{0} & -[m(-\tau)]^{-1} \mathbf{I}_r \end{pmatrix} \mathbf{D}_1^{-1} \\
& \begin{pmatrix} \tau^{-1/2} \mathbf{I}_r & \mathbf{0} \\ \mathbf{0} & \tau^{1/2} \mathbf{I}_r \end{pmatrix}.
\end{aligned}$$

Thus,

$$\|\mathbf{D}_1^{-1}[\mathbf{D}_1^{-1} + \mathbf{U}_1^\top \mathbf{G}_1(\tau) \mathbf{U}_1]^{-1} \mathbf{D}_1^{-1}\| = O_p(\tau^{-1} \|\mathbf{D}_1^{-1}\|^2). \quad (\text{S.3.15})$$

$$\begin{aligned}
& (\mathbf{a}^\top, \mathbf{0}_{1 \times T}) \mathbf{P}_{U_1}^\perp \mathbf{G}_1(\tau) \mathbf{U}_1 [\mathbf{D}_1^{-1} + \mathbf{U}_1^\top \mathbf{G}_1(\tau) \mathbf{U}_1]^{-1} \mathbf{U}_1^\top \mathbf{G}_1(\tau) \mathbf{P}_{U_1}^\perp (\mathbf{a}^\top, \mathbf{0}_{1 \times T})^\top \\
= & \tau^{-2} (\mathbf{a}^\top \mathbf{P}_V^\perp [\mathbf{I}_N + m(-\tau) \mathbf{\Omega}]^{-1} \mathbf{V}, \mathbf{0}) \begin{pmatrix} \mathbf{V}^\top \tau^{-1} [\mathbf{I}_N + m(-\tau) \mathbf{\Omega}]^{-1} \mathbf{V} & \mathbf{0} \\ \mathbf{0} & -\tau m(-\tau) \mathbf{I}_r \end{pmatrix}^{-1} \\
& (\mathbf{a}^\top \mathbf{P}_V^\perp [\mathbf{I}_N + m(-\tau) \mathbf{\Omega}]^{-1} \mathbf{V}, \mathbf{0})^\top [1 + o_p(1)] \\
= & \tau^{-1} \mathbf{a}^\top \mathbf{P}_V^\perp [\mathbf{I}_N + m(-\tau) \mathbf{\Omega}]^{-1} \mathbf{V} [\mathbf{V}^\top [\mathbf{I}_N + m(-\tau) \mathbf{\Omega}]^{-1} \mathbf{V}]^{-1} \mathbf{V}^\top [\mathbf{I}_N + m(-\tau) \mathbf{\Omega}]^{-1} \\
& \mathbf{P}_V^\perp \mathbf{a} [1 + o_p(1)],
\end{aligned}$$

Recall (S.2.21) and  $\|\mathbf{D}_1^{-1}\| = O_p(N^{-\delta/2}) = o_p(\|\mathbf{P}_V^\perp \mathbf{a}\|)$ ,

$$\begin{aligned}
& (\mathbf{a}^\top, \mathbf{0}_{1 \times T}) \mathbf{U}_1 \mathbf{D}_1^{-1} [\mathbf{D}_1^{-1} + \mathbf{U}_1^\top \mathbf{G}_1(\tau) \mathbf{U}_1]^{-1} \mathbf{U}_1^\top \mathbf{G}_1(\tau) \mathbf{P}_{U_1}^\perp (\mathbf{a}^\top, \mathbf{0}_{1 \times T})^\top \\
& = O_p(\tau^{-1} \|\mathbf{D}_1^{-1}\| \|\mathbf{P}_V^\perp \mathbf{a}\|) = o_p(\tau^{-1} \|\mathbf{P}_V^\perp \mathbf{a}\|^2).
\end{aligned}$$

$$\begin{aligned}
& (\mathbf{a}^\top, \mathbf{0}_{1 \times T}) \mathbf{U}_1 \mathbf{D}_1^{-1} [\mathbf{D}_1^{-1} + \mathbf{U}_1^\top \mathbf{G}_1(\tau) \mathbf{U}_1]^{-1} \mathbf{D}_1^{-1} \mathbf{U}_1^\top (\mathbf{a}^\top, \mathbf{0}_{1 \times T})^\top \\
= & O_p(\tau^{-1} \|\mathbf{D}_1^{-1}\|^2 \|\mathbf{V}^\top \mathbf{a}\|^2) = o_p(\tau^{-1} \|\mathbf{P}_V^\perp \mathbf{a}\|^2).
\end{aligned}$$

Thus,

$$\begin{aligned}
\mathbf{a}^\top \mathbf{S}_\tau^{-1} \mathbf{a} &= (\mathbf{a}^\top, \mathbf{0}_{1 \times T}) \mathbf{G}_2(\tau) (\mathbf{a}^\top, \mathbf{0}_{1 \times T})^\top \\
&= \tau^{-1} \mathbf{a}^\top \mathbf{P}_V^\perp [\mathbf{I}_N + m(-\tau) \boldsymbol{\Omega}]^{-1/2} (\mathbf{I}_N - \mathbf{P}_{[\mathbf{I}_N + m(-\tau) \boldsymbol{\Omega}]^{-1/2} \mathbf{V}}) [\mathbf{I}_N + m(-\tau) \boldsymbol{\Omega}]^{-1/2} \\
&\quad \mathbf{P}_V^\perp \mathbf{a} [1 + o_p(1)].
\end{aligned}$$

Note that

$$[\mathbf{I}_N - \mathbf{P}_{[\mathbf{I}_N + m(-\tau) \boldsymbol{\Omega}]^{-1/2} \mathbf{V}}] [\mathbf{I}_N + m(-\tau) \boldsymbol{\Omega}]^{-1/2} \mathbf{V} \mathbf{V}^\top = 0.$$

$$\begin{aligned}
\mathbf{a}^\top \mathbf{S}_\tau^{-1} \mathbf{a} &= (\mathbf{a}^\top, \mathbf{0}_{1 \times T}) \mathbf{G}_2(\tau) (\mathbf{a}^\top, \mathbf{0}_{1 \times T})^\top \\
&= \tau^{-1} \mathbf{a}^\top [\mathbf{I}_N + m(-\tau) \boldsymbol{\Omega}]^{-1/2} (\mathbf{I}_N - \mathbf{P}_{[\mathbf{I}_N + m(-\tau) \boldsymbol{\Omega}]^{-1/2} \mathbf{V}}) [\mathbf{I}_N + m(-\tau) \boldsymbol{\Omega}]^{-1/2} \mathbf{a} [1 + o_p(1)].
\end{aligned}$$

Recall (S.2.20),

$$\mathbf{a}^\top \mathbf{S}_\tau^{-1} \mathbf{a} = \tau^{-1} \tilde{\mathbf{a}}_\tau^\top \tilde{\mathbf{a}}_\tau [1 + o_p(1)]. \quad (\text{S.3.16})$$

### S.3.4 When $N \gg T$

When  $N \gg T$ ,

$$\begin{aligned}
\|N^{-1} \mathbf{Z}^\top \mathbf{Z} - \mathbf{I}_T\| &= O_p(N^{-1/2} T^{1/2}), \\
\|N^{-1} \mathbf{Z}^\top \boldsymbol{\Omega} \mathbf{Z} - N^{-1} \text{tr}(\boldsymbol{\Omega}) \mathbf{I}_T\| &= O_p(N^{-1/2} T^{1/2}).
\end{aligned}$$

Then the non-zero eigenvalues of  $T^{-1} \mathbf{Z} \mathbf{Z}^\top$  are  $T^{-1} N [1 + O_p(N^{-1/2} T^{1/2})]$ .

For any  $N$ -dimensional unit vectors  $\mathbf{b}$  and  $\mathbf{c}$ ,

$$\mathbf{b}^\top (\tau \boldsymbol{\Omega}^{-1} + T^{-1} \mathbf{Z} \mathbf{Z}^\top)^{-1} \mathbf{c} = \tau^{-1} \mathbf{b}^\top \boldsymbol{\Omega} \mathbf{c} - \tau^{-1} \mathbf{b}^\top \boldsymbol{\Omega} T^{-1} \mathbf{Z} \mathbf{Z}^\top (\tau \boldsymbol{\Omega}^{-1} + T^{-1} \mathbf{Z} \mathbf{Z}^\top)^{-1} \mathbf{c}.$$

Let  $\mathbf{z}_i$  be the  $i$ -th column of  $\mathbf{Z}$ .

$$\begin{aligned} & \mathbf{z}_i^\top (\tau \mathbf{\Omega}^{-1} + T^{-1} \mathbf{Z} \mathbf{Z}^\top)^{-1} - \mathbf{z}_i^\top (\tau \mathbf{\Omega}^{-1} + T^{-1} \sum_{j \neq i} \mathbf{z}_j \mathbf{z}_j^\top)^{-1} \\ = & -T^{-1} \mathbf{z}_i^\top (\tau \mathbf{\Omega}^{-1} + T^{-1} \sum_{j \neq i} \mathbf{z}_j \mathbf{z}_j^\top)^{-1} \mathbf{z}_i \mathbf{z}_i^\top (\tau \mathbf{\Omega}^{-1} + T^{-1} \mathbf{Z} \mathbf{Z}^\top)^{-1}. \end{aligned}$$

$$T^{-1} \mathbf{z}_i^\top (\tau \mathbf{\Omega}^{-1} + T^{-1} \sum_{j \neq i} \mathbf{z}_j \mathbf{z}_j^\top)^{-1} \mathbf{z}_i \geq 0,$$

$$\begin{aligned} & \mathbb{E}[T^{-1} \mathbf{z}_i^\top (\tau \mathbf{\Omega}^{-1} + T^{-1} \sum_{j \neq i} \mathbf{z}_j \mathbf{z}_j^\top)^{-1} \mathbf{z}_i] \\ = & T^{-1} \mathbb{E} \text{tr}[(\tau \mathbf{\Omega}^{-1} + T^{-1} \sum_{j \neq i} \mathbf{z}_j \mathbf{z}_j^\top)^{-1}] \asymp \tau^{-1} T^{-1} N \end{aligned}$$

and

$$\begin{aligned} & \text{Var}[T^{-1} \mathbf{z}_i^\top (\tau \mathbf{\Omega}^{-1} + T^{-1} \sum_{j \neq i} \mathbf{z}_j \mathbf{z}_j^\top)^{-1} \mathbf{z}_i] \\ = & O\{T^{-2} \mathbb{E} \text{tr}[(\tau \mathbf{\Omega}^{-1} + T^{-1} \sum_{j \neq i} \mathbf{z}_j \mathbf{z}_j^\top)^{-2}]\} = O(\tau^{-2} T^{-2} N). \end{aligned}$$

Thus,

$$\mathbf{z}_i^\top (\tau \mathbf{\Omega}^{-1} + T^{-1} \mathbf{Z} \mathbf{Z}^\top)^{-1} = \frac{\mathbf{z}_i^\top (\tau \mathbf{\Omega}^{-1} + T^{-1} \sum_{j \neq i} \mathbf{z}_j \mathbf{z}_j^\top)^{-1}}{1 + T^{-1} \mathbf{z}_i^\top (\tau \mathbf{\Omega}^{-1} + T^{-1} \sum_{j \neq i} \mathbf{z}_j \mathbf{z}_j^\top)^{-1} \mathbf{z}_i} \quad (\text{S.3.17})$$

and

$$\frac{1}{1 + T^{-1} \mathbf{z}_i^\top (\tau \mathbf{\Omega}^{-1} + T^{-1} \sum_{j \neq i} \mathbf{z}_j \mathbf{z}_j^\top)^{-1} \mathbf{z}_i} = O_p\left(\frac{1}{1 + \tau^{-1} T^{-1} N}\right).$$

$$\begin{aligned}
& \mathbf{b}^\top \Omega T^{-1} \mathbf{Z} \mathbf{Z}^\top (\tau \Omega^{-1} + T^{-1} \mathbf{Z} \mathbf{Z}^\top)^{-1} \mathbf{c} \\
= & T^{-1} \sum_{i=1}^T \mathbf{b}^\top \Omega \mathbf{z}_i \mathbf{z}_i^\top (\tau \Omega^{-1} + T^{-1} \mathbf{Z} \mathbf{Z}^\top)^{-1} \mathbf{c} \\
= & T^{-1} \sum_{i=1}^T \frac{\mathbf{b}^\top \Omega \mathbf{z}_i \mathbf{z}_i^\top (\tau \Omega^{-1} + T^{-1} \sum_{j \neq i} \mathbf{z}_j \mathbf{z}_j^\top)^{-1} \mathbf{c}}{1 + T^{-1} \mathbf{z}_i^\top (\tau \Omega^{-1} + T^{-1} \sum_{j \neq i} \mathbf{z}_j \mathbf{z}_j^\top)^{-1} \mathbf{z}_i}.
\end{aligned}$$

Note that

$$\mathbf{b}^\top \Omega \mathbf{z}_i \mathbf{z}_i^\top (\tau \Omega^{-1} + T^{-1} \sum_{j \neq i} \mathbf{z}_j \mathbf{z}_j^\top)^{-1} \mathbf{c} = O_p(\tau^{-1}).$$

Thus,

$$\begin{aligned}
& \mathbf{b}^\top \Omega T^{-1} \mathbf{Z} \mathbf{Z}^\top (\tau \Omega^{-1} + T^{-1} \mathbf{Z} \mathbf{Z}^\top)^{-1} \mathbf{c} \\
= & O_p\left(\frac{\tau^{-1}}{1 + \tau^{-1} T^{-1} N}\right) = O_p(N^{-1} T).
\end{aligned}$$

$$\mathbf{b}^\top (\tau \Omega^{-1} + T^{-1} \mathbf{Z} \mathbf{Z}^\top)^{-1} \mathbf{c} = \tau^{-1} \mathbf{b}^\top \Omega \mathbf{c} + O_p(\tau^{-1} N^{-1} T).$$

Similarly, for any  $N$ -dimensional unit vector  $\mathbf{b}$  and  $T$ -dimensional unit vector

$$\begin{aligned}
& T^{-1/2} \mathbf{b}^\top (\tau \Omega^{-1} + T^{-1} \mathbf{Z} \mathbf{Z}^\top)^{-1} \mathbf{Z} \mathbf{c} \\
= & \sum_{i=1}^T c_i T^{-1/2} \mathbf{b}^\top (\tau \Omega^{-1} + T^{-1} \mathbf{Z} \mathbf{Z}^\top)^{-1} \mathbf{z}_i \\
= & \sum_{i=1}^T c_i T^{-1/2} \frac{\mathbf{z}_i^\top (\tau \Omega^{-1} + T^{-1} \sum_{j \neq i} \mathbf{z}_j \mathbf{z}_j^\top)^{-1} \mathbf{b}}{1 + T^{-1} \mathbf{z}_i^\top (\tau \Omega^{-1} + T^{-1} \sum_{j \neq i} \mathbf{z}_j \mathbf{z}_j^\top)^{-1} \mathbf{z}_i} \\
= & O_p(N^{-1} T^{1/2}). \tag{S.3.18}
\end{aligned}$$

For any  $T$ -dimensional unit vector  $\mathbf{b}$  and  $\mathbf{c}$ , we use (S.3.17) to get

$$\begin{aligned}
& \mathbf{b}^\top T^{-1} \mathbf{Z}^\top (\tau \mathbf{\Omega}^{-1} + T^{-1} \mathbf{Z} \mathbf{Z}^\top)^{-1} \mathbf{Z} \mathbf{c} \\
= & \sum_{i=1}^T c_i T^{-1} \mathbf{b}^\top \mathbf{Z}^\top (\tau \mathbf{\Omega}^{-1} + T^{-1} \mathbf{Z} \mathbf{Z}^\top)^{-1} \mathbf{z}_i \\
= & \sum_{i=1}^T c_i T^{-1} \sum_{k=1}^T \frac{\mathbf{z}_i^\top (\tau \mathbf{\Omega}^{-1} + T^{-1} \sum_{j \neq i} \mathbf{z}_j \mathbf{z}_j^\top)^{-1} \mathbf{z}_k b_k}{1 + T^{-1} \mathbf{z}_i^\top (\tau \mathbf{\Omega}^{-1} + T^{-1} \sum_{j \neq i} \mathbf{z}_j \mathbf{z}_j^\top)^{-1} \mathbf{z}_i} \\
= & \sum_{i=1}^T b_i c_i \frac{T^{-1} \mathbf{z}_i^\top (\tau \mathbf{\Omega}^{-1} + T^{-1} \sum_{j \neq i} \mathbf{z}_j \mathbf{z}_j^\top)^{-1} \mathbf{z}_i}{1 + T^{-1} \mathbf{z}_i^\top (\tau \mathbf{\Omega}^{-1} + T^{-1} \sum_{j \neq i} \mathbf{z}_j \mathbf{z}_j^\top)^{-1} \mathbf{z}_i} \\
& + \sum_{i=1}^T \sum_{k \neq i} b_k c_i \frac{T^{-1} \mathbf{z}_i^\top (\tau \mathbf{\Omega}^{-1} + T^{-1} \sum_{j \neq i} \mathbf{z}_j \mathbf{z}_j^\top)^{-1} \mathbf{z}_k}{1 + T^{-1} \mathbf{z}_i^\top (\tau \mathbf{\Omega}^{-1} + T^{-1} \sum_{j \neq i} \mathbf{z}_j \mathbf{z}_j^\top)^{-1} \mathbf{z}_i} \\
= & \sum_{i=1}^T b_i c_i \frac{T^{-1} \mathbf{z}_i^\top (\tau \mathbf{\Omega}^{-1} + T^{-1} \sum_{j \neq i} \mathbf{z}_j \mathbf{z}_j^\top)^{-1} \mathbf{z}_i}{1 + T^{-1} \mathbf{z}_i^\top (\tau \mathbf{\Omega}^{-1} + T^{-1} \sum_{j \neq i} \mathbf{z}_j \mathbf{z}_j^\top)^{-1} \mathbf{z}_i} \\
& + \sum_{i=1}^T \sum_{k \neq i} \frac{b_k c_i T^{-1} \mathbf{z}_i^\top (\tau \mathbf{\Omega}^{-1} + T^{-1} \sum_{j \neq i, k} \mathbf{z}_j \mathbf{z}_j^\top)^{-1} \mathbf{z}_k}{1 + T^{-1} \mathbf{z}_i^\top (\tau \mathbf{\Omega}^{-1} + T^{-1} \sum_{j \neq i} \mathbf{z}_j \mathbf{z}_j^\top)^{-1} \mathbf{z}_i} \\
& \frac{1}{1 + T^{-1} \mathbf{z}_k^\top (\tau \mathbf{\Omega}^{-1} + T^{-1} \sum_{j \neq i, k} \mathbf{z}_j \mathbf{z}_j^\top)^{-1} \mathbf{z}_k} \\
= & \mathbf{b}^\top \mathbf{c} [1 + O_p(\tau N^{-1} T)] + o_p(N^{-1} T).
\end{aligned}$$

These, together with (S.3.2) and (S.3.3), imply that for any  $N + T$ -dimensional unit vector  $\mathbf{b}$  and  $\mathbf{c}$ ,

$$\mathbf{b}^\top \mathbf{G}^{(\emptyset)} \mathbf{c} = \mathbf{b}^\top \begin{pmatrix} \tau^{-1} \mathbf{\Omega} & \mathbf{0} \\ \mathbf{0} & \mathbf{0} \end{pmatrix} \mathbf{c} + O_p(\tau^{-1} N^{-1} T)$$

Recalling that

$$\mathbf{H}^{-1} = \mathbf{G}^{(\emptyset)} = \begin{pmatrix} \mathbf{\Omega}^{1/2} & \mathbf{0} \\ \mathbf{0} & \mathbf{I}_T \end{pmatrix} \mathbf{G}_1(\tau) \begin{pmatrix} \mathbf{\Omega}^{1/2} & \mathbf{0} \\ \mathbf{0} & \mathbf{I}_T \end{pmatrix}.$$

We find that

$$\mathbf{b}^\top \mathbf{G}_1(\tau) \mathbf{c} = \tau^{-1} \mathbf{b}^\top \begin{pmatrix} \mathbf{I}_N & \mathbf{0} \\ \mathbf{0} & \mathbf{0} \end{pmatrix} \mathbf{c} + O_p(\tau^{-1} N^{-1} T).$$

Recalling (S.2.15),

$$\begin{aligned}
& \mathbf{a}^\top \mathbf{S}_\tau^{-1} \mathbf{a} = (\mathbf{a}^\top, \mathbf{0}_{1 \times T}) \mathbf{G}_2(\tau) (\mathbf{a}^\top, \mathbf{0}_{1 \times T})^\top \\
= & (\mathbf{a}^\top, \mathbf{0}_{1 \times T}) \mathbf{P}_{U_1}^\perp \mathbf{G}_1(\tau) \mathbf{P}_{U_1}^\perp (\mathbf{a}^\top, \mathbf{0}_{1 \times T})^\top \\
& - (\mathbf{a}^\top, \mathbf{0}_{1 \times T}) \mathbf{P}_{U_1}^\perp \mathbf{G}_1(\tau) \mathbf{U}_1 \left[ \mathbf{D}_1^{-1} + \mathbf{U}_1^\top \mathbf{G}_1(\tau) \mathbf{U}_1 \right]^{-1} \mathbf{U}_1^\top \mathbf{G}_1(\tau) \mathbf{P}_{U_1}^\perp (\mathbf{a}^\top, \mathbf{0}_{1 \times T})^\top \\
& + 2(\mathbf{a}^\top, \mathbf{0}_{1 \times T}) \mathbf{U}_1 \mathbf{D}_1^{-1} [\mathbf{D}_1^{-1} + \mathbf{U}_1^\top \mathbf{G}_1(\tau) \mathbf{U}_1]^{-1} \mathbf{U}_1^\top \mathbf{G}_1(\tau) \mathbf{P}_{U_1}^\perp (\mathbf{a}^\top, \mathbf{0}_{1 \times T})^\top \\
& - (\mathbf{a}^\top, \mathbf{0}_{1 \times T}) \mathbf{U}_1 \mathbf{D}_1^{-1} [\mathbf{D}_1^{-1} + \mathbf{U}_1^\top \mathbf{G}_1(\tau) \mathbf{U}_1]^{-1} \mathbf{D}_1^{-1} \mathbf{U}_1^\top (\mathbf{a}^\top, \mathbf{0}_{1 \times T})^\top
\end{aligned}$$

$$(\mathbf{a}^\top, \mathbf{0}_{1 \times T}) \mathbf{P}_{U_1}^\perp \mathbf{G}_1(\tau) \mathbf{P}_{U_1}^\perp (\mathbf{a}^\top, \mathbf{0}_{1 \times T})^\top = \tau^{-1} \|\mathbf{P}_V^\perp \mathbf{a}\|^2 [1 + O_p(N^{-1}T)].$$

The other terms can be controlled by the same method as the case  $N \asymp T$ . The only difference is in  $[\mathbf{D}_1^{-1} + \mathbf{U}_1^\top \mathbf{G}_1(\tau) \mathbf{U}_1]^{-1}$ . We can rewrite  $\mathbf{D}_1^{-1} + \mathbf{U}_1^\top \mathbf{G}_1(\tau) \mathbf{U}_1$  as

$$\begin{aligned}
& \mathbf{D}_1^{-1} + \mathbf{U}_1^\top \mathbf{G}_1(\tau) \mathbf{U}_1 \\
= & \begin{pmatrix} \tau^{-1}(\mathbf{I}_r + \mathbf{M}_1) & T^{1/2}(\mathbf{B}_1^\top)^{-1}(\mathbf{F}_1^\top)^{-1} + \mathbf{M}_2 \\ T^{1/2}\mathbf{F}_1^{-1}\mathbf{B}_1^{-1} + \mathbf{M}_2^\top & \mathbf{M}_3 \end{pmatrix}.
\end{aligned}$$

$\|\mathbf{M}_1\| = O_p(N^{-1}T) = o_p(1)$ . (S.3.18) implies that  $\|\mathbf{M}_2\| = O_p(N^{-1}T^{1/2})$ . The order of  $\mathbf{M}_3$  is  $\tau N^{-1}T$ , when  $N \gg T$ , its order is  $o(1)$ . Recall (S.2.11), non-zero elements of  $\mathbf{D}_1$  and  $\mathbf{D}_1^{-1}$  are in the off-diagonal block.

$$\begin{aligned}
& \mathbf{D}_1^{-1} \\
= & \begin{pmatrix} \tau^{-1/2}N^{1/4}T^{-1/4}\mathbf{I}_r & \mathbf{0} \\ \mathbf{0} & \tau^{1/2}N^{-1/4}T^{1/4}\mathbf{I}_r \end{pmatrix} \mathbf{D}_1^{-1} \begin{pmatrix} \tau^{-1/2}N^{1/4}T^{-1/4}\mathbf{I}_r & \mathbf{0} \\ \mathbf{0} & \tau^{1/2}N^{-1/4}T^{1/4}\mathbf{I}_r \end{pmatrix} \\
& \mathbf{U}_1^\top \mathbf{G}_1(\tau) \mathbf{U}_1 \\
= & \begin{pmatrix} \tau^{-1/2}N^{1/4}T^{-1/4}\mathbf{I}_r & \mathbf{0} \\ \mathbf{0} & \tau^{1/2}N^{-1/4}T^{1/4}\mathbf{I}_r \end{pmatrix} \begin{pmatrix} N^{-1/2}T^{1/2}(\mathbf{I}_r + \mathbf{M}_1) & \mathbf{M}_2 \\ \mathbf{M}_2^\top & \tau^{-1}N^{1/2}T^{1/2}\mathbf{M}_3 \end{pmatrix} \\
& \begin{pmatrix} \tau^{-1/2}N^{1/4}T^{-1/4}\mathbf{I}_r & \mathbf{0} \\ \mathbf{0} & \tau^{1/2}N^{-1/4}T^{1/4}\mathbf{I}_r \end{pmatrix}.
\end{aligned}$$

$\|\tau^{-1}N^{1/2}T^{-1/2}\mathbf{M}_3\| \asymp \|N^{-1/2}T^{1/2}(\mathbf{I}_r + \mathbf{M}_1)\| \asymp N^{-1/2}T^{1/2}$  in probability. Since  $\|\mathbf{D}_1^{-1}\| \asymp N^{-\delta/2} = o(N^{-1/2}T^{1/2})$ . Thus, the impact of  $\mathbf{D}_1^{-1}$  can still be controlled.

Then

$$\begin{aligned}
& \mathbf{a}^\top \mathbf{S}_\tau^{-1} \mathbf{a} = (\mathbf{a}^\top, \mathbf{0}_{1 \times T}) \mathbf{G}_2(\tau) (\mathbf{a}^\top, \mathbf{0}_{1 \times T})^\top \\
&= (\mathbf{a}^\top, \mathbf{0}_{1 \times T}) \mathbf{P}_{U_1}^\perp \mathbf{G}_1(\tau) \mathbf{P}_{U_1}^\perp (\mathbf{a}^\top, \mathbf{0}_{1 \times T})^\top \\
&\quad - (\mathbf{a}^\top, \mathbf{0}_{1 \times T}) \mathbf{P}_{U_1}^\perp \mathbf{G}_1(\tau) \mathbf{U}_1 \left[ \mathbf{D}_1^{-1} + \mathbf{U}_1^\top \mathbf{G}_1(\tau) \mathbf{U}_1 \right]^{-1} \mathbf{U}_1^\top \mathbf{G}_1(\tau) \mathbf{P}_{U_1}^\perp (\mathbf{a}^\top, \mathbf{0}_{1 \times T})^\top \\
&\quad + 2(\mathbf{a}^\top, \mathbf{0}_{1 \times T}) \mathbf{U}_1 \mathbf{D}_1^{-1} [\mathbf{D}_1^{-1} + \mathbf{U}_1^\top \mathbf{G}_1(\tau) \mathbf{U}_1]^{-1} \mathbf{U}_1^\top \mathbf{G}_1(\tau) \mathbf{P}_{U_1}^\perp (\mathbf{a}^\top, \mathbf{0}_{1 \times T})^\top \\
&\quad - (\mathbf{a}^\top, \mathbf{0}_{1 \times T}) \mathbf{U}_1 \mathbf{D}_1^{-1} [\mathbf{D}_1^{-1} + \mathbf{U}_1^\top \mathbf{G}_1(\tau) \mathbf{U}_1]^{-1} \mathbf{D}_1^{-1} \mathbf{U}_1^\top (\mathbf{a}^\top, \mathbf{0}_{1 \times T})^\top \\
&= \tau^{-1} \|\mathbf{P}_V^\perp \mathbf{a}\|^2 [1 + O_p(N^{-1}T)] + O_p(\tau^{-1}N^{1-\delta}T^{-1} \|\mathbf{V}^\top \mathbf{a}\|^2).
\end{aligned}$$

Recall (S.2.21),  $\|\mathbf{P}_V^\perp \mathbf{a}\|^2 \gg N^{1-\delta}T^{-1} \geq N^{1-\delta}T^{-1} \|\mathbf{V}^\top \mathbf{a}\|^2$ ,

$$\mathbf{a}^\top \mathbf{S}_\tau^{-1} \mathbf{a} = \tau^{-1} \mathbf{a}^\top \mathbf{P}_V^\perp \mathbf{a} [1 + O_p(TN^{-1}) + o_p(1)]. \quad (\text{S.3.19})$$

## S.4 The limit of $\mathbf{a}^\top \mathbf{S}_\tau^{-1} \Sigma \mathbf{S}_\tau^{-1} \mathbf{a}$

In this section we study the limit of  $\mathbf{a}^\top \mathbf{S}_\tau^{-1} \Sigma \mathbf{S}_\tau^{-1} \mathbf{a}$ . Then we can prove (S.1.7) and (S.1.10).

Recall (S.2.16),

$$\begin{aligned}
& \mathbf{a}^\top \mathbf{S}_\tau^{-1} \Sigma \mathbf{S}_\tau^{-1} \mathbf{a} \\
&= (\mathbf{a}^\top, \mathbf{0}_{1 \times T}) \mathbf{P}_{U_1}^\perp \mathbf{G}_2(\tau) \tilde{\Omega} \mathbf{G}_2(\tau) \mathbf{P}_{U_1}^\perp (\mathbf{a}^\top, \mathbf{0}_{1 \times T})^\top \\
&\quad + 2(\mathbf{a}^\top, \mathbf{0}_{1 \times T}) \mathbf{U}_1 \mathbf{D}_1^{-1} [\mathbf{D}_1^{-1} + \mathbf{U}_1^\top \mathbf{G}_1(\tau) \mathbf{U}_1]^{-1} \mathbf{U}_1^\top \mathbf{G}_1(\tau) \tilde{\Omega} \mathbf{G}_2(\tau) \mathbf{P}_{U_1}^\perp (\mathbf{a}^\top, \mathbf{0}_{1 \times T})^\top \\
&\quad + (\mathbf{a}^\top, \mathbf{0}_{1 \times T}) \mathbf{U}_1 \mathbf{D}_1^{-1} [\mathbf{D}_1^{-1} + \mathbf{U}_1^\top \mathbf{G}_1(\tau) \mathbf{U}_1]^{-1} \mathbf{U}_1^\top \mathbf{G}_1(\tau) \tilde{\Omega} \mathbf{G}_1(\tau) \mathbf{U}_1 [\mathbf{D}_1^{-1} + \mathbf{U}_1^\top \mathbf{G}_1(\tau) \mathbf{U}_1]^{-1} \\
&\quad \mathbf{D}_1^{-1} \mathbf{U}_1^\top (\mathbf{a}^\top, \mathbf{0}_{1 \times T})^\top + (\mathbf{a}^\top, \mathbf{0}_{1 \times T}) \mathbf{G}_2(\tau) \begin{pmatrix} \mathbf{B}\mathbf{B}^\top & \mathbf{0} \\ \mathbf{0}^\top & \mathbf{0} \end{pmatrix} \mathbf{G}_2(\tau) (\mathbf{a}^\top, \mathbf{0}_{1 \times T})^\top,
\end{aligned}$$

where

$$\tilde{\Omega} = \begin{pmatrix} \Omega & \mathbf{0} \\ \mathbf{0} & \mathbf{0} \end{pmatrix}.$$

### S.4.1 The leading term of $\mathbf{a}^\top \mathbf{S}_\tau^{-1} \Sigma \mathbf{S}_\tau^{-1} \mathbf{a}$

In this section, we define

$$\mathbf{M} = \begin{pmatrix} \Omega^{1/2} & \mathbf{0} \\ \mathbf{0} & \mathbf{I}_T \end{pmatrix} \mathbf{G}_1(\tau) \tilde{\Omega} \mathbf{G}_1(\tau) \begin{pmatrix} \Omega^{1/2} & \mathbf{0} \\ \mathbf{0} & \mathbf{I}_T \end{pmatrix} = \mathbf{G}^{(\emptyset)} \begin{pmatrix} \mathbf{I}_N & \mathbf{0} \\ \mathbf{0} & \mathbf{0} \end{pmatrix} \mathbf{G}^{(\emptyset)} \quad (\text{S.4.1})$$

Rewrite

$$\mathbf{M} = \begin{pmatrix} \mathbf{M}_{11} & \mathbf{M}_{12} \\ \mathbf{M}_{21} & \mathbf{M}_{22} \end{pmatrix} \quad (\text{S.4.2})$$

where  $\mathbf{M}_{11}$  is a  $N \times N$  matrix.

Now we focus on  $\mathbf{M}_{11}$ . Let  $M_{st}$  be the  $(s, t)$  entry of  $\mathbf{M}_{11}$ .

Then for  $1 \leq s \neq t \leq N$ , recall (S.3.8), (S.3.6) and (S.3.2),

$$\begin{aligned} M_{ss} &= \sum_{k=1}^N G_{sk}^2 \\ &= \sum_{k \neq s} T^{-1} G_{ss}^2 (\tilde{\mathbf{z}}_s^\top \mathbf{G}^{(s)})_k^2 + G_{ss}^2 \\ &= G_{ss}^2 \left[ \sum_{k \neq s} T^{-1} (\tilde{\mathbf{z}}_s^\top \mathbf{G}^{(s)})_k^2 + 1 \right] \\ &= \frac{1}{(\tau \theta_s^{-1} - T^{-1} \tilde{\mathbf{z}}_s^\top \mathbf{G}^{(s)} \tilde{\mathbf{z}}_s)^2} \left[ \sum_{k \neq s} T^{-1} (\tilde{\mathbf{z}}_s^\top \mathbf{G}^{(s)})_k^2 + 1 \right] \\ &= \frac{1}{(\tau \theta_s^{-1} - T^{-1} \sum_{i=N+1}^{T+N} G_{ii}^{(s)})^2} \left[ T^{-1} \sum_{i=N+1}^{T+N} \sum_{j \neq s}^N [G_{ij}^{(s)}]^2 + 1 \right] [1 + O_p(T^{-1/2})] \\ &= \frac{1}{\tau^2 [\theta_s^{-1} + m(-\tau)]^2} [T^{-2} \text{tr}\{\mathbf{Z}^\top (\tau \Omega^{-1} + T^{-1} \mathbf{Z} \mathbf{Z}^\top)^{-2} \mathbf{Z}\} + 1] [1 + O_p(T^{-1/2})]. \end{aligned} \quad (\text{S.4.3})$$

$$\begin{aligned} M_{st} &= \sum_{k=1}^N G_{sk} G_{kt} \\ &= (G_{ss} + G_{tt}) G_{st} + G_{ss} G_{tt} \sum_{k \neq s, t; 1 \leq k \leq N} T^{-1} (\tilde{\mathbf{z}}_s^\top \mathbf{G}^{(s)})_k (\tilde{\mathbf{z}}_t^\top \mathbf{G}^{(t)})_k \\ &= O_p(\tau^{-2} T^{-1/2}). \end{aligned} \quad (\text{S.4.4})$$

Let  $\mathbf{z}_i$  be the  $i$ th column of  $\mathbf{Z}$ ,  $\mathbf{Z}\mathbf{Z}^\top = \sum_{i=1}^T \mathbf{z}_i \mathbf{z}_i^\top$ .

$$\begin{aligned}
& (\tau\mathbf{\Omega}^{-1} + T^{-1}\mathbf{Z}\mathbf{Z}^\top)^{-1}\mathbf{z}_i \\
= & (\tau\mathbf{\Omega}^{-1} + T^{-1}\sum_{j \neq i} \mathbf{z}_j \mathbf{z}_j^\top)^{-1}\mathbf{z}_i - (\tau\mathbf{\Omega}^{-1} + T^{-1}\mathbf{Z}\mathbf{Z}^\top)^{-1}T^{-1}\mathbf{z}_i \mathbf{z}_i^\top (\tau\mathbf{\Omega}^{-1} + T^{-1}\sum_{j \neq i} \mathbf{z}_j \mathbf{z}_j^\top)^{-1}\mathbf{z}_i.
\end{aligned}$$

Thus,

$$\begin{aligned}
& (\tau\mathbf{\Omega}^{-1} + T^{-1}\mathbf{Z}\mathbf{Z}^\top)^{-1}\mathbf{z}_i \\
= & \frac{(\tau\mathbf{\Omega}^{-1} + T^{-1}\sum_{j \neq i} \mathbf{z}_j \mathbf{z}_j^\top)^{-1}\mathbf{z}_i}{1 + T^{-1}\mathbf{z}_i^\top (\tau\mathbf{\Omega}^{-1} + T^{-1}\sum_{j \neq i} \mathbf{z}_j \mathbf{z}_j^\top)^{-1}\mathbf{z}_i}.
\end{aligned}$$

$$\begin{aligned}
& T^{-2}\text{tr}[\mathbf{Z}^\top (\tau\mathbf{\Omega}^{-1} + T^{-1}\mathbf{Z}\mathbf{Z}^\top)^{-2}\mathbf{Z}] \\
= & T^{-2}\sum_{i=1}^T \mathbf{z}_i^\top (\tau\mathbf{\Omega}^{-1} + T^{-1}\mathbf{Z}^\top \mathbf{Z})^{-2}\mathbf{z}_i \\
= & T^{-2}\sum_{i=1}^T \|(\tau\mathbf{\Omega}^{-1} + T^{-1}\mathbf{Z}\mathbf{Z}^\top)^{-1}\mathbf{z}_i\|^2 \\
= & T^{-2}\sum_{i=1}^T \left\| \frac{(\tau\mathbf{\Omega}^{-1} + T^{-1}\sum_{j \neq i} \mathbf{z}_j \mathbf{z}_j^\top)^{-1}\mathbf{z}_i}{1 + T^{-1}\mathbf{z}_i^\top (\tau\mathbf{\Omega}^{-1} + T^{-1}\sum_{j \neq i} \mathbf{z}_j \mathbf{z}_j^\top)^{-1}\mathbf{z}_i} \right\|^2 \\
= & \frac{T^{-1}\text{tr}[(\tau\mathbf{\Omega}^{-1} + T^{-1}\sum_{j \neq i} \mathbf{z}_j \mathbf{z}_j^\top)^{-2}]}{\{1 + T^{-1}\text{tr}[(\tau\mathbf{\Omega}^{-1} + T^{-1}\sum_{j \neq i} \mathbf{z}_j \mathbf{z}_j^\top)^{-1}]\}^2} [1 + O_p(T^{-1/2})] \\
= & \frac{T^{-1}\text{tr}[(\tau\mathbf{\Omega}^{-1} + T^{-1}\mathbf{Z}\mathbf{Z}^\top)^{-2}]}{\{1 + T^{-1}\text{tr}[(\tau\mathbf{\Omega}^{-1} + T^{-1}\mathbf{Z}\mathbf{Z}^\top)^{-1}]\}^2} [1 + O_p(T^{-1/2})].
\end{aligned}$$

This convergence rate  $O_p(T^{-1/2})$  stems from the theoretical properties of quadratic forms.

(S.3.3) and (S.3.5) implies that

$$\begin{aligned}
& 1 + T^{-1} \text{tr}[(\tau \mathbf{\Omega}^{-1} + T^{-1} \mathbf{Z} \mathbf{Z}^\top)^{-1}] \\
= & 1 + T^{-1} \tau^{-1} \sum_{i=1}^N \frac{\theta_i}{1 + \theta_i m(-\tau)} [1 + O_p(T^{-1/2})] \\
= & \tau^{-1} \left[ \tau + T^{-1} \sum_{i=1}^N \frac{\theta_i}{1 + \theta_i m(-\tau)} \right] [1 + O_p(T^{-1/2})] \\
= & \frac{\tau^{-1}}{m(-\tau)} [1 + O_p(T^{-1/2})].
\end{aligned}$$

The last equation is from (S.10.1).

$$\begin{aligned}
& T^{-2} \text{tr}[\mathbf{Z}^\top (\tau \mathbf{\Omega}^{-1} + T^{-1} \mathbf{Z} \mathbf{Z}^\top)^{-2} \mathbf{Z}] \\
= & \frac{T^{-1} \text{tr}[(\tau \mathbf{\Omega}^{-1} + T^{-1} \mathbf{Z} \mathbf{Z}^\top)^{-2}]}{\tau^{-2} \frac{1}{m^2(-\tau)}} [1 + O_p(T^{-1/2})] \\
= & T^{-1} \text{tr}[(\tau \mathbf{\Omega}^{-1} + T^{-1} \mathbf{Z} \mathbf{Z}^\top)^{-2}] \tau^2 m^2(-\tau) [1 + O_p(T^{-1/2})] \\
= & T^{-1} \sum_{i=1}^N M_{ii} \tau^2 m^2(-\tau) [1 + O_p(T^{-1/2})] \\
= & T^{-1} \sum_{s=1}^N \frac{\theta_s^2 m^2(-\tau)}{[1 + \theta_s m(-\tau)]^2} [T^{-2} \text{tr}\{\mathbf{Z}^\top (\tau \mathbf{\Omega}^{-1} + T^{-1} \mathbf{Z} \mathbf{Z}^\top)^{-2} \mathbf{Z}\} + 1] [1 + O_p(T^{-1/2})].
\end{aligned}$$

The last equation is from (S.4.3). Thus,

$$\begin{aligned}
& T^{-2} \text{tr}[\mathbf{Z}^\top (\tau \mathbf{\Omega}^{-1} + T^{-1} \mathbf{Z} \mathbf{Z}^\top)^{-2} \mathbf{Z}] \\
= & \frac{T^{-1} \sum_{s=1}^N \frac{\theta_s^2 m^2(-\tau)}{[1 + \theta_s m(-\tau)]^2}}{1 - T^{-1} \sum_{s=1}^N \frac{\theta_s^2 m^2(-\tau)}{[1 + \theta_s m(-\tau)]^2}} [1 + O_p(T^{-1/2})] \\
= & \frac{T^{-1} m^2(-\tau) \text{tr}\{\mathbf{\Omega}[\mathbf{I}_N + m(-\tau)\mathbf{\Omega}]^{-2} \mathbf{\Omega}\}}{1 - T^{-1} m^2(-\tau) \text{tr}\{\mathbf{\Omega}[\mathbf{I}_N + m(-\tau)\mathbf{\Omega}]^{-2} \mathbf{\Omega}\}} [1 + O_p(T^{-1/2})] \\
= & [c(\tau) - 1] [1 + O_p(T^{-1/2})].
\end{aligned}$$

The last equation is from the definition of  $c(\tau)$  in (S.1.5). This, together with (S.4.3),

implies

$$\begin{aligned}
M_{ss} &= \sum_{k=1}^N G_{sk}^2 \\
&= \frac{1}{\tau^2[\theta_s^{-1} + m(-\tau)]^2} \frac{1}{1 - T^{-1}m^2(-\tau)\text{tr}\{\boldsymbol{\Omega}[\mathbf{I}_N + m(-\tau)\boldsymbol{\Omega}]^{-2}\boldsymbol{\Omega}\}} [1 + O_p(T^{-1/2})] \\
&= \frac{c(\tau)}{\tau^2[\theta_s^{-1} + m(-\tau)]^2} [1 + O_p(T^{-1/2})]. \tag{S.4.5}
\end{aligned}$$

(S.4.4) and (S.4.5) imply a similar result in Lemma S.8 for  $\mathbf{M}_{11}$ . Based on it, we can follow section 6 in Knowles and Yin (2017) to get a similar result of (S.3.5) for  $\mathbf{M}_{11}$ .

Thus, for any  $N$ -dimensional unit vector  $\mathbf{b}$  and  $\mathbf{c}$ ,

$$\begin{aligned}
&\mathbf{b}^\top \boldsymbol{\Omega}^{-1/2} \mathbf{M}_{11} \boldsymbol{\Omega}^{-1/2} \mathbf{c} \\
&= \tau^{-2} \{T^{-2} \text{tr}[\mathbf{Z}(\tau\boldsymbol{\Omega}^{-1} + T^{-1}\mathbf{Z}^\top \mathbf{Z})^{-2}\mathbf{Z}^\top] + 1\} \mathbf{b}^\top \boldsymbol{\Omega}^{-1/2} [m(-\tau)\mathbf{I}_N + \boldsymbol{\Omega}^{-1}]^{-2} \boldsymbol{\Omega}^{-1/2} \mathbf{c} [1 + o_p(1)] \\
&= \tau^{-2} \frac{\mathbf{b}^\top \boldsymbol{\Omega}^{1/2} [m(-\tau)\boldsymbol{\Omega} + \mathbf{I}_N]^{-2} \boldsymbol{\Omega}^{1/2} \mathbf{c}}{1 - T^{-1}m^2(-\tau)\text{tr}\{\boldsymbol{\Omega}[\mathbf{I}_N + m(-\tau)\boldsymbol{\Omega}]^{-2}\boldsymbol{\Omega}\}} [1 + o_p(1)] \\
&= \tau^{-2} c(\tau) \mathbf{b}^\top \boldsymbol{\Omega}^{1/2} [m(-\tau)\boldsymbol{\Omega} + \mathbf{I}_N]^{-2} \boldsymbol{\Omega}^{1/2} \mathbf{c} [1 + o_p(1)]. \tag{S.4.6}
\end{aligned}$$

Thus,  $\mathbf{b}^\top \mathbf{M}_{11} \mathbf{b} \asymp \tau^{-2}$  in probability. Similarly,

$$\mathbf{M}_{21}^\top = \mathbf{M}_{12} = T^{-1/2}(\tau\boldsymbol{\Omega}^{-1} + T^{-1}\mathbf{Z}\mathbf{Z}^\top)^{-2}\mathbf{Z}$$

and

$$\mathbf{M}_{22} = T^{-1}\mathbf{Z}^\top (\tau\boldsymbol{\Omega}^{-1} + T^{-1}\mathbf{Z}\mathbf{Z}^\top)^{-2}\mathbf{Z}.$$

$$\begin{aligned}
&\|\mathbf{M}_{12}^\top \mathbf{M}_{12}\| \\
&= \|T^{-1}\mathbf{Z}^\top (\tau\boldsymbol{\Omega}^{-1} + T^{-1}\mathbf{Z}\mathbf{Z}^\top)^{-4}\mathbf{Z}\| \\
&= O(\|T^{-1}\mathbf{Z}\mathbf{Z}^\top\|_{\min}^{-3}) = O_p(N^{-3}T^3).
\end{aligned}$$

$$\begin{aligned}
& \|\mathbf{M}_{22}\| \\
&= \|T^{-1}\mathbf{Z}^\top (\tau\boldsymbol{\Omega}^{-1} + T^{-1}\mathbf{Z}\mathbf{Z}^\top)^{-2}\mathbf{Z}\| \\
&= O(\|T^{-1}\mathbf{Z}\mathbf{Z}^\top\|_{min}^{-1}) = O_p(N^{-1}T).
\end{aligned}$$

From  $\tau = o(\|\mathbf{P}_V^\perp \mathbf{a}\|)$ , for any random or non-random  $(N+T)$ -dimensional unit vector  $\mathbf{b}$  and  $\mathbf{c}$ ,

$$\begin{aligned}
\mathbf{b}^\top \mathbf{M} \mathbf{c} &= \mathbf{b}^\top \begin{pmatrix} \mathbf{M}_{11} & \mathbf{M}_{12} \\ \mathbf{M}_{21} & \mathbf{M}_{22} \end{pmatrix} \mathbf{c} = \mathbf{b}^\top \begin{pmatrix} \mathbf{M}_{11} & \mathbf{0} \\ \mathbf{0} & \mathbf{0} \end{pmatrix} \mathbf{c} + O(\|\mathbf{M}_{12}\| + \|\mathbf{M}_{22}\|) \\
&= \mathbf{b}^\top \begin{pmatrix} \mathbf{M}_{11} & \mathbf{0} \\ \mathbf{0} & \mathbf{0} \end{pmatrix} \mathbf{c} + o(N^{-1}T\tau^{-2}\|\mathbf{P}_V^\perp \mathbf{a}\|^2) \\
&= \mathbf{b}^\top \begin{pmatrix} \mathbf{M}_{11} & \mathbf{0} \\ \mathbf{0} & \mathbf{0} \end{pmatrix} \mathbf{c} + o(\tau^{-2}\|\mathbf{P}_V^\perp \mathbf{a}\|^2). \tag{S.4.7}
\end{aligned}$$

At first, we consider this term

$$\begin{aligned}
& (\mathbf{a}^\top, \mathbf{0}_{1 \times T}) \mathbf{P}_{U_1}^\perp \mathbf{G}_2(\tau) \tilde{\boldsymbol{\Omega}} \mathbf{G}_2(\tau) \mathbf{P}_{U_1}^\perp (\mathbf{a}^\top, \mathbf{0}_{1 \times T})^\top \\
&= (\mathbf{a}^\top, \mathbf{0}_{1 \times T}) \mathbf{P}_{U_1}^\perp \mathbf{G}_1(\tau) \tilde{\boldsymbol{\Omega}} \mathbf{G}_1(\tau) \mathbf{P}_{U_1}^\perp (\mathbf{a}^\top, \mathbf{0}_{1 \times T})^\top - \\
& \quad 2(\mathbf{a}^\top, \mathbf{0}_{1 \times T}) \mathbf{P}_{U_1}^\perp \mathbf{G}_1(\tau) \tilde{\boldsymbol{\Omega}} \mathbf{G}_1(\tau) \mathbf{U}_1 [\mathbf{D}_1^{-1} + \mathbf{U}_1^\top \mathbf{G}_1(\tau) \mathbf{U}_1]^{-1} \\
& \quad \mathbf{U}_1^\top \mathbf{G}_1(\tau) \mathbf{P}_{U_1}^\perp (\mathbf{a}^\top, \mathbf{0}_{1 \times T})^\top \\
& \quad + (\mathbf{a}^\top, \mathbf{0}_{1 \times T}) \mathbf{P}_{U_1}^\perp \mathbf{G}_1(\tau) \mathbf{U}_1 [\mathbf{D}_1^{-1} + \mathbf{U}_1^\top \mathbf{G}_1(\tau) \mathbf{U}_1]^{-1} \mathbf{U}_1^\top \mathbf{G}_1(\tau) \tilde{\boldsymbol{\Omega}} \mathbf{G}_1(\tau) \mathbf{U}_1 \\
& \quad [\mathbf{D}_1^{-1} + \mathbf{U}_1^\top \mathbf{G}_1(\tau) \mathbf{U}_1]^{-1} \mathbf{U}_1^\top \mathbf{G}_1(\tau) \mathbf{P}_{U_1}^\perp (\mathbf{a}^\top, \mathbf{0}_{1 \times T})^\top.
\end{aligned}$$

Since  $\|(\mathbf{a}^\top, \mathbf{0}_{1 \times T}) \mathbf{P}_{U_1}^\perp\| = O(1)$  and

$$\|(\mathbf{a}^\top, \mathbf{0}_{1 \times T}) \mathbf{P}_{U_1}^\perp \mathbf{G}_1(\tau) \mathbf{U}_1 [\mathbf{D}_1^{-1} + \mathbf{U}_1^\top \mathbf{G}_1(\tau) \mathbf{U}_1]^{-1} \mathbf{U}_1^\top\| = O(1),$$

(S.4.7) implies that the terms about  $\mathbf{M}_{12}$ ,  $\mathbf{M}_{21}$  and  $\mathbf{M}_{22}$  are  $o(\tau^{-2}\|\mathbf{P}_V^\perp \mathbf{a}\|^2)$ .

$$\begin{aligned}
& (\mathbf{a}^\top, \mathbf{0}_{1 \times T}) \mathbf{P}_{U_1}^\perp \mathbf{G}_1(\tau) \tilde{\Omega} \mathbf{G}_1(\tau) \mathbf{P}_{U_1}^\perp (\mathbf{a}^\top, \mathbf{0}_{1 \times T})^\top \\
= & (\mathbf{a}^\top \mathbf{P}_V^\perp \Omega^{-1/2}, \mathbf{0}_T) \begin{pmatrix} \mathbf{M}_{11} & \mathbf{M}_{12} \\ \mathbf{M}_{21} & \mathbf{M}_{22} \end{pmatrix} \begin{pmatrix} \Omega^{-1/2} \mathbf{P}_V^\perp \mathbf{a} \\ \mathbf{0}_T \end{pmatrix} \\
= & \mathbf{a}^\top \mathbf{P}_V^\perp \Omega^{-1/2} \mathbf{M}_{11} \Omega^{-1/2} \mathbf{P}_V^\perp \mathbf{a}
\end{aligned}$$

$$\begin{aligned}
& (\mathbf{a}^\top, \mathbf{0}_{1 \times T}) \mathbf{P}_{U_1}^\perp \mathbf{G}_1(\tau) \tilde{\Omega} \mathbf{G}_1(\tau) \mathbf{U}_1 [\mathbf{D}_1^{-1} + \mathbf{U}_1^\top \mathbf{G}_1(\tau) \mathbf{U}_1]^{-1} \mathbf{U}_1^\top \mathbf{G}_1(\tau) \mathbf{P}_{U_1}^\perp (\mathbf{a}^\top, \mathbf{0}_{1 \times T})^\top \\
= & [1 + o_p(1)] \left( \mathbf{a}^\top \mathbf{P}_V^\perp \Omega^{-1/2} \mathbf{M}_{11} \Omega^{-1/2} \mathbf{V}, \mathbf{0} \right) \\
& \begin{pmatrix} \tau^{-1} \mathbf{V}^\top [\mathbf{I}_N + m(-\tau) \Omega]^{-1} \mathbf{V} & \mathbf{0} \\ \mathbf{0} & -\tau m(-\tau) \mathbf{I}_r \end{pmatrix}^{-1} \begin{pmatrix} \mathbf{V}^\top \tau^{-1} [\mathbf{I}_N + m(-\tau) \Omega]^{-1} \mathbf{P}_V^\perp \mathbf{a} \\ \mathbf{0} \end{pmatrix} \\
& + o(\tau^{-2} \|\mathbf{P}_V^\perp \mathbf{a}\|^2) \\
= & \mathbf{a}^\top \mathbf{P}_V^\perp \Omega^{-1/2} \mathbf{M}_{11} \Omega^{-1/2} \mathbf{V} \{ \mathbf{V}^\top [\mathbf{I}_N + m(-\tau) \Omega]^{-1} \mathbf{V} \}^{-1} \mathbf{V}^\top \\
& [\mathbf{I}_N + m(-\tau) \Omega]^{-1} \mathbf{P}_V^\perp \mathbf{a} [1 + o_p(1)].
\end{aligned}$$

$$\begin{aligned}
& \mathbf{U}_1^\top \mathbf{G}_1(\tau) \tilde{\Omega} \mathbf{G}_1(\tau) \mathbf{U}_1 \\
= & \begin{pmatrix} \mathbf{V}^\top \Omega^{-1/2} & \mathbf{0} \\ \mathbf{0} & \mathbf{V}_1^\top \end{pmatrix} \begin{pmatrix} \mathbf{M}_{11} & \mathbf{M}_{12} \\ \mathbf{M}_{21} & \mathbf{M}_{22} \end{pmatrix} \begin{pmatrix} \Omega^{-1/2} \mathbf{V} & \mathbf{0}_{N \times r} \\ \mathbf{0}_{T \times r} & \mathbf{V}_1 \end{pmatrix} \\
= & \begin{pmatrix} \mathbf{V}^\top \Omega^{-1/2} \mathbf{M}_{11} \Omega^{-1/2} \mathbf{V} & \mathbf{V}^\top \Omega^{-1/2} \mathbf{M}_{12} \mathbf{V}_1 \\ \mathbf{V}_1^\top \mathbf{M}_{21} \Omega^{-1/2} \mathbf{V} & \mathbf{V}_1^\top \mathbf{M}_{22} \mathbf{V}_1 \end{pmatrix}
\end{aligned}$$

$$\begin{aligned}
& (\mathbf{a}^\top, \mathbf{0}_{1 \times T}) \mathbf{P}_{U_1}^\perp \mathbf{G}_1(\tau) \mathbf{U}_1 [\mathbf{D}_1^{-1} + \mathbf{U}_1^\top \mathbf{G}_1(\tau) \mathbf{U}_1]^{-1} \mathbf{U}_1^\top \mathbf{G}_1(\tau) \tilde{\Omega} \mathbf{G}_1(\tau) \mathbf{U}_1 \\
& [\mathbf{D}_1^{-1} + \mathbf{U}_1^\top \mathbf{G}_1(\tau) \mathbf{U}_1]^{-1} \mathbf{U}_1^\top \mathbf{G}_1(\tau) \mathbf{P}_{U_1}^\perp (\mathbf{a}^\top, \mathbf{0}_{1 \times T})^\top \\
= & \mathbf{a}^\top \mathbf{P}_V^\perp [\mathbf{I}_N + m(-\tau) \Omega]^{-1} \mathbf{V} \{ \mathbf{V}^\top [\mathbf{I}_N + m(-\tau) \Omega]^{-1} \mathbf{V} \}^{-1} \mathbf{V}^\top \Omega^{-1/2} \mathbf{M}_{11} \Omega^{-1/2} \\
& \mathbf{V} \{ \mathbf{V}^\top [\mathbf{I}_N + m(-\tau) \Omega]^{-1} \mathbf{V} \}^{-1} \mathbf{V}^\top [\mathbf{I}_N + m(-\tau) \Omega]^{-1} \mathbf{P}_V^\perp \mathbf{a} [1 + o_p(1)]
\end{aligned}$$

$$\begin{aligned}
& (\mathbf{a}^\top, \mathbf{0}_{1 \times T}) \mathbf{P}_{U_1}^\perp \mathbf{G}_2(\tau) \tilde{\Omega} \mathbf{G}_2(\tau) \mathbf{P}_{U_1}^\perp (\mathbf{a}^\top, \mathbf{0}_{1 \times T})^\top \\
= & (\mathbf{a}^\top, \mathbf{0}_{1 \times T}) \mathbf{P}_{U_1}^\perp \mathbf{G}_1(\tau) \tilde{\Omega} \mathbf{G}_1(\tau) \mathbf{P}_{U_1}^\perp (\mathbf{a}^\top, \mathbf{0}_{1 \times T})^\top \\
- & 2(\mathbf{a}^\top, \mathbf{0}_{1 \times T}) \mathbf{P}_{U_1}^\perp \mathbf{G}_1(\tau) \tilde{\Omega} \mathbf{G}_1(\tau) \mathbf{U}_1 [\mathbf{D}_1^{-1} + \mathbf{U}_1^\top \mathbf{G}_1(\tau) \mathbf{U}_1]^{-1} \\
& \mathbf{U}_1^\top \mathbf{G}_1(\tau) \mathbf{P}_{U_1}^\perp (\mathbf{a}^\top, \mathbf{0}_{1 \times T})^\top \\
& + (\mathbf{a}^\top, \mathbf{0}_{1 \times T}) \mathbf{P}_{U_1}^\perp \mathbf{G}_1(\tau) \mathbf{U}_1 [\mathbf{D}_1^{-1} + \mathbf{U}_1^\top \mathbf{G}_1(\tau) \mathbf{U}_1]^{-1} \mathbf{U}_1^\top \mathbf{G}_1(\tau) \tilde{\Omega} \mathbf{G}_1(\tau) \mathbf{U}_1 \\
& [\mathbf{D}_1^{-1} + \mathbf{U}_1^\top \mathbf{G}_1(\tau) \mathbf{U}_1]^{-1} \mathbf{U}_1^\top \mathbf{G}_1(\tau) \mathbf{P}_{U_1}^\perp (\mathbf{a}^\top, \mathbf{0}_{1 \times T})^\top \\
= & \mathbf{a}^\top \mathbf{P}_V^\perp \left[ \mathbf{I}_N - [\mathbf{I}_N + m(-\tau) \Omega]^{-1} \mathbf{V} \{ \mathbf{V}^\top [\mathbf{I}_N + m(-\tau) \Omega]^{-1} \mathbf{V} \}^{-1} \mathbf{V}^\top \right] \Omega^{-1/2} \mathbf{M}_{11} \Omega^{-1/2} \\
& \left[ \mathbf{I}_N - \mathbf{V} \{ \mathbf{V}^\top [\mathbf{I}_N + m(-\tau) \Omega]^{-1} \mathbf{V} \}^{-1} \mathbf{V}^\top [\mathbf{I}_N + m(-\tau) \Omega]^{-1} \right] \mathbf{P}_V^\perp \mathbf{a} [1 + o_p(1)].
\end{aligned}$$

Thus, (S.4.6) implies that

$$\begin{aligned}
& (\mathbf{a}^\top, \mathbf{0}_{1 \times T}) \mathbf{P}_{U_1}^\perp \mathbf{G}_2(\tau) \tilde{\Omega} \mathbf{G}_2(\tau) \mathbf{P}_{U_1}^\perp (\mathbf{a}^\top, \mathbf{0}_{1 \times T})^\top \\
= & \tau^{-2} c(\tau) \mathbf{a}^\top \mathbf{P}_V^\perp \left[ \mathbf{I}_N - [\mathbf{I}_N + m(-\tau) \Omega]^{-1} \mathbf{V} \{ \mathbf{V}^\top [\mathbf{I}_N + m(-\tau) \Omega]^{-1} \mathbf{V} \}^{-1} \mathbf{V}^\top \right] \\
& \Omega^{1/2} [m(-\tau) \Omega + \mathbf{I}_N]^{-2} \Omega^{1/2} \left[ \mathbf{I}_N - \mathbf{V} \{ \mathbf{V}^\top [\mathbf{I}_N + m(-\tau) \Omega]^{-1} \mathbf{V} \}^{-1} \mathbf{V}^\top [\mathbf{I}_N + m(-\tau) \Omega]^{-1} \right] \\
& \mathbf{P}_V^\perp \mathbf{a} [1 + o_p(1)] \tag{S.4.8}
\end{aligned}$$

Note we rewrite

$$[\mathbf{I}_N - [\mathbf{I}_N + m(-\tau) \Omega]^{-1} \mathbf{V} \{ \mathbf{V}^\top [\mathbf{I}_N + m(-\tau) \Omega]^{-1} \mathbf{V} \}^{-1} \mathbf{V}^\top]$$

by the following equation.

$$\begin{aligned}
& [\mathbf{I}_N + m(-\tau) \Omega]^{1/2} [\mathbf{I}_N - [\mathbf{I}_N + m(-\tau) \Omega]^{-1} \mathbf{V} \{ \mathbf{V}^\top [\mathbf{I}_N + m(-\tau) \Omega]^{-1} \mathbf{V} \}^{-1} \mathbf{V}^\top] \\
= & \left[ \mathbf{I}_N - [\mathbf{I}_N + m(-\tau) \Omega]^{-1/2} \mathbf{V} \{ \mathbf{V}^\top [\mathbf{I}_N + m(-\tau) \Omega]^{-1} \mathbf{V} \}^{-1} \mathbf{V}^\top [\mathbf{I}_N + m(-\tau) \Omega]^{-1/2} \right] \\
& [\mathbf{I}_N + m(-\tau) \Omega]^{1/2} \\
= & [\mathbf{I}_N - \mathbf{P}_{[\mathbf{I}_N + m(-\tau) \Omega]^{-1/2} \mathbf{V}}] [\mathbf{I}_N + m(-\tau) \Omega]^{1/2}
\end{aligned}$$

where

$$\begin{aligned} & \mathbf{P}_{[\mathbf{I}_N + m(-\tau)\boldsymbol{\Omega}]^{-1/2}\mathbf{V}} \\ = & [\mathbf{I}_N + m(-\tau)\boldsymbol{\Omega}]^{-1/2}\mathbf{V}\{\mathbf{V}^\top[\mathbf{I}_N + m(-\tau)\boldsymbol{\Omega}]^{-1}\mathbf{V}\}^{-1}\mathbf{V}^\top[\mathbf{I}_N + m(-\tau)\boldsymbol{\Omega}]^{-1/2} \end{aligned}$$

is the projection matrix of  $[\mathbf{I}_N + m(-\tau)\boldsymbol{\Omega}]^{-1/2}\mathbf{V}$ .

Thus,

$$\begin{aligned} & (\mathbf{a}^\top, \mathbf{0}_{1 \times T})\mathbf{P}_{U_1}^\perp \mathbf{G}_2(\tau)\tilde{\boldsymbol{\Omega}}\mathbf{G}_2(\tau)\mathbf{P}_{U_1}^\perp (\mathbf{a}^\top, \mathbf{0}_{1 \times T})^\top \\ = & \tau^{-2}c(\tau)\mathbf{a}^\top \mathbf{P}_V^\perp [\mathbf{I}_N + m(-\tau)\boldsymbol{\Omega}]^{-1/2}[\mathbf{I}_N - \mathbf{P}_{[\mathbf{I}_N + m(-\tau)\boldsymbol{\Omega}]^{-1/2}\mathbf{V}}] \\ & [\mathbf{I}_N + m(-\tau)\boldsymbol{\Omega}]^{1/2}\boldsymbol{\Omega}^{1/2}[m(-\tau)\boldsymbol{\Omega} + \mathbf{I}_N]^{-2}\boldsymbol{\Omega}^{1/2}[\mathbf{I}_N + m(-\tau)\boldsymbol{\Omega}]^{1/2} \\ & [\mathbf{I}_N - \mathbf{P}_{[\mathbf{I}_N + m(-\tau)\boldsymbol{\Omega}]^{-1/2}\mathbf{V}}][\mathbf{I}_N + m(-\tau)\boldsymbol{\Omega}]^{-1/2}\mathbf{P}_V^\perp \mathbf{a}[1 + o_p(1)] \\ \asymp & \tau^{-2}\|\mathbf{P}_V^\perp \mathbf{a}\| \end{aligned}$$

in probability. Note that

$$[\mathbf{I}_N - \mathbf{P}_{[\mathbf{I}_N + m(-\tau)\boldsymbol{\Omega}]^{-1/2}\mathbf{V}}][\mathbf{I}_N + m(-\tau)\boldsymbol{\Omega}]^{-1/2}\mathbf{V}\mathbf{V}^\top = \mathbf{0}.$$

Thus,

$$\begin{aligned} & (\mathbf{a}^\top, \mathbf{0}_{1 \times T})\mathbf{P}_{U_1}^\perp \mathbf{G}_2(\tau)\tilde{\boldsymbol{\Omega}}\mathbf{G}_2(\tau)\mathbf{P}_{U_1}^\perp (\mathbf{a}^\top, \mathbf{0}_{1 \times T})^\top \\ = & \tau^{-2}c(\tau)\mathbf{a}^\top [\mathbf{I}_N + m(-\tau)\boldsymbol{\Omega}]^{-1/2}[\mathbf{I}_N - \mathbf{P}_{[\mathbf{I}_N + m(-\tau)\boldsymbol{\Omega}]^{-1/2}\mathbf{V}}] \\ & [\mathbf{I}_N + m(-\tau)\boldsymbol{\Omega}]^{1/2}\boldsymbol{\Omega}^{1/2}[m(-\tau)\boldsymbol{\Omega} + \mathbf{I}_N]^{-2}\boldsymbol{\Omega}^{1/2}[\mathbf{I}_N + m(-\tau)\boldsymbol{\Omega}]^{1/2} \\ & [\mathbf{I}_N - \mathbf{P}_{[\mathbf{I}_N + m(-\tau)\boldsymbol{\Omega}]^{-1/2}\mathbf{V}}][\mathbf{I}_N + m(-\tau)\boldsymbol{\Omega}]^{-1/2}\mathbf{a}[1 + o_p(1)]. \end{aligned}$$

Note that  $[\mathbf{I}_N + m(-\tau)\boldsymbol{\Omega}]^{1/2}\boldsymbol{\Omega}^{1/2} = \boldsymbol{\Omega}^{1/2}[\mathbf{I}_N + m(-\tau)\boldsymbol{\Omega}]^{1/2}$  due to  $\boldsymbol{\Omega}^{1/2}$  is a symmetric matrix. Then

$$\begin{aligned}
& (\mathbf{a}^\top, \mathbf{0}_{1 \times T}) \mathbf{P}_{U_1}^\perp \mathbf{G}_2(\tau) \tilde{\boldsymbol{\Omega}} \mathbf{G}_2(\tau) \mathbf{P}_{U_1}^\perp (\mathbf{a}^\top, \mathbf{0}_{1 \times T})^\top \tag{S.4.9} \\
= & \tau^{-2} c(\tau) a^\top [\mathbf{I}_N + m(-\tau) \boldsymbol{\Omega}]^{-1/2} [\mathbf{I}_N - \mathbf{P}_{[\mathbf{I}_N + m(-\tau) \boldsymbol{\Omega}]^{-1/2} \mathbf{V}}] \\
& \boldsymbol{\Omega}^{1/2} [m(-\tau) \boldsymbol{\Omega} + \mathbf{I}_N]^{-1} \boldsymbol{\Omega}^{1/2} [\mathbf{I}_N - \mathbf{P}_{[\mathbf{I}_N + m(-\tau) \boldsymbol{\Omega}]^{-1/2} \mathbf{V}}] \\
& [\mathbf{I}_N + m(-\tau) \boldsymbol{\Omega}]^{-1/2} \mathbf{a} [1 + o_p(1)] \\
\asymp & \tau^{-2} \|\mathbf{P}_V^\perp \mathbf{a}\|
\end{aligned}$$

in probability.

#### S.4.2 The other term of $\mathbf{a}^\top \mathbf{S}_\tau^{-1} \boldsymbol{\Sigma} \mathbf{S}_\tau^{-1} \mathbf{a}$

Recall (S.2.16), (S.3.14)-(S.3.15),

$$\begin{aligned}
& (\mathbf{a}^\top, \mathbf{0}_{1 \times T}) \mathbf{U}_1 \mathbf{D}_1^{-1} [\mathbf{D}_1^{-1} + \mathbf{U}_1^\top \mathbf{G}_1(\tau) \mathbf{U}_1]^{-1} \mathbf{U}_1^\top \mathbf{G}_1(\tau) \tilde{\boldsymbol{\Omega}} \mathbf{G}_2(\tau) \mathbf{P}_{U_1}^\perp (\mathbf{a}^\top, \mathbf{0}_{1 \times T})^\top \\
= & O_p(\tau^{-1} \|\mathbf{D}_1^{-1}\| \|\mathbf{P}_V^\perp \mathbf{a}\|) = o_p(\tau^{-2} \|\mathbf{P}_V^\perp \mathbf{a}\|^2).
\end{aligned}$$

$$\begin{aligned}
& (\mathbf{a}^\top, \mathbf{0}_{1 \times T}) \mathbf{U}_1 \mathbf{D}_1^{-1} [\mathbf{D}_1^{-1} + \mathbf{U}_1^\top \mathbf{G}_1(\tau) \mathbf{U}_1]^{-1} \mathbf{U}_1^\top \mathbf{G}_1(\tau) \tilde{\boldsymbol{\Omega}} \mathbf{G}_1(\tau) \mathbf{U}_1 \\
& [\mathbf{D}_1^{-1} + \mathbf{U}_1^\top \mathbf{G}_1(\tau) \mathbf{U}_1]^{-1} \mathbf{D}_1^{-1} \mathbf{U}_1^\top (\mathbf{a}^\top, \mathbf{0}_{1 \times T})^\top \\
= & O_p(\|\mathbf{D}_1^{-1}\|^2) = o_p(\tau^{-2} \|\mathbf{P}_V^\perp \mathbf{a}\|^2).
\end{aligned}$$

Thus, in this subsection we focus on

$$\begin{aligned}
& (\mathbf{a}^\top, \mathbf{0}_{1 \times T}) \mathbf{G}_2(\tau) \begin{pmatrix} \mathbf{B}\mathbf{B}^\top & \mathbf{0} \\ \mathbf{0}^\top & \mathbf{0} \end{pmatrix} \mathbf{G}_2(\tau) (\mathbf{a}^\top, \mathbf{0}_{1 \times T})^\top \\
= & (\mathbf{a}^\top, \mathbf{0}_{1 \times T}) \mathbf{P}_{U_1}^\perp \mathbf{G}_2(\tau) \mathbf{U}_1 \begin{pmatrix} \mathbf{B}_1 \mathbf{B}_1^\top & \mathbf{0} \\ \mathbf{0}^\top & \mathbf{0} \end{pmatrix} \mathbf{U}_1^\top \mathbf{G}_2(\tau) \mathbf{P}_{U_1}^\perp (\mathbf{a}^\top, \mathbf{0}_{1 \times T})^\top \\
& + 2(\mathbf{a}^\top, \mathbf{0}_{1 \times T}) \mathbf{P}_{U_1}^\perp \mathbf{G}_2(\tau) \mathbf{U}_1 \begin{pmatrix} \mathbf{B}_1 \mathbf{B}_1^\top & \mathbf{0} \\ \mathbf{0}^\top & \mathbf{0} \end{pmatrix} \mathbf{U}_1^\top \mathbf{G}_2(\tau) \mathbf{U}_1 \mathbf{U}_1^\top (\mathbf{a}^\top, \mathbf{0}_{1 \times T})^\top \\
& + (\mathbf{a}^\top, \mathbf{0}_{1 \times T}) \mathbf{U}_1 \mathbf{U}_1^\top \mathbf{G}_2(\tau) \mathbf{U}_1 \begin{pmatrix} \mathbf{B}_1 \mathbf{B}_1^\top & \mathbf{0} \\ \mathbf{0}^\top & \mathbf{0} \end{pmatrix} \mathbf{U}_1^\top \mathbf{G}_2(\tau) \mathbf{U}_1 \mathbf{U}_1^\top (\mathbf{a}^\top, \mathbf{0}_{1 \times T})^\top.
\end{aligned}$$

Recall (S.2.25), (S.3.14) and  $\tau = o(\|\mathbf{P}_V^\perp \mathbf{a}\|)$ .

$$\begin{aligned}
& (\mathbf{a}^\top, \mathbf{0}_{1 \times T}) \mathbf{P}_{U_1}^\perp \mathbf{G}_2(\tau) \mathbf{U}_1 \begin{pmatrix} \mathbf{B}_1 \mathbf{B}_1^\top & \mathbf{0} \\ \mathbf{0}^\top & \mathbf{0} \end{pmatrix} \mathbf{U}_1^\top \mathbf{G}_2(\tau) \mathbf{P}_{U_1}^\perp (\mathbf{a}^\top, \mathbf{0}_{1 \times T})^\top \\
= & O(\|\mathbf{P}_V^\perp \mathbf{a}\|^2 \|\mathbf{B}_1 \mathbf{B}_1^\top\| \|\mathbf{D}_1^{-1} [\mathbf{D}_1^{-1} + \mathbf{U}_1^\top \mathbf{G}_1(\tau) \mathbf{U}_1]^{-1} \mathbf{U}_1^\top \mathbf{G}_1(\tau)\|^2) \\
= & O_p(\|\mathbf{P}_V^\perp \mathbf{a}\|^2 \|\mathbf{B}_1 \mathbf{B}_1^\top\| \|\mathbf{D}_1^{-1}\|^2) \\
= & O_p(\|\mathbf{P}_V^\perp \mathbf{a}\|^2) = o_p(\tau^{-2} \|\mathbf{P}_V^\perp \mathbf{a}\|^2).
\end{aligned}$$

$$\begin{aligned}
& (\mathbf{a}^\top, \mathbf{0}_{1 \times T}) \mathbf{P}_{U_1}^\perp \mathbf{G}_2(\tau) \mathbf{U}_1 \begin{pmatrix} \mathbf{B}_1 \mathbf{B}_1^\top & \mathbf{0} \\ \mathbf{0}^\top & \mathbf{0} \end{pmatrix} \mathbf{U}_1^\top \mathbf{G}_2(\tau) \mathbf{U}_1 \mathbf{U}_1^\top (\mathbf{a}^\top, \mathbf{0}_{1 \times T})^\top \\
= & O(\|\mathbf{P}_V^\perp \mathbf{a}\| \|\mathbf{B}_1 \mathbf{B}_1^\top\| \|\mathbf{D}_1^{-1} [\mathbf{D}_1^{-1} + \mathbf{U}_1^\top \mathbf{G}_1(\tau) \mathbf{U}_1]^{-1} \mathbf{U}_1^\top \mathbf{G}_1(\tau)\|^2) \\
= & O_p(\|\mathbf{P}_V^\perp \mathbf{a}\| \|\mathbf{B}_1 \mathbf{B}_1^\top\| \|\mathbf{D}_1^{-1}\|^2) \\
= & O_p(\|\mathbf{P}_V^\perp \mathbf{a}\|) = o_p(\tau^{-2} \|\mathbf{P}_V^\perp \mathbf{a}\|^2).
\end{aligned}$$

$$\begin{aligned}
& (\mathbf{a}^\top, \mathbf{0}_{1 \times T}) \mathbf{U}_1 \mathbf{U}_1^\top \mathbf{G}_2(\tau) \mathbf{U}_1 \begin{pmatrix} \mathbf{B}_1 \mathbf{B}_1^\top & \mathbf{0} \\ \mathbf{0}^\top & \mathbf{0} \end{pmatrix} \mathbf{U}_1^\top \mathbf{G}_2(\tau) \mathbf{U}_1 \mathbf{U}_1^\top (\mathbf{a}^\top, \mathbf{0}_{1 \times T})^\top \\
= & O(\|\mathbf{B}_1 \mathbf{B}_1^\top\| \|\mathbf{D}_1^{-1} [\mathbf{D}_1^{-1} + \mathbf{U}_1^\top \mathbf{G}_1(\tau) \mathbf{U}_1]^{-1} \mathbf{U}_1^\top \mathbf{G}_1(\tau)\|^2) \\
= & O_p(\|\mathbf{B}_1 \mathbf{B}_1^\top\| \|\mathbf{D}_1^{-1}\|^2) \\
= & O_p(1) = o_p(\tau^{-2} \|\mathbf{P}_V^\perp \mathbf{a}\|^2).
\end{aligned}$$

Thus,

$$(\mathbf{a}^\top, \mathbf{0}_{1 \times T}) \mathbf{G}_2(\tau) \begin{pmatrix} \mathbf{B}\mathbf{B}^\top & \mathbf{0} \\ \mathbf{0}^\top & \mathbf{0} \end{pmatrix} \mathbf{G}_2(\tau) (\mathbf{a}^\top, \mathbf{0}_{1 \times T})^\top = o_p(\tau^{-2} \|\mathbf{P}_V^\perp \mathbf{a}\|^2).$$

These and (S.4.9) imply that

$$\begin{aligned} & \mathbf{a}^\top \mathbf{S}_\tau^{-1} \Sigma \mathbf{S}_\tau^{-1} \mathbf{a} \\ = & \tau^{-2} c(\tau) \mathbf{a}^\top \mathbf{P}_V^\perp [\mathbf{I}_N + m(-\tau) \Omega]^{-1/2} [\mathbf{I}_N - \mathbf{P}_{[\mathbf{I}_N + m(-\tau) \Omega]^{-1/2} \mathbf{V}}] \\ & \Omega^{1/2} [m(-\tau) \Omega + \mathbf{I}_N]^{-1} \Omega^{1/2} [\mathbf{I}_N - \mathbf{P}_{[\mathbf{I}_N + m(-\tau) \Omega]^{-1/2} \mathbf{V}}] \\ & [\mathbf{I}_N + m(-\tau) \Omega]^{-1/2} \mathbf{P}_V^\perp \mathbf{a} [1 + o_p(1)]. \end{aligned}$$

Note that

$$\left[ \mathbf{I}_N - \mathbf{P}_{[\mathbf{I}_N + m(-\tau) \Omega]^{-1/2} \mathbf{V}} \right] [\mathbf{I}_N + m(-\tau) \Omega]^{-1/2} \mathbf{V} \mathbf{V}^\top = \mathbf{0}.$$

Then

$$\begin{aligned} & \left[ \mathbf{I}_N - \mathbf{P}_{[\mathbf{I}_N + m(-\tau) \Omega]^{-1/2} \mathbf{V}} \right] [\mathbf{I}_N + m(-\tau) \Omega]^{-1/2} \mathbf{P}_V^\perp \mathbf{a} \\ = & \left[ \mathbf{I}_N - \mathbf{P}_{[\mathbf{I}_N + m(-\tau) \Omega]^{-1/2} \mathbf{V}} \right] [\mathbf{I}_N + m(-\tau) \Omega]^{-1/2} \mathbf{a}. \end{aligned}$$

Recall (S.2.20) and (S.1.5),

$$\begin{aligned} & \mathbf{a}^\top \mathbf{S}_\tau^{-1} \Sigma \mathbf{S}_\tau^{-1} \mathbf{a} \\ = & \tau^{-2} c(\tau) \tilde{\mathbf{a}}_\tau^\top \Omega^{1/2} [m(-\tau) \Omega + \mathbf{I}_N]^{-1} \Omega^{1/2} \tilde{\mathbf{a}}_\tau [1 + o_p(1)]. \end{aligned} \quad (\text{S.4.10})$$

Recall (S.1.3)-(S.1.4),

$$\begin{aligned} & \mathbf{1}^\top \mathbf{S}_\tau^{-1} \Sigma \mathbf{S}_\tau^{-1} \mathbf{1} \\ = & \tau^{-2} c(\tau) \tilde{\mathbf{1}}_\tau^\top \Omega^{1/2} [m(-\tau) \Omega + \mathbf{I}_N]^{-1} \Omega^{1/2} \tilde{\mathbf{1}}_\tau [1 + o_p(1)] \\ = & \tau^{-2} c(\tau) \check{\mathbf{1}}_\tau^\top \check{\mathbf{1}}_\tau [1 + o_p(1)]. \end{aligned} \quad (\text{S.4.11})$$

From (S.3.16) and (S.4.11), we can prove (S.1.7).

We note that  $m(-\tau) \asymp N^{-1}T$ , thus when  $N \gg T$ ,

$$\begin{aligned} & \mathbf{a}^\top \mathbf{S}_\tau^{-1} \boldsymbol{\Sigma} \mathbf{S}_\tau^{-1} \mathbf{a} \\ = & \tau^{-2} \mathbf{a}^\top \mathbf{P}_V^\perp \boldsymbol{\Omega} \mathbf{P}_V^\perp \mathbf{a} [1 + O(TN^{-1})][1 + o_p(1)]. \end{aligned} \quad (\text{S.4.12})$$

From (S.3.19) and (S.4.12), we prove (S.1.10).

## S.5 The case $N/T \rightarrow \gamma \in (0, 1)$ and (S.1.11)-(S.1.12)

In this section, we prove (S.1.11). Recall (S.2.4),

$$\mathbb{V}(\hat{\boldsymbol{\omega}}) = \frac{\mathbf{1}^\top \mathbf{S}_0^{-1} \boldsymbol{\Sigma} \mathbf{S}_0^{-1} \mathbf{1}}{[\mathbf{1}^\top \mathbf{S}_0^{-1} \mathbf{1}]^2}.$$

When  $T > N$ ,  $\mathbf{S}_0 = T^{-1} \mathbf{R} \mathbf{R}^\top$  is invertible in probability.

Recall (S.2.15) and  $\tau = 0$ , we need to study two terms

$$(\mathbf{a}^\top, \mathbf{0}_{1 \times T}) \mathbf{P}_{U_1}^\perp \mathbf{G}_1(0) \mathbf{P}_{U_1}^\perp (\mathbf{a}^\top, \mathbf{0}_{1 \times T})^\top$$

and

$$(\mathbf{a}^\top, \mathbf{0}_{1 \times T}) \mathbf{P}_{U_1}^\perp \mathbf{G}_1(0) \mathbf{U}_1 \left[ \mathbf{D}_1^{-1} + \mathbf{U}_1^\top \mathbf{G}_1(0) \mathbf{U}_1 \right]^{-1} \mathbf{U}_1^\top \mathbf{G}_1(0) \mathbf{P}_{U_1}^\perp (\mathbf{a}^\top, \mathbf{0}_{1 \times T})^\top.$$

To study  $\mathbf{G}_1(0)$ , we recall (S.3.2) and  $\tau = 0$ ,

$$\begin{aligned} & \begin{pmatrix} \boldsymbol{\Omega}^{1/2} & \mathbf{0} \\ \mathbf{0} & \mathbf{I}_T \end{pmatrix} \mathbf{G}_1(0) \begin{pmatrix} \boldsymbol{\Omega}^{1/2} & \mathbf{0} \\ \mathbf{0} & \mathbf{I}_T \end{pmatrix} \\ = & \begin{pmatrix} (T^{-1} \mathbf{Z} \mathbf{Z}^\top)^{-1} & T^{-1/2} (T^{-1} \mathbf{Z} \mathbf{Z}^\top)^{-1} \mathbf{Z} \\ T^{-1/2} \mathbf{Z}^\top (T^{-1} \mathbf{Z} \mathbf{Z}^\top)^{-1} & -\mathbf{I}_T + T^{-1} \mathbf{Z}^\top (T^{-1} \mathbf{Z} \mathbf{Z}^\top)^{-1} \mathbf{Z} \end{pmatrix}. \end{aligned} \quad (\text{S.5.1})$$

Rewrite the SVD of  $T^{-1/2} \mathbf{Z}$  as  $T^{-1/2} \mathbf{Z} = \mathbf{W}_1 \mathbf{L} \mathbf{W}_2$ . Then  $\|\mathbf{L}^{-1}\| \asymp \|\mathbf{L}^{-1}\|_{\min} = 1$  due to  $\gamma < 1$ . From Bai, Miao, and Pan (2007),  $\mathbf{W}_1$  and  $\mathbf{W}_2$  are asymptotically Haar distributed.

Then for any  $N$ –dimensional unit-vector  $\mathbf{b}$  and  $T$ –dimensional unit-vector  $\mathbf{c}$ ,

$$\|\mathbf{b}^\top \mathbf{W}_1 \mathbf{L} \mathbf{W}_2 \mathbf{c}\| = \|T^{-1/2} \mathbf{b}^\top \mathbf{Z} \mathbf{c}\| = O_p(T^{-1/2}).$$

$$\begin{aligned} & \mathbf{b}^\top (T^{-1} \mathbf{Z} \mathbf{Z}^\top)^{-1} \mathbf{b} \\ = & \mathbf{b}^\top \mathbf{W}_1 \mathbf{L}^{-2} \mathbf{W}_1^\top \mathbf{b} \\ = & N^{-1} \text{tr}(\mathbf{L}^{-2}) [1 + o_p(1)] \\ = & N^{-1} \text{tr}[(T^{-1} \mathbf{Z} \mathbf{Z}^\top)^{-1}] [1 + o_p(1)] \\ = & (T - N)^{-1} T [1 + o_p(1)]. \end{aligned}$$

The last equation is from (S.10.4).

$$\|T^{-1/2} \mathbf{b}^\top (T^{-1} \mathbf{Z} \mathbf{Z}^\top)^{-1} \mathbf{Z} \mathbf{c}\| = \|\mathbf{b}^\top \mathbf{W}_1 \mathbf{L}^{-1} \mathbf{W}_2 \mathbf{c}\| = O_p(T^{-1/2}).$$

$$\begin{aligned} & \mathbf{c}^\top T^{-1} \mathbf{Z}^\top (T^{-1} \mathbf{Z} \mathbf{Z}^\top)^{-1} \mathbf{Z} \mathbf{c} \\ = & \mathbf{c}^\top \mathbf{W}_2^\top \mathbf{W}_2 \mathbf{c} \\ = & T^{-1} N [1 + o_p(1)]. \end{aligned}$$

Thus,

$$\begin{aligned} & (\mathbf{a}^\top, \mathbf{0}_{1 \times T}) \mathbf{P}_{\tilde{U}_1}^\perp \mathbf{G}_1(0) \mathbf{P}_{\tilde{U}_1}^\perp (\mathbf{a}^\top, \mathbf{0}_{1 \times T})^\top \\ = & \mathbf{a}^\top \mathbf{P}_V^\perp \boldsymbol{\Omega}^{-1/2} (T^{-1} \mathbf{Z} \mathbf{Z}^\top)^{-1} \boldsymbol{\Omega}^{-1/2} \mathbf{a} [1 + o_p(1)] \\ = & (T - N)^{-1} T \mathbf{a}^\top \mathbf{P}_V^\perp \boldsymbol{\Omega}^{-1} \mathbf{P}_V^\perp \mathbf{a} [1 + o_p(1)]. \end{aligned} \tag{S.5.2}$$

Now we consider the term

$$(\mathbf{a}^\top, \mathbf{0}_{1 \times T}) \mathbf{P}_{\tilde{U}_1}^\perp \mathbf{G}_1(0) \mathbf{U}_1 \left[ \mathbf{D}_1^{-1} + \mathbf{U}_1^\top \mathbf{G}_1(0) \mathbf{U}_1 \right]^{-1} \mathbf{U}_1^\top \mathbf{G}_1(0) \mathbf{P}_{\tilde{U}_1}^\perp (\mathbf{a}^\top, \mathbf{0}_{1 \times T})^\top.$$

$$\begin{aligned}
& (\mathbf{a}^\top, \mathbf{0}_{1 \times T}) \mathbf{P}_{U_1}^\perp \mathbf{G}_1(0) \mathbf{U}_1 \\
= & (\mathbf{a}^\top, \mathbf{0}_{1 \times T}) \begin{pmatrix} \mathbf{I}_N - \mathbf{V} \mathbf{V}^\top & \mathbf{0} \\ \mathbf{0} & \mathbf{I}_T - \mathbf{V}_1 \mathbf{V}_1^\top \end{pmatrix} \begin{pmatrix} (T - N)^{-1} T \boldsymbol{\Omega}^{-1} & 0 \\ 0 & -T^{-1}(T - N) \mathbf{I}_T \end{pmatrix} \\
& \begin{pmatrix} \mathbf{V} & \mathbf{0} \\ \mathbf{0} & \mathbf{V}_1 \end{pmatrix} [1 + o_p(1)] \\
= & ((T - N)^{-1} T \mathbf{a}^\top \mathbf{P}_V^\perp \boldsymbol{\Omega}^{-1} \mathbf{V}, \mathbf{0}_r) [1 + o_p(1)]
\end{aligned}$$

$$\begin{aligned}
& (\mathbf{a}^\top, \mathbf{0}_{1 \times T}) \mathbf{P}_{U_1}^\perp \mathbf{G}_1(0) \mathbf{U}_1 \left[ \mathbf{D}_1^{-1} + \mathbf{U}_1^\top \mathbf{G}_1(0) \mathbf{U}_1 \right]^{-1} \mathbf{U}_1^\top \mathbf{G}_1(0) \mathbf{P}_{U_1}^\perp (\mathbf{a}^\top, \mathbf{0}_{1 \times T})^\top \\
= & (\mathbf{a}^\top \mathbf{P}_V^\perp [T^{-1}(T - N) \boldsymbol{\Omega}]^{-1} \mathbf{V}, \mathbf{0}_r) \\
& \begin{pmatrix} \mathbf{V}^\top [T^{-1}(T - N) \boldsymbol{\Omega}]^{-1} \mathbf{V} & \mathbf{0} \\ \mathbf{0} & -T^{-1}(T - N) \mathbf{I}_r \end{pmatrix}^{-1} \\
& (\mathbf{a}^\top \mathbf{P}_V^\perp [T^{-1}(T - N) \boldsymbol{\Omega}]^{-1} \mathbf{V}, \mathbf{0}_r)^\top [1 + o_p(1)] \\
= & (T - N)^{-1} T \mathbf{a}^\top \mathbf{P}_V^\perp \boldsymbol{\Omega}^{-1} \mathbf{V} [\mathbf{V}^\top \boldsymbol{\Omega}^{-1} \mathbf{V}]^{-1} \mathbf{V}^\top \boldsymbol{\Omega}^{-1} \mathbf{P}_V^\perp \mathbf{a} [1 + o_p(1)].
\end{aligned}$$

This, together with (S.5.2) and (S.2.5), implies that

$$\begin{aligned}
& \mathbf{a}^\top (T^{-1} \mathbf{R} \mathbf{R}^\top)^{-1} \mathbf{a} \\
= & (T - N)^{-1} T \mathbf{a}^\top \mathbf{P}_V^\perp \boldsymbol{\Omega}^{-1} \mathbf{P}_V^\perp \mathbf{a} [1 + o_p(1)] \\
& -(T - N)^{-1} T \mathbf{a}^\top \mathbf{P}_V^\perp \boldsymbol{\Omega}^{-1} \mathbf{V} [\mathbf{V}^\top \boldsymbol{\Omega}^{-1} \mathbf{V}]^{-1} \mathbf{V}^\top \boldsymbol{\Omega}^{-1} \mathbf{P}_V^\perp \mathbf{a} \\
= & (T - N)^{-1} T \mathbf{a}^\top \mathbf{P}_V^\perp \boldsymbol{\Omega}^{-1/2} \{ \mathbf{I}_N - \boldsymbol{\Omega}^{-1/2} \mathbf{V} [\mathbf{V}^\top \boldsymbol{\Omega}^{-1} \mathbf{V}]^{-1} \mathbf{V}^\top \boldsymbol{\Omega}^{-1/2} \} \\
& \boldsymbol{\Omega}^{-1/2} \mathbf{P}_V^\perp \mathbf{a} [1 + o_p(1)] \\
= & (T - N)^{-1} T \mathbf{a}^\top \boldsymbol{\Sigma}^{-1} \mathbf{a} [1 + o_p(1)].
\end{aligned}$$

$$\mathbf{a}^\top \mathbf{S}_0^{-1} \mathbf{a} = \frac{T}{T - N} \mathbf{a}^\top \boldsymbol{\Sigma}^{-1} \mathbf{a} [1 + o_p(1)] \quad (\text{S.5.3})$$

Recall (S.2.9), (S.2.14) and (S.2.16) with  $\tau = 0$ , we focus on

$$\begin{aligned}
& (\mathbf{a}^\top, \mathbf{0}_{1 \times T}) \mathbf{P}_{U_1}^\perp \mathbf{G}_2(0) \tilde{\Omega} \mathbf{G}_2(0) \mathbf{P}_{U_1}^\perp (\mathbf{a}^\top, \mathbf{0}_{1 \times T})^\top \\
= & (\mathbf{a}^\top, \mathbf{0}_{1 \times T}) \mathbf{P}_{U_1}^\perp \mathbf{G}_1(0) \tilde{\Omega} \mathbf{G}_1(0) \mathbf{P}_{U_1}^\perp (\mathbf{a}^\top, \mathbf{0}_{1 \times T})^\top - \\
& 2(\mathbf{a}^\top, \mathbf{0}_{1 \times T}) \mathbf{P}_{U_1}^\perp \mathbf{G}_1(0) \tilde{\Omega} \mathbf{G}_1(0) \mathbf{U}_1 [\mathbf{D}_1^{-1} + \mathbf{U}_1^\top \mathbf{G}_1(0) \mathbf{U}_1]^{-1} \\
& \mathbf{U}_1^\top \mathbf{G}_1(0) \mathbf{P}_{U_1}^\perp (\mathbf{a}^\top, \mathbf{0}_{1 \times T})^\top \\
& + (\mathbf{a}^\top, \mathbf{0}_{1 \times T}) \mathbf{P}_{U_1}^\perp \mathbf{G}_1(0) \mathbf{U}_1 [\mathbf{D}_1^{-1} + \mathbf{U}_1^\top \mathbf{G}_1(0) \mathbf{U}_1]^{-1} \mathbf{U}_1^\top \mathbf{G}_1(0) \tilde{\Omega} \mathbf{G}_1(0) \mathbf{U}_1 \\
& [\mathbf{D}_1^{-1} + \mathbf{U}_1^\top \mathbf{G}_1(0) \mathbf{U}_1]^{-1} \mathbf{U}_1^\top \mathbf{G}_1(0) \mathbf{P}_{U_1}^\perp (\mathbf{a}^\top, \mathbf{0}_{1 \times T})^\top.
\end{aligned}$$

The other term can be controlled by the same method in Section S.4.2.

$$\begin{aligned}
& \begin{pmatrix} \Omega^{1/2} & \mathbf{0} \\ \mathbf{0} & \mathbf{I}_T \end{pmatrix} \mathbf{G}_1(0) \tilde{\Omega} \mathbf{G}_1(0) \begin{pmatrix} \Omega^{1/2} & \mathbf{0} \\ \mathbf{0} & \mathbf{I}_T \end{pmatrix} \\
= & \begin{pmatrix} \Omega^{1/2} & \mathbf{0} \\ \mathbf{0} & \mathbf{I}_T \end{pmatrix} \begin{pmatrix} \mathbf{0} & T^{-1/2} \mathbf{E} \\ T^{-1/2} \mathbf{E}^\top & -\mathbf{I}_T \end{pmatrix}^{-1} \begin{pmatrix} \Omega & \mathbf{0} \\ \mathbf{0} & \mathbf{0} \end{pmatrix} \begin{pmatrix} \mathbf{0} & T^{-1/2} \mathbf{E} \\ T^{-1/2} \mathbf{E}^\top & -\mathbf{I}_T \end{pmatrix}^{-1} \\
& \begin{pmatrix} \Omega^{1/2} & \mathbf{0} \\ \mathbf{0} & \mathbf{I}_T \end{pmatrix} \\
= & \begin{pmatrix} (T^{-1} \mathbf{Z} \mathbf{Z}^\top)^{-1} & T^{-1/2} (T^{-1} \mathbf{Z} \mathbf{Z}^\top)^{-1} \mathbf{Z} \\ T^{-1/2} \mathbf{Z}^\top (T^{-1} \mathbf{Z} \mathbf{Z}^\top)^{-1} & -\mathbf{I}_T + \mathbf{Z}^\top (\mathbf{Z} \mathbf{Z}^\top)^{-1} \mathbf{Z} \end{pmatrix} \begin{pmatrix} \mathbf{I}_N & \mathbf{0} \\ \mathbf{0} & \mathbf{0} \end{pmatrix} \\
& \begin{pmatrix} (T^{-1} \mathbf{Z} \mathbf{Z}^\top)^{-1} & T^{-1/2} (T^{-1} \mathbf{Z} \mathbf{Z}^\top)^{-1} \mathbf{Z} \\ T^{-1/2} \mathbf{Z}^\top (T^{-1} \mathbf{Z} \mathbf{Z}^\top)^{-1} & -\mathbf{I}_T + \mathbf{Z}^\top (\mathbf{Z} \mathbf{Z}^\top)^{-1} \mathbf{Z} \end{pmatrix} \\
= & \begin{pmatrix} (T^{-1} \mathbf{Z} \mathbf{Z}^\top)^{-2} & T^{-1/2} (T^{-1} \mathbf{Z} \mathbf{Z}^\top)^{-2} \mathbf{Z} \\ T^{-1/2} \mathbf{Z}^\top (T^{-1} \mathbf{Z} \mathbf{Z}^\top)^{-2} & T^{-1} \mathbf{Z}^\top (T^{-1} \mathbf{Z} \mathbf{Z}^\top)^{-2} \mathbf{Z} \end{pmatrix}.
\end{aligned}$$

Then for any  $N$ -dimensional unit-vector  $\mathbf{b}$  and  $T$ -dimensional unit-vector  $\mathbf{c}$ ,

$$\begin{aligned}
& \mathbf{b}^\top (T^{-1} \mathbf{Z} \mathbf{Z}^\top)^{-2} \mathbf{b} \\
= & \mathbf{b}^\top \mathbf{W}_1 \mathbf{L}^{-4} \mathbf{W}_1^\top \mathbf{b} \\
= & N^{-1} \text{tr}(\mathbf{L}^{-4}) [1 + o_p(1)] \\
= & N^{-1} \text{tr}[(T^{-1} \mathbf{Z} \mathbf{Z}^\top)^{-2}] [1 + o_p(1)] \\
= & (T - N)^{-3} T^3 [1 + o_p(1)].
\end{aligned}$$

The last equation is from (S.10.5).

$$\|T^{-1/2} \mathbf{b}^\top (T^{-1} \mathbf{Z} \mathbf{Z}^\top)^{-2} \mathbf{Z} \mathbf{c}\| = \|\mathbf{b}^\top \mathbf{W}_1 \mathbf{L}^{-3} \mathbf{W}_2 \mathbf{c}\| = O_p(T^{-1/2}).$$

$$\begin{aligned}
& \mathbf{c}^\top T^{-1} \mathbf{Z}^\top (T^{-1} \mathbf{Z} \mathbf{Z}^\top)^{-2} \mathbf{Z} \mathbf{c} \\
= & \mathbf{c}^\top \mathbf{W}_2^\top \mathbf{L}^{-2} \mathbf{W}_2 \mathbf{c} \\
= & T^{-1} \text{tr}(\mathbf{L}^{-2}) [1 + O_p(T^{-1/2})] \\
= & T^{-1} \text{tr}[(T^{-1} \mathbf{Z} \mathbf{Z}^\top)^{-1}] [1 + O_p(T^{-1/2})] \\
= & (T - N)^{-1} N [1 + O_p(T^{-1/2})].
\end{aligned}$$

The last equation is from (S.10.4).

For any  $T$ -dimensional unit-vectors  $\mathbf{c}_1$  and  $\mathbf{c}_2$  such that  $\mathbf{c}_1^\top \mathbf{c}_2 = 0$ , we can find that

$$\begin{aligned}
& (T - N)^{-1} N [1 + O_p(T^{-1/2})] \\
= & (\lambda \mathbf{c}_1 + \sqrt{1 - \lambda^2} \mathbf{c}_2)^\top T^{-1} \mathbf{Z}^\top (T^{-1} \mathbf{Z} \mathbf{Z}^\top)^{-2} \mathbf{Z} (\lambda \mathbf{c}_1 + \sqrt{1 - \lambda^2} \mathbf{c}_2) \\
= & \lambda^2 \mathbf{c}_1^\top \mathbf{W}_2^\top \mathbf{L}^{-2} \mathbf{W}_2 \mathbf{c}_1 + (1 - \lambda^2) \mathbf{c}_2^\top \mathbf{W}_2^\top \mathbf{L}^{-2} \mathbf{W}_2 \mathbf{c}_2 \\
& + 2\lambda \sqrt{1 - \lambda^2} \mathbf{c}_1^\top \mathbf{W}_2^\top \mathbf{L}^{-2} \mathbf{W}_2 \mathbf{c}_2 \\
= & (T - N)^{-1} N [1 + O_p(T^{-1/2})] + 2\lambda \sqrt{1 - \lambda^2} \mathbf{c}_1^\top \mathbf{W}_2^\top \mathbf{L}^{-2} \mathbf{W}_2 \mathbf{c}_2
\end{aligned}$$

for any  $\lambda \in (0, 1)$ . Then

$$c_1^\top \mathbf{W}_2^\top \mathbf{L}^{-2} \mathbf{W}_2 \mathbf{c}_2 = O_p(T^{-1/2}).$$

$$\begin{aligned} & \mathbf{U}_1^\top \mathbf{G}_1(0) \tilde{\Omega} \mathbf{G}_1(0) \mathbf{U}_1 \\ = & \begin{pmatrix} \mathbf{V}^\top & \mathbf{0} \\ \mathbf{0} & \mathbf{V}_1^\top \end{pmatrix} \begin{pmatrix} \Omega^{-1/2} & \mathbf{0} \\ \mathbf{0} & \mathbf{I}_T \end{pmatrix} \begin{pmatrix} (T^{-1} \mathbf{Z} \mathbf{Z}^\top)^{-2} & T^{-1/2} (T^{-1} \mathbf{Z} \mathbf{Z}^\top)^{-2} \mathbf{Z} \\ T^{-1/2} \mathbf{Z}^\top (T^{-1} \mathbf{Z} \mathbf{Z}^\top)^{-2} & T^{-1} \mathbf{Z}^\top (T^{-1} \mathbf{Z} \mathbf{Z}^\top)^{-2} \mathbf{Z} \end{pmatrix} \\ & \begin{pmatrix} \Omega^{-1/2} & \mathbf{0} \\ \mathbf{0} & \mathbf{I}_T \end{pmatrix} \begin{pmatrix} \mathbf{V} & \mathbf{0} \\ \mathbf{0} & \mathbf{V}_1 \end{pmatrix} \\ = & \begin{pmatrix} \mathbf{V}^\top \Omega^{-1/2} (T^{-1} \mathbf{Z} \mathbf{Z}^\top)^{-2} \Omega^{-1/2} \mathbf{V} & T^{-1/2} \mathbf{V}^\top \Omega^{-1/2} (T^{-1} \mathbf{Z} \mathbf{Z}^\top)^{-2} \mathbf{Z} \mathbf{V}_1 \\ T^{-1/2} \mathbf{V}_1^\top \mathbf{Z}^\top (T^{-1} \mathbf{Z} \mathbf{Z}^\top)^{-2} \Omega^{-1/2} \mathbf{V} & T^{-1} \mathbf{V}_1^\top \mathbf{Z}^\top (T^{-1} \mathbf{Z} \mathbf{Z}^\top)^{-2} \mathbf{Z} \mathbf{V}_1 \end{pmatrix} \end{aligned}$$

$$\begin{aligned} & (\mathbf{a}^\top, \mathbf{0}_{1 \times T}) \mathbf{P}_{U_1}^\perp \mathbf{G}_1(0) \tilde{\Omega} \mathbf{G}_1(0) \mathbf{P}_{U_1}^\perp (\mathbf{a}^\top, \mathbf{0}_{1 \times T})^\top \\ = & \mathbf{a}^\top \mathbf{P}_V^\perp \Omega^{-1/2} (T^{-1} \mathbf{Z} \mathbf{Z}^\top)^{-2} \Omega^{-1/2} \mathbf{P}_V^\perp \mathbf{a} \\ = & N^{-1} \text{tr}[(T^{-1} \mathbf{Z} \mathbf{Z}^\top)^{-2}] \mathbf{a}^\top \mathbf{P}_V^\perp \Omega^{-1} \mathbf{P}_V^\perp \mathbf{a} [1 + o_p(1)]. \end{aligned}$$

$$\begin{aligned} & (\mathbf{a}^\top, \mathbf{0}_{1 \times T}) \mathbf{P}_{U_1}^\perp \mathbf{G}_1(0) \tilde{\Omega} \mathbf{G}_1(0) \mathbf{U}_1 \\ = & (\mathbf{a}^\top \mathbf{P}_V^\perp \Omega^{-1/2} (T^{-1} \mathbf{Z} \mathbf{Z}^\top)^{-2} \Omega^{-1/2} \mathbf{V}, T^{-1/2} \mathbf{a}^\top \mathbf{P}_V^\perp \Omega^{-1/2} (T^{-1} \mathbf{Z} \mathbf{Z}^\top)^{-2} \mathbf{Z} \mathbf{V}_1) \end{aligned}$$

Then  $\|T^{-1/2} \mathbf{a}^\top \mathbf{P}_V^\perp \Omega^{-1/2} (T^{-1} \mathbf{Z} \mathbf{Z}^\top)^{-2} \mathbf{Z} \mathbf{V}_1\| = O_p(T^{-1/2} \|\mathbf{P}_V^\perp \mathbf{a}\|)$  since  $\mathbf{V}_1$  is  $T \times r$ .

$$\begin{aligned}
& (\mathbf{a}^\top, \mathbf{0}_{1 \times T}) \mathbf{P}_{U_1}^\perp \mathbf{G}_1(0) \tilde{\Omega} \mathbf{G}_1(0) \mathbf{U}_1 [\mathbf{D}_1^{-1} + \mathbf{U}_1^\top \mathbf{G}_1(\tau) \mathbf{U}_1]^{-1} \mathbf{U}_1^\top \mathbf{G}_1(0) \mathbf{P}_{U_1}^\perp (\mathbf{a}^\top, \mathbf{0}_{1 \times T})^\top \\
= & (\mathbf{a}^\top \mathbf{P}_V^\perp \Omega^{-1/2} (T^{-1} \mathbf{Z} \mathbf{Z}^\top)^{-2} \Omega^{-1/2} \mathbf{V}, \mathbf{0}_r) \\
& \left( \begin{array}{cc} \mathbf{V}^\top [T^{-1} (T - N) \Omega]^{-1} \mathbf{V} & \mathbf{0} \\ \mathbf{0} & -T^{-1} (T - N) \mathbf{I}_r \end{array} \right)^{-1} \\
& ((T - N)^{-1} T \mathbf{a}^\top \mathbf{P}_V^\perp \Omega^{-1} \mathbf{V}, \mathbf{0}_r)^\top [1 + o_p(1)] + o_p(\|\mathbf{P}_V^\perp \mathbf{a}\|^2) \\
= & \mathbf{a}^\top \mathbf{P}_V^\perp \Omega^{-1/2} (T^{-1} \mathbf{Z} \mathbf{Z}^\top)^{-2} \Omega^{-1/2} \mathbf{V} [\mathbf{V}^\top \Omega^{-1} \mathbf{V}]^{-1} \mathbf{V}^\top \Omega^{-1} \mathbf{P}_V^\perp \mathbf{a} [1 + o_p(1)] \\
& + o_p(\|\mathbf{P}_V^\perp \mathbf{a}\|^2) \\
= & N^{-1} \text{tr}[(T^{-1} \mathbf{Z} \mathbf{Z}^\top)^{-2}] \mathbf{a}^\top \mathbf{P}_V^\perp \Omega^{-1} \mathbf{V} [\mathbf{V}^\top \Omega^{-1} \mathbf{V}]^{-1} \mathbf{V}^\top \Omega^{-1} \mathbf{P}_V^\perp \mathbf{a} [1 + o_p(1)] \\
= & N^{-1} \text{tr}[(T^{-1} \mathbf{Z} \mathbf{Z}^\top)^{-2}] \mathbf{a}^\top \mathbf{P}_V^\perp \Omega^{-1/2} \mathbf{P}_{\Omega^{-1/2} \mathbf{V}}^\perp \Omega^{-1/2} \mathbf{P}_V^\perp \mathbf{a} [1 + o_p(1)]
\end{aligned}$$

$$\begin{aligned}
& (\mathbf{a}^\top, \mathbf{0}_{1 \times T}) \mathbf{P}_{U_1}^\perp \mathbf{G}_1(0) \mathbf{U}_1 [\mathbf{D}_1^{-1} + \mathbf{U}_1^\top \mathbf{G}_1(0) \mathbf{U}_1]^{-1} \mathbf{U}_1^\top \mathbf{G}_1(0) \tilde{\Omega} \mathbf{G}_1(0) \mathbf{U}_1 \\
& [\mathbf{D}_1^{-1} + \mathbf{U}_1^\top \mathbf{G}_1(0) \mathbf{U}_1]^{-1} \mathbf{U}_1^\top \mathbf{G}_1(0) \mathbf{P}_{U_1}^\perp (\mathbf{a}^\top, \mathbf{0}_{1 \times T})^\top \\
= & N^{-1} \text{tr}[(T^{-1} \mathbf{Z} \mathbf{Z}^\top)^{-2}] \mathbf{a}^\top \mathbf{P}_V^\perp \Omega^{-1} \mathbf{V} [\mathbf{V}^\top \Omega^{-1} \mathbf{V}]^{-1} \mathbf{V}^\top \Omega^{-1} \mathbf{P}_V^\perp \mathbf{a} [1 + o_p(1)] \\
= & N^{-1} \text{tr}[(T^{-1} \mathbf{Z} \mathbf{Z}^\top)^{-2}] \mathbf{a}^\top \mathbf{P}_V^\perp \Omega^{-1/2} \mathbf{P}_{\Omega^{-1/2} \mathbf{V}}^\perp \Omega^{-1/2} \mathbf{P}_V^\perp \mathbf{a} [1 + o_p(1)]
\end{aligned}$$

Summarizing the above terms, (S.2.5), (S.2.22) and (S.10.5), we have

$$\begin{aligned}
& (\mathbf{a}^\top, \mathbf{0}_{1 \times T}) \mathbf{P}_{U_1}^\perp \mathbf{G}_2(0) \tilde{\Omega} \mathbf{G}_2(0) \mathbf{P}_{U_1}^\perp (\mathbf{a}^\top, \mathbf{0}_{1 \times T})^\top \\
= & N^{-1} \text{tr}[(T^{-1} \mathbf{Z} \mathbf{Z}^\top)^{-2}] \mathbf{a}^\top \mathbf{P}_V^\perp \Omega^{-1/2} (\mathbf{I}_N - \mathbf{P}_{\Omega^{-1/2} \mathbf{V}}^\perp) \Omega^{-1/2} \mathbf{P}_V^\perp \mathbf{a} [1 + o_p(1)] \\
= & N^{-1} \text{tr}[(T^{-1} \mathbf{Z} \mathbf{Z}^\top)^{-2}] [\mathbf{a}^\top \Sigma^{-1} \mathbf{a}] [1 + o_p(1)] \\
= & (T - N)^{-3} T^3 [\mathbf{a}^\top \Sigma^{-1} \mathbf{a}] [1 + o_p(1)].
\end{aligned}$$

Then,

$$\begin{aligned}
& \frac{\mathbf{a}^\top (T^{-1} \mathbf{R} \mathbf{R}^\top)^{-1} \Sigma (T^{-1} \mathbf{R} \mathbf{R}^\top)^{-1} \mathbf{a}}{[\mathbf{a}^\top (T^{-1} \mathbf{R} \mathbf{R}^\top)^{-1} \mathbf{a}]^2} \\
= & \frac{T}{(T - N) \mathbf{a}^\top \Sigma^{-1} \mathbf{a}} [1 + o_p(1)].
\end{aligned}$$

$$\mathbf{a}^\top \mathbf{S}_0^{-1} \Sigma \mathbf{S}_0^{-1} \mathbf{a} = \frac{T^3}{(T-N)^3} \mathbf{a}^\top \Sigma^{-1} \mathbf{a} [1 + o_p(1)] \quad (\text{S.5.4})$$

From (S.5.3) and (S.5.4), we prove (S.1.11).

Moreover, we note that  $\|\mathbf{S}_\tau^{-1} \mathbf{a}\| \asymp \|\mathbf{a}\|$  in probability.

$$\mathbf{S}_0^{-1} - \mathbf{S}_\tau^{-1} = \mathbf{S}_\tau^{-1} (\mathbf{S}_\tau - \mathbf{S}_0) \mathbf{S}_0^{-1} = \tau \mathbf{S}_\tau^{-1} \mathbf{S}_0^{-1}.$$

Thus, (S.5.3) implies that

$$\begin{aligned} \mathbf{a}^\top \mathbf{S}_\tau^{-1} \mathbf{a} &= \mathbf{a}^\top \mathbf{S}_0^{-1} \mathbf{a} - \tau \mathbf{a}^\top \mathbf{S}_\tau^{-1} \mathbf{S}_0^{-1} \mathbf{a} \\ &= \frac{T}{T-N} \mathbf{a}^\top \Sigma^{-1} \mathbf{a} [1 + o_p(1) + O_p(\tau)]. \end{aligned}$$

(S.5.4) implies that

$$\begin{aligned} & \mathbf{a}^\top \mathbf{S}_\tau^{-1} \Sigma \mathbf{S}_\tau^{-1} \mathbf{a} \\ &= \mathbf{a}^\top \mathbf{S}_0^{-1} \Sigma \mathbf{S}_0^{-1} \mathbf{a} - 2\mathbf{a}^\top (\mathbf{S}_0^{-1} - \mathbf{S}_\tau^{-1}) \Sigma \mathbf{S}_0^{-1} \mathbf{a} \\ & \quad + \mathbf{a}^\top (\mathbf{S}_0^{-1} - \mathbf{S}_\tau^{-1}) \Sigma (\mathbf{S}_0^{-1} - \mathbf{S}_\tau^{-1}) \mathbf{a} \\ &= \mathbf{a}^\top \mathbf{S}_0^{-1} \Sigma \mathbf{S}_0^{-1} \mathbf{a} - 2\tau \mathbf{a}^\top \mathbf{S}_\tau^{-1} \mathbf{S}_0^{-1} \Sigma \mathbf{S}_0^{-1} \mathbf{a} \\ & \quad + \tau^2 \mathbf{a}^\top \mathbf{S}_\tau^{-1} \mathbf{S}_0^{-1} \Sigma \mathbf{S}_0^{-1} \mathbf{S}_\tau^{-1} \mathbf{a} \\ &= \frac{T^3}{(T-N)^3} \mathbf{a}^\top \Sigma^{-1} \mathbf{a} [1 + o_p(1) + O_p(\tau + \tau^2)]. \end{aligned}$$

When  $\tau = o(1)$ ,

$$\begin{aligned} & \frac{\mathbf{1}^\top \mathbf{S}_\tau^{-1} \Sigma \mathbf{S}_\tau^{-1} \mathbf{1}}{[\mathbf{1}^\top \mathbf{S}_\tau^{-1} \mathbf{1}]^2} \\ &= \frac{T}{T-N} (\mathbf{1}^\top \Sigma^{-1} \mathbf{1})^{-1} [1 + o_p(1)]. \end{aligned}$$

We prove (S.1.12).

## S.6 Differences between $\Omega$ and $\mathbf{I}_N$

Now we prove (S.1.8)-(S.1.9). We focus on the difference between  $[\mathbf{I}_N + m(-\tau)\Omega]^{-1}$  and  $[1 + m(-\tau)N^{-1}\text{tr}(\Omega)]^{-1}\mathbf{I}_N$ . Without losing generality, we set  $N^{-1}\text{tr}(\Omega) = b$ .

We define  $\mathbf{A} = [\mathbf{I}_N + m(-\tau)\boldsymbol{\Omega}]^{-1/2}$  and  $\mathbf{A}_0 = [1 + m(-\tau)b]^{-1}\mathbf{I}_N$ . Then

$$\begin{aligned} \mathbf{A}^2 - \mathbf{A}_0 &= [\mathbf{I}_N + m(-\tau)\boldsymbol{\Omega}]^{-1} - [\mathbf{I}_N + m(-\tau)b\mathbf{I}_N]^{-1} \\ &= [\mathbf{I}_N + m(-\tau)\boldsymbol{\Omega}]^{-1}m(-\tau)b[\mathbf{I}_N - b^{-1}\boldsymbol{\Omega}][\mathbf{I}_N + m(-\tau)b\mathbf{I}_N]^{-1} \\ &= \frac{m(-\tau)b}{1 + bm(-\tau)}[\mathbf{I}_N + m(-\tau)\boldsymbol{\Omega}]^{-1}[\mathbf{I}_N - b^{-1}\boldsymbol{\Omega}]. \end{aligned}$$

Thus,  $\|\mathbf{A}^2 - \mathbf{A}_0\| = O(\|\mathbf{I}_N - b^{-1}\boldsymbol{\Omega}\|)$ .

$$\mathbf{P}_{[\mathbf{I}_N + m(-\tau)\boldsymbol{\Omega}]^{-1/2}\mathbf{V}} = \mathbf{A}\mathbf{V}[\mathbf{V}^\top \mathbf{A}^2 \mathbf{V}]^{-1}\mathbf{V}^\top \mathbf{A}.$$

Recall (S.2.20) and (S.3.16),

$$\begin{aligned} \mathbf{a}^\top \mathbf{S}_\tau^{-1} \mathbf{a} &= \tau^{-1} \tilde{\mathbf{a}}_\tau^\top \tilde{\mathbf{a}}_\tau [1 + o_p(1)] \\ &= \tau^{-1} \mathbf{a}^\top [\mathbf{I}_N + m(-\tau)\boldsymbol{\Omega}]^{-1/2} (\mathbf{I}_N - \mathbf{P}_{[\mathbf{I}_N + m(-\tau)\boldsymbol{\Omega}]^{-1/2}\mathbf{V}}) [\mathbf{I}_N + m(-\tau)\boldsymbol{\Omega}]^{-1/2} \mathbf{a} [1 + o_p(1)]. \end{aligned}$$

$$\begin{aligned} &\mathbf{a}^\top [\mathbf{I}_N + m(-\tau)\boldsymbol{\Omega}]^{-1/2} (\mathbf{I}_N - \mathbf{P}_{[\mathbf{I}_N + m(-\tau)\boldsymbol{\Omega}]^{-1/2}\mathbf{V}}) [\mathbf{I}_N + m(-\tau)\boldsymbol{\Omega}]^{-1/2} \mathbf{a} \\ &= \mathbf{a}^\top \mathbf{A} [\mathbf{I}_N - \mathbf{A}\mathbf{V}[\mathbf{V}^\top \mathbf{A}^2 \mathbf{V}]^{-1}\mathbf{V}^\top \mathbf{A}] \mathbf{A} \mathbf{a} \\ &= \mathbf{a}^\top \mathbf{A}^2 [\mathbf{I}_N - \mathbf{V}[\mathbf{V}^\top \mathbf{A}^2 \mathbf{V}]^{-1}\mathbf{V}^\top \mathbf{A}^2] \mathbf{a} \\ &= \mathbf{a}^\top \mathbf{A}_0 [\mathbf{I}_N - \mathbf{V}[\mathbf{V}^\top \mathbf{A}_0 \mathbf{V}]^{-1}\mathbf{V}^\top \mathbf{A}_0] \mathbf{a} [1 + O(\|\mathbf{A}^2 - \mathbf{A}_0\|)] \\ &= [1 + m(-\tau)b]^{-1} \mathbf{a}^\top \mathbf{P}_V^\perp \mathbf{a} [1 + O(\|\mathbf{I}_N - b^{-1}\boldsymbol{\Omega}\|)]. \end{aligned} \tag{S.6.1}$$

Thus,

(S.4.10) shows that

$$\begin{aligned} &\mathbf{a}^\top \mathbf{S}_\tau^{-1} \boldsymbol{\Sigma} \mathbf{S}_\tau^{-1} \mathbf{a} \\ &= \frac{\tau^{-2}}{1 - T^{-1}m^2(-\tau)\text{tr}\{\boldsymbol{\Omega}[\mathbf{I}_N + m(-\tau)\boldsymbol{\Omega}]^{-2}\boldsymbol{\Omega}\}} \mathbf{a}^\top [\mathbf{I}_N + m(-\tau)\boldsymbol{\Omega}]^{-1/2} \\ &\quad (\mathbf{I}_N - \mathbf{P}_{[\mathbf{I}_N + m(-\tau)\boldsymbol{\Omega}]^{-1/2}\mathbf{V}}) \boldsymbol{\Omega}^{1/2} [m(-\tau)\boldsymbol{\Omega} + \mathbf{I}_N]^{-1} \boldsymbol{\Omega}^{1/2} \\ &\quad (\mathbf{I}_N - \mathbf{P}_{[\mathbf{I}_N + m(-\tau)\boldsymbol{\Omega}]^{-1/2}\mathbf{V}}) [\mathbf{I}_N + m(-\tau)\boldsymbol{\Omega}]^{-1/2} \mathbf{a} [1 + o_p(1)] \\ &= \frac{\tau^{-2}}{1 - T^{-1}m^2(-\tau)\text{tr}\{\mathbf{A}^4 \boldsymbol{\Omega}^2\}} \mathbf{a}^\top \mathbf{A} (\mathbf{I}_N - \mathbf{P}_{\mathbf{A}\mathbf{V}}) \boldsymbol{\Omega}^{1/2} \mathbf{A}^2 \boldsymbol{\Omega}^{1/2} (\mathbf{I}_N - \mathbf{P}_{\mathbf{A}\mathbf{V}}) \mathbf{A} \mathbf{a} [1 + o_p(1)]. \end{aligned}$$

$$\begin{aligned}
& \text{tr}\{\mathbf{A}^4\Omega^2\} = \text{tr}\{\mathbf{A}^2\Omega^2\mathbf{A}^2\} \\
&= \text{tr}\{\mathbf{A}_0\Omega^2\mathbf{A}_0\} + 2\text{tr}\{\mathbf{A}^2\Omega^2(\mathbf{A}^2 - \mathbf{A}_0)\} + \text{tr}\{(\mathbf{A}^2 - \mathbf{A}_0)\Omega^2(\mathbf{A}^2 - \mathbf{A}_0)\} \\
&= [1 + m(-\tau)b]^{-2}b^2\text{tr}\{\mathbf{I}_N\} + [1 + m(-\tau)b]^{-2}b^2\text{tr}\{(b^{-2}\Omega^2 - \mathbf{I}_N)\} \\
&\quad + \frac{2m(-\tau)b}{1 + m(-\tau)b}\text{tr}\{\mathbf{A}^2\Omega^2[\mathbf{I}_N + m(-\tau)\Omega]^{-1}[\mathbf{I}_N - b^{-1}\Omega]\} \\
&\quad + \text{tr}\left\{\frac{m^2(-\tau)b^2}{[1 + m(-\tau)b]^2}[\mathbf{I}_N + m(-\tau)\Omega]^{-1}[\mathbf{I}_N - b^{-1}\Omega]\Omega^2[\mathbf{I}_N + m(-\tau)\Omega]^{-1}[\mathbf{I}_N - b^{-1}\Omega]\right\} \\
&= [1 + m(-\tau)b]^{-2}b^2N\{1 + O[N^{-1}\text{tr}(b^{-1}\Omega - \mathbf{I}_N) + m(-\tau)\|b^{-1}\Omega - \mathbf{I}_N\|]\}. \tag{S.6.2}
\end{aligned}$$

Note that  $\mathbf{A}\Omega^{1/2} = [\mathbf{I}_N + m(-\tau)\Omega]^{-1/2}\Omega^{1/2} = \Omega^{1/2}[\mathbf{I}_N + m(-\tau)\Omega]^{-1/2} = \Omega^{1/2}\mathbf{A}$ .

$$\begin{aligned}
& \mathbf{a}^\top \mathbf{A}(\mathbf{I}_N - \mathbf{P}_{\mathbf{AV}})\Omega^{1/2}\mathbf{A}^2\Omega^{1/2}(\mathbf{I}_N - \mathbf{P}_{\mathbf{AV}})\mathbf{A}\mathbf{a} \\
&= \mathbf{a}^\top \mathbf{A}(\mathbf{I}_N - \mathbf{P}_{\mathbf{AV}})\mathbf{A}\Omega\mathbf{A}(\mathbf{I}_N - \mathbf{P}_{\mathbf{AV}})\mathbf{A}\mathbf{a} \\
&= \mathbf{a}^\top \mathbf{P}_V^\perp \mathbf{A}(\mathbf{I}_N - \mathbf{P}_{\mathbf{AV}})\mathbf{A}\mathbf{P}_V^\perp \Omega \mathbf{P}_V^\perp \mathbf{A}(\mathbf{I}_N - \mathbf{P}_{\mathbf{AV}})\mathbf{A}\mathbf{P}_V^\perp \mathbf{a} \\
&= b * \mathbf{a}^\top \mathbf{P}_V^\perp \mathbf{A}(\mathbf{I}_N - \mathbf{P}_{\mathbf{AV}})\mathbf{A}\mathbf{P}_V^\perp \mathbf{A}(\mathbf{I}_N - \mathbf{P}_{\mathbf{AV}})\mathbf{A}\mathbf{P}_V^\perp \mathbf{a} + O(\|\mathbf{P}_V^\perp \mathbf{a}\|^2 \|(b^{-1}\Omega - \mathbf{I}_N)\mathbf{P}_V^\perp\|).
\end{aligned}$$

$$\begin{aligned}
& \mathbf{a}^\top \mathbf{P}_V^\perp \mathbf{A}(\mathbf{I}_N - \mathbf{P}_{\mathbf{AV}})\mathbf{A}\mathbf{P}_V^\perp \mathbf{A}(\mathbf{I}_N - \mathbf{P}_{\mathbf{AV}})\mathbf{A}\mathbf{P}_V^\perp \mathbf{a} \\
&= \mathbf{a}^\top \mathbf{P}_V^\perp \mathbf{A}[\mathbf{I}_N - \mathbf{AV}(\mathbf{V}^\top \mathbf{A}^2 \mathbf{V})^{-1} \mathbf{V}^\top \mathbf{A}]\mathbf{A}\mathbf{P}_V^\perp \mathbf{A}[\mathbf{I}_N - \mathbf{AV}(\mathbf{V}^\top \mathbf{A}^2 \mathbf{V})^{-1} \mathbf{V}^\top \mathbf{A}]\mathbf{A}\mathbf{P}_V^\perp \mathbf{a} \\
&= \mathbf{a}^\top \mathbf{P}_V^\perp [\mathbf{I}_N - \mathbf{A}^2 \mathbf{V}(\mathbf{V}^\top \mathbf{A}^2 \mathbf{V})^{-1} \mathbf{V}^\top] \mathbf{A}^2 \mathbf{P}_V^\perp \mathbf{A}^2 [\mathbf{I}_N - \mathbf{V}(\mathbf{V}^\top \mathbf{A}^2 \mathbf{V})^{-1} \mathbf{V}^\top \mathbf{A}^2] \mathbf{P}_V^\perp \mathbf{a} \\
&= [1 + m(-\tau)b]^{-2} \mathbf{a}^\top \mathbf{P}_V^\perp \mathbf{a} [1 + O(\|(\mathbf{A}^2 - \mathbf{A}_0)\mathbf{P}_V^\perp\|)] \\
&= [1 + m(-\tau)b]^{-2} \mathbf{a}^\top \mathbf{P}_V^\perp \mathbf{a} [1 + O(\|(\mathbf{I}_N - b^{-1}\Omega)\mathbf{P}_V^\perp\|)].
\end{aligned}$$

The third equation is based on (S.9.2).

Then

$$\begin{aligned}
& \mathbf{a}^\top \mathbf{A}\mathbf{P}_V^\perp \mathbf{A}^{-1}\Omega^{1/2}\mathbf{A}^4\Omega^{1/2}\mathbf{A}^{-1}\mathbf{P}_V^\perp \mathbf{A}\mathbf{a} \\
&= b[1 + m(-\tau)b]^{-2} \mathbf{a}^\top \mathbf{P}_V^\perp \mathbf{a} [1 + O(\|(\mathbf{I}_N - b^{-1}\Omega)\mathbf{P}_V^\perp\|)] + O(\|\mathbf{P}_V^\perp \mathbf{a}\|^2 \|(\mathbf{I}_N - b^{-1}\Omega)\mathbf{P}_V^\perp\|) \\
&= b[1 + m(-\tau)b]^{-2} \mathbf{a}^\top \mathbf{P}_V^\perp \mathbf{a} [1 + O(\|(\mathbf{I}_N - b^{-1}\Omega)\mathbf{P}_V^\perp\|)]. \tag{S.6.3}
\end{aligned}$$

From (S.6.1) and (S.6.3), we prove (S.1.8).

When  $\Omega = \sigma^2 \mathbf{I}_N$ , (S.1.8) and (S.2.5) imply that

$$\mathbb{V}(\hat{\boldsymbol{\omega}}_\tau) = \sigma^2 c(\tau) \frac{1 + o_p(1)}{[\mathbf{1}^\top \mathbf{P}_V^\perp \mathbf{1}]} = c(\tau) [\mathbf{1}^\top \boldsymbol{\Sigma}^{-1} \mathbf{1}]^{-1} [1 + o_p(1)].$$

with

$$\begin{aligned} c(\tau) &= \frac{1}{1 - T^{-1} m^2(-\tau) \sigma^4 \text{tr}\{[1 + m(-\tau) \sigma^2]^{-2} \mathbf{I}_N\}} \\ &= \frac{1}{1 - \gamma m^2(-\tau) \sigma^4 [1 + m(-\tau) \sigma^2]^{-2}}. \end{aligned}$$

Since  $\boldsymbol{\Omega} = \sigma^2 \mathbf{I}_N$  and  $\tau = o(1)$ , (S.10.2) shows that

$$m(-\tau) = \frac{\sigma^{-2}}{\gamma - 1} [1 + o(1)].$$

Then

$$\begin{aligned} c(\tau) &= \frac{1}{1 - T^{-1} m^2(-\tau) \text{tr}\{[1 + m(-\tau)]^{-2} \mathbf{I}_N\}} \\ &= \frac{1}{1 - \gamma m^2(-\tau) \sigma^4 [1 + m(-\tau) \sigma^2]^{-2}} \\ &= \frac{1}{1 - \gamma \frac{1}{[\gamma - 1]^2} [1 + \frac{1}{\gamma - 1}]^{-2}} [1 + o(1)] \\ &= \frac{1}{1 - \frac{1}{\gamma}} [1 + o(1)] \\ &= \frac{\gamma}{\gamma - 1} [1 + o(1)]. \end{aligned}$$

We conclude (S.1.9)

## S.7 The case for $\mathbf{S}_{\tau, \Omega}$

In this section, we prove (S.1.13) and (S.1.14). Recall (S.2.2),

$$\mathbb{V}(\tilde{\boldsymbol{\omega}}_\tau^{\text{ifs}}) = \frac{\mathbf{1}^\top \mathbf{S}_{\tau, \Omega}^{-1} \boldsymbol{\Sigma} \mathbf{S}_{\tau, \Omega}^{-1} \mathbf{1}}{[\mathbf{1}^\top \mathbf{S}_{\tau, \Omega}^{-1} \mathbf{1}]^2}$$

with  $\mathbf{S}_{\tau, \Omega} = \tau \boldsymbol{\Omega} + \mathbf{R} \mathbf{R}^\top / T$ . We have

$$\begin{aligned}
& \mathbf{1}^\top \mathbf{S}_{\tau, \Omega}^{-1} \mathbf{1} \\
= & \mathbf{1}^\top [\tau \Omega + \mathbf{R} \mathbf{R}^\top / T]^{-1} \mathbf{1} \\
= & \mathbf{1}^\top \Omega^{-1/2} [\tau \mathbf{I}_N + \Omega^{-1/2} \mathbf{R} \mathbf{R}^\top \Omega^{-1/2} / T]^{-1} \Omega^{-1/2} \mathbf{1} \\
= & \mathbf{1}^\top \Omega^{-1} \mathbf{1} \mathbf{a}^\top [\tau \mathbf{I}_N + \Omega^{-1/2} \mathbf{R} \mathbf{R}^\top \Omega^{-1/2} / T]^{-1} \mathbf{a}
\end{aligned}$$

and

$$\begin{aligned}
& \mathbf{1}^\top \mathbf{S}_{\tau, \Omega}^{-1} \Sigma \mathbf{S}_{\tau, \Omega}^{-1} \mathbf{1} \\
= & \mathbf{1}^\top [\tau \Omega + \mathbf{R} \mathbf{R}^\top / T]^{-1} \Sigma [\tau \Omega + \mathbf{R} \mathbf{R}^\top / T]^{-1} \mathbf{1} \\
= & \mathbf{1}^\top \Omega^{-1/2} [\tau \mathbf{I}_N + \Omega^{-1/2} \mathbf{R} \mathbf{R}^\top \Omega^{-1/2} / T]^{-1} \Omega^{-1/2} \Sigma \Omega^{-1/2} \\
& [\tau \mathbf{I}_N + \Omega^{-1/2} \mathbf{R} \mathbf{R}^\top \Omega^{-1/2} / T]^{-1} \Omega^{-1/2} \mathbf{1} \\
= & \mathbf{1}^\top \Omega^{-1} \mathbf{1} \mathbf{a}^\top [\tau \mathbf{I}_N + \Omega^{-1/2} \mathbf{R} \mathbf{R}^\top \Omega^{-1/2} / T]^{-1} \Omega^{-1/2} \Sigma \Omega^{-1/2} \\
& [\tau \mathbf{I}_N + \Omega^{-1/2} \mathbf{R} \mathbf{R}^\top \Omega^{-1/2} / T]^{-1} \mathbf{a}
\end{aligned}$$

with  $\mathbf{a} = \frac{\Omega^{-1/2} \mathbf{1}}{\|\Omega^{-1/2} \mathbf{1}\|}$  being an unit vector.

Recalling (S.1.1), we have

$$\Omega^{-1/2} \mathbf{R} = \Omega^{-1/2} \mathbf{B} \mathbf{F} + \Omega^{-1/2} \mathbf{E} = \Omega^{-1/2} \mathbf{B} \mathbf{F} + \mathbf{Z}, \quad (\text{S.7.1})$$

$$\Omega^{-1/2} \Sigma \Omega^{-1/2} = \Omega^{-1/2} \mathbf{B} \mathbf{B}^\top \Omega^{-1/2} + \mathbf{I}_N.$$

Thus, we can deal with the following terms

$$\begin{aligned}
& \mathbf{a}^\top [\tau \mathbf{I}_N + \Omega^{-1/2} \mathbf{R} \mathbf{R}^\top \Omega^{-1/2} / T]^{-1} \mathbf{a} \\
& \mathbf{a}^\top [\tau \mathbf{I}_N + \Omega^{-1/2} \mathbf{R} \mathbf{R}^\top \Omega^{-1/2} / T]^{-1} \Omega^{-1/2} \Sigma \Omega^{-1/2} [\tau \mathbf{I}_N + \Omega^{-1/2} \mathbf{R} \mathbf{R}^\top \Omega^{-1/2} / T]^{-1} \mathbf{a}
\end{aligned}$$

by the same method in 3-5.

Thus,

$$\begin{aligned} & \frac{\mathbf{1}^\top \mathbf{S}_{\tau, \Omega}^{-1} \Sigma \mathbf{S}_{\tau, \Omega}^{-1} \mathbf{1}}{[\mathbf{1}^\top \mathbf{S}_{\tau, \Omega}^{-1} \mathbf{1}]^2} \\ = & \frac{[\mathbf{1}^\top \Omega^{-1} \mathbf{1}]^{-1}}{1 - NT^{-1}m_1^2(-\tau)[1 + m_1(-\tau)]^{-2}} \frac{1 + o_p(1)}{\mathbf{a}^\top \mathbf{P}_{\Omega^{-1/2} \mathbf{V}}^\perp \mathbf{a}}. \end{aligned}$$

Since  $\mathbf{a} = \frac{\Omega^{-1/2} \mathbf{1}}{\|\Omega^{-1/2} \mathbf{1}\|}$  and (S.2.5)

$$\begin{aligned} & \mathbf{1}^\top \Omega^{-1} \mathbf{1} * \mathbf{a}^\top \mathbf{P}_{\Omega^{-1/2} \mathbf{V}}^\perp \mathbf{a} \\ = & \mathbf{1}^\top \Omega^{-1/2} \mathbf{P}_{\Omega^{-1/2} \mathbf{V}}^\perp \Omega^{-1/2} \mathbf{1} \\ = & \mathbf{1}^\top \Sigma^{-1} \mathbf{1} [1 + o(1)]. \end{aligned}$$

Recall (S.1.16), the leading term of  $m_1(-\tau)$  is

$$\begin{aligned} & T^{-1} \mathbb{E} \text{tr}[(T^{-1} \mathbf{Z}^\top \mathbf{Z} + \tau \mathbf{I}_T)^{-1}] \\ = & T^{-1} \mathbb{E} \text{tr}[(T^{-1} \mathbf{Z}^\top \mathbf{Z})^{-1}] [1 + o(1)] \\ = & (N - T)^{-1} T [1 + o(1)]. \end{aligned}$$

The last equation is from (S.10.3).

Then we can prove (S.1.13) and (S.1.14).

## S.8 The case for $\mathbf{S}_{\tau, \hat{\Omega}}$

In this section, we prove (S.1.17) and (S.1.18). Recall (S.2.3),

$$\mathbb{V}(\tilde{\omega}_\tau) = \frac{\mathbf{1}^\top \mathbf{S}_{\tau, \hat{\Omega}}^{-1} \Sigma \mathbf{S}_{\tau, \hat{\Omega}}^{-1} \mathbf{1}}{[\mathbf{1}^\top \mathbf{S}_{\tau, \hat{\Omega}}^{-1} \mathbf{1}]^2}$$

with  $\mathbf{S}_{\tau, \hat{\Omega}} = \tau \hat{\Omega} + \mathbf{R} \mathbf{R}^\top / T$ . We have

$$\begin{aligned}
& \mathbf{1}^\top \mathbf{S}_{\tau, \hat{\Omega}}^{-1} \mathbf{1} \\
= & \mathbf{1}^\top [\tau \hat{\Omega} + \mathbf{R} \mathbf{R}^\top / T]^{-1} \mathbf{1} \\
= & \mathbf{1}^\top \hat{\Omega}^{-1/2} [\tau \mathbf{I}_N + \hat{\Omega}^{-1/2} \mathbf{R} \mathbf{R}^\top \hat{\Omega}^{-1/2} / T]^{-1} \hat{\Omega}^{-1/2} \mathbf{1} \\
= & \mathbf{1}^\top \hat{\Omega}^{-1} \mathbf{1} \mathbf{a}^\top [\tau \mathbf{I}_N + \hat{\Omega}^{-1/2} \mathbf{R} \mathbf{R}^\top \hat{\Omega}^{-1/2} / T]^{-1} \mathbf{a}
\end{aligned}$$

and

$$\begin{aligned}
& \mathbf{1}^\top \mathbf{S}_{\tau, \hat{\Omega}}^{-1} \Sigma \mathbf{S}_{\tau, \hat{\Omega}}^{-1} \mathbf{1} \\
= & \mathbf{1}^\top [\tau \hat{\Omega} + \mathbf{R} \mathbf{R}^\top / T]^{-1} \Sigma [\tau \hat{\Omega} + \mathbf{R} \mathbf{R}^\top / T]^{-1} \mathbf{1} \\
= & \mathbf{1}^\top \hat{\Omega}^{-1/2} [\tau \mathbf{I}_N + \hat{\Omega}^{-1/2} \mathbf{R} \mathbf{R}^\top \hat{\Omega}^{-1/2} / T]^{-1} \hat{\Omega}^{-1/2} \Sigma \hat{\Omega}^{-1/2} \\
& [\tau \mathbf{I}_N + \hat{\Omega}^{-1/2} \mathbf{R} \mathbf{R}^\top \hat{\Omega}^{-1/2} / T]^{-1} \hat{\Omega}^{-1/2} \mathbf{1} \\
= & \mathbf{1}^\top \hat{\Omega}^{-1} \mathbf{1} \mathbf{a}^\top [\tau \mathbf{I}_N + \hat{\Omega}^{-1/2} \mathbf{R} \mathbf{R}^\top \hat{\Omega}^{-1/2} / T]^{-1} \hat{\Omega}^{-1/2} \Sigma \hat{\Omega}^{-1/2} \\
& [\tau \mathbf{I}_N + \hat{\Omega}^{-1/2} \mathbf{R} \mathbf{R}^\top \hat{\Omega}^{-1/2} / T]^{-1} \mathbf{a}
\end{aligned}$$

with  $\mathbf{a} = \frac{\hat{\Omega}^{-1/2} \mathbf{1}}{\|\hat{\Omega}^{-1/2} \mathbf{1}\|}$  being an unit vector.

Let  $\Omega_1 = \hat{\Omega}^{-1/2} \Omega^{1/2}$ ,  $\Omega_2 = \Omega_1 \Omega_1^\top$  and  $b = N^{-1} \text{tr}(\Omega_2)$ . Recalling (S.1.1), we have

$$\hat{\Omega}^{-1/2} \mathbf{R} = \hat{\Omega}^{-1/2} \mathbf{B} \mathbf{F} + \hat{\Omega}^{-1/2} \mathbf{E} = \Omega^{-1/2} \mathbf{B} \mathbf{F} + \Omega_1 \mathbf{Z}, \quad (\text{S.8.1})$$

$$\hat{\Omega}^{-1/2} \Sigma \hat{\Omega}^{-1/2} = \hat{\Omega}^{-1/2} \mathbf{B} \mathbf{B}^\top \hat{\Omega}^{-1/2} + \Omega_2.$$

Thus, we can deal with the following terms

$$\begin{aligned}
& \mathbf{a}^\top [\tau \mathbf{I}_N + \hat{\Omega}^{-1/2} \mathbf{R} \mathbf{R}^\top \hat{\Omega}^{-1/2} / T]^{-1} \mathbf{a} \\
& \mathbf{a}^\top [\tau \mathbf{I}_N + \hat{\Omega}^{-1/2} \mathbf{R} \mathbf{R}^\top \hat{\Omega}^{-1/2} / T]^{-1} \hat{\Omega}^{-1/2} \Sigma \hat{\Omega}^{-1/2} [\tau \mathbf{I}_N + \hat{\Omega}^{-1/2} \mathbf{R} \mathbf{R}^\top \hat{\Omega}^{-1/2} / T]^{-1} \mathbf{a}
\end{aligned}$$

by the same method in Sections 3-5.

Note that in this case, the leading term of  $m_{\Omega_1}(-\tau)$  is

$$T^{-1}\mathbb{E}\text{tr}[(T^{-1}\mathbf{Z}^\top\Omega_1^\top\Omega_1\mathbf{Z} + \tau\mathbf{I}_T)^{-1}].$$

Thus, when  $N \gg T$ ,  $m_{\Omega_1}(-\tau) = T[\text{tr}(\Omega_2)]^{-1}[1 + o(1)] \asymp N^{-1}T$ .

Let the  $N \times r$  matrix  $\tilde{\mathbf{V}}$  be the eigenvector matrix of  $\hat{\Omega}^{-1/2}\mathbf{B}\mathbf{B}^\top\hat{\Omega}^{-1/2}$ . Since the  $N \times r$  matrix  $\mathbf{V}$  is the eigenvector matrix of  $\mathbf{B}\mathbf{B}^\top$ , we have

$$\begin{aligned} & \tilde{\mathbf{V}}\tilde{\mathbf{V}}^\top \\ = & \hat{\Omega}^{-1/2}\mathbf{V}[\mathbf{V}^\top\hat{\Omega}^{-1}\mathbf{V}]^{-1}\mathbf{V}^\top\hat{\Omega}^{-1/2} \\ = & \Omega_1\Omega^{-1/2}\mathbf{V}[\mathbf{V}^\top\Omega^{-1/2}\Omega_1^\top\Omega_1\Omega^{-1/2}\mathbf{V}]^{-1}\mathbf{V}^\top\Omega^{-1/2}\Omega_1^\top. \end{aligned}$$

Let  $\mathbf{P}_{\tilde{\mathbf{V}}}^\perp = \mathbf{I}_N - \tilde{\mathbf{V}}\tilde{\mathbf{V}}^\top$ ,  $\mathbf{P}_{\Omega^{-1/2}\mathbf{V}}^\perp = \mathbf{I}_N - \mathbf{P}_{\Omega^{-1/2}\mathbf{V}}$ .

$$\begin{aligned} & \mathbf{a}^\top[\tau\mathbf{I}_N + \hat{\Omega}^{-1/2}\mathbf{R}\mathbf{R}^\top\hat{\Omega}^{-1/2}/T]^{-1}\mathbf{a} \\ = & \tau^{-1}\mathbf{a}^\top[\mathbf{I}_N + m_{\Omega_1}(-\tau)\Omega_2]^{-1/2}(\mathbf{I}_N - \mathbf{P}_{[\mathbf{I}_N + m_{\Omega_1}(-\tau)\Omega_2]^{-1/2}\tilde{\mathbf{V}}})[\mathbf{I}_N + m_{\Omega_1}(-\tau)\Omega_2]^{-1/2}\mathbf{a} \\ & [1 + o_p(1)] \\ = & [1 + m_{\Omega_1}(-\tau)]^{-1}\mathbf{a}^\top\mathbf{P}_{\tilde{\mathbf{V}}}^\perp\mathbf{a}[1 + O(\|(\Omega_2 - b\mathbf{I}_N)\mathbf{P}_{\tilde{\mathbf{V}}}^\perp\|)][1 + o_p(1)]. \end{aligned}$$

$$\begin{aligned} & \mathbf{a}^\top[\tau\mathbf{I}_N + \hat{\Omega}^{-1/2}\mathbf{R}\mathbf{R}^\top\hat{\Omega}^{-1/2}/T]^{-1}\hat{\Omega}^{-1/2}\Sigma\hat{\Omega}^{-1/2}[\tau\mathbf{I}_N + \hat{\Omega}^{-1/2}\mathbf{R}\mathbf{R}^\top\hat{\Omega}^{-1/2}/T]^{-1}\mathbf{a} \\ = & bc_{\Omega_1}(\tau)[1 + m_{\Omega_1}(-\tau)]^{-2}\mathbf{a}^\top\mathbf{P}_{\tilde{\mathbf{V}}}^\perp\mathbf{a}[1 + O(\|(\Omega_2 - b\mathbf{I}_N)\mathbf{P}_{\tilde{\mathbf{V}}}^\perp\|)][1 + o_p(1)] \end{aligned}$$

with

$$c_{\Omega_1}(\tau) = \frac{1}{1 - T^{-1}m_{\Omega_1}^2(-\tau)\text{tr}\{[\mathbf{I}_N + m_{\Omega_1}(-\tau)\Omega_2]^{-2}\Omega_2^2\}}.$$

From Lemma S.6, we have

$$\|\mathbf{P}_{\tilde{\mathbf{V}}}^\perp\mathbf{a}\| = \frac{\|\mathbf{P}_{\tilde{\mathbf{V}}}^\perp\hat{\Omega}^{-1/2}\mathbf{1}\|}{\|\hat{\Omega}^{-1/2}\mathbf{1}\|} \asymp \frac{\|\mathbf{P}_{\tilde{\mathbf{V}}}^\perp\mathbf{1}\|}{\|\hat{\Omega}^{-1/2}\mathbf{1}\|}$$

Note that

$$\mathbf{P}_{\hat{\mathbf{V}}}^\perp \hat{\mathbf{\Omega}}^{-1/2} \mathbf{V} = \mathbf{0}, \quad (\text{S.8.2})$$

$$\mathbf{P}_{\hat{\mathbf{V}}}^\perp \hat{\mathbf{\Omega}}^{-1/2} \mathbf{P}_V^\perp = \mathbf{P}_{\hat{\mathbf{V}}}^\perp \hat{\mathbf{\Omega}}^{-1/2}. \quad (\text{S.8.3})$$

From (S.8.2),

$$\begin{aligned} & \hat{\mathbf{\Omega}}^{1/2} (\mathbf{\Omega}_2 - b\mathbf{I}_N) \mathbf{P}_{\hat{\mathbf{V}}}^\perp \\ = & (\mathbf{\Omega} - b\hat{\mathbf{\Omega}}) \hat{\mathbf{\Omega}}^{-1/2} \mathbf{P}_{\hat{\mathbf{V}}}^\perp \\ = & (\mathbf{\Omega} - b\hat{\mathbf{\Omega}}) \mathbf{P}_V^\perp \hat{\mathbf{\Omega}}^{-1/2} \mathbf{P}_{\hat{\mathbf{V}}}^\perp. \end{aligned}$$

Thus,

$$\begin{aligned} & \frac{\mathbf{1}^\top \mathbf{S}_{\tau, \hat{\mathbf{\Omega}}}^{-1} \mathbf{\Sigma} \mathbf{S}_{\tau, \hat{\mathbf{\Omega}}}^{-1} \mathbf{1}}{[\mathbf{1}^\top \mathbf{S}_{\tau, \hat{\mathbf{\Omega}}}^{-1} \mathbf{1}]^2} \\ = & [\mathbf{1}^\top \hat{\mathbf{\Omega}}^{-1} \mathbf{1}]^{-1} b c_{\mathbf{\Omega}_1}(\tau) [\mathbf{a}^\top \mathbf{P}_{\hat{\mathbf{V}}}^\perp \mathbf{a}]^{-1} [1 + O(\|(\mathbf{\Omega}_2 - b\mathbf{I}_N) \mathbf{P}_{\hat{\mathbf{V}}}^\perp\|)] [1 + o_p(1)] \\ = & b c_{\mathbf{\Omega}_1}(\tau) [\mathbf{1}^\top \hat{\mathbf{\Omega}}^{-1/2} \mathbf{P}_{\hat{\mathbf{V}}}^\perp \hat{\mathbf{\Omega}}^{-1/2} \mathbf{1}]^{-1} [1 + O(\|(\mathbf{\Omega} - b\hat{\mathbf{\Omega}}) \mathbf{P}_V^\perp\|)] [1 + o_p(1)] \end{aligned}$$

Recall (S.2.5) and (S.2.22),

$$\begin{aligned} \mathbf{1}^\top \mathbf{\Sigma}^{-1} \mathbf{1} &= \mathbf{1}^\top \mathbf{\Omega}^{-1/2} \mathbf{P}_{\mathbf{\Omega}^{-1/2} \mathbf{V}}^\perp \mathbf{\Omega}^{-1/2} \mathbf{1} [1 + o(1)] \\ &= \mathbf{1}^\top \mathbf{P}_V^\perp \mathbf{\Omega}^{-1/2} \mathbf{P}_{\mathbf{\Omega}^{-1/2} \mathbf{V}}^\perp \mathbf{\Omega}^{-1/2} \mathbf{P}_V^\perp \mathbf{1} [1 + o(1)]. \end{aligned}$$

Now we consider the relation of

$$b^{-1} \mathbf{1}^\top \hat{\mathbf{\Omega}}^{-1/2} \mathbf{P}_{\hat{\mathbf{V}}}^\perp \hat{\mathbf{\Omega}}^{-1/2} \mathbf{1}$$

and

$$\mathbf{1}^\top \mathbf{P}_V^\perp \mathbf{\Omega}^{-1/2} (\mathbf{I}_N - \mathbf{P}_{\mathbf{\Omega}^{-1/2} \mathbf{V}}) \mathbf{\Omega}^{-1/2} \mathbf{P}_V^\perp \mathbf{1}.$$

From (S.8.3),

$$\begin{aligned}
& \mathbf{1}^\top \widehat{\Omega}^{-1/2} \mathbf{P}_{\widehat{\mathbf{V}}}^\perp \widehat{\Omega}^{-1/2} \mathbf{1} \\
= & \mathbf{1}^\top \mathbf{P}_V^\perp \widehat{\Omega}^{-1/2} \mathbf{P}_{\widehat{\mathbf{V}}}^\perp \widehat{\Omega}^{-1/2} \mathbf{P}_V^\perp \mathbf{1} \\
= & \mathbf{1}^\top \mathbf{P}_V^\perp \widehat{\Omega}^{-1} \mathbf{P}_V^\perp \mathbf{1} - \mathbf{1}^\top \mathbf{P}_V^\perp \widehat{\Omega}^{-1} \mathbf{V} [\mathbf{V}^\top \widehat{\Omega}^{-1} \mathbf{V}]^{-1} \mathbf{V}^\top \widehat{\Omega}^{-1} \mathbf{P}_V^\perp \mathbf{1}
\end{aligned}$$

$$\begin{aligned}
& \mathbf{1}^\top \mathbf{P}_V^\perp \Omega^{-1/2} (\mathbf{I}_N - \mathbf{P}_{\Omega^{-1/2} \mathbf{V}}) \Omega^{-1/2} \mathbf{P}_V^\perp \mathbf{1} \\
= & \mathbf{1}^\top \mathbf{P}_V^\perp \Omega^{-1} \mathbf{P}_V^\perp \mathbf{1} - \mathbf{1}^\top \mathbf{P}_V^\perp \Omega^{-1} \mathbf{V} [\mathbf{V}^\top \Omega^{-1} \mathbf{V}]^{-1} \mathbf{V}^\top \Omega^{-1} \mathbf{P}_V^\perp \mathbf{1}
\end{aligned}$$

From (S.9.2), we can find that, we can find that  $\widehat{\Omega}$  and  $\Omega$  can be replaced by  $\widehat{\Omega} + \mathbf{V} \mathbf{C}_1 \mathbf{V}^\top$  and  $\Omega + \mathbf{V} \mathbf{C}_2 \mathbf{V}^\top$  for any  $\mathbf{C}_1$  and  $\mathbf{C}_2$  satisfying the conditions in Lemma S.9.2. Thus,

$$\begin{aligned}
& \mathbf{1}^\top \widehat{\Omega}^{-1/2} \mathbf{P}_{\widehat{\mathbf{V}}}^\perp \widehat{\Omega}^{-1/2} \mathbf{1} \\
= & b * \mathbf{1}^\top \mathbf{P}_V^\perp \Omega^{-1/2} (\mathbf{I}_N - \mathbf{P}_{\Omega^{-1/2} \mathbf{V}}) \Omega^{-1/2} \mathbf{P}_V^\perp \mathbf{1} [1 + O(\|(\Omega - b\widehat{\Omega}) \mathbf{P}_V^\perp\|)].
\end{aligned}$$

Thus,

$$\begin{aligned}
& \frac{\mathbf{1}^\top \mathbf{S}_{\tau, \widehat{\Omega}}^{-1} \Sigma \mathbf{S}_{\tau, \widehat{\Omega}}^{-1} \mathbf{1}}{[\mathbf{1}^\top \mathbf{S}_{\tau, \widehat{\Omega}}^{-1} \mathbf{1}]^2} \\
= & bc_{\Omega_1}(\tau) [b * \mathbf{1}^\top \mathbf{P}_V^\perp \Omega^{-1/2} (\mathbf{I}_N - \mathbf{P}_{\Omega^{-1/2} \mathbf{V}}) \Omega^{-1/2} \mathbf{P}_V^\perp \mathbf{1}]^{-1} \\
& [1 + O(\|(\Omega - b\widehat{\Omega}) \mathbf{P}_V^\perp\|)] [1 + o_p(1)] \\
= & c_{\Omega_1}(\tau) [\mathbf{1}^\top \Sigma^{-1} \mathbf{1}]^{-1} [1 + O(\|(\Omega - b\widehat{\Omega}) \mathbf{P}_V^\perp\|)] [1 + o_p(1)].
\end{aligned}$$

Then,

$$\begin{aligned}
& \frac{\mathbf{1}^\top \mathbf{S}_{\tau, \widehat{\Omega}}^{-1} \Sigma \mathbf{S}_{\tau, \widehat{\Omega}}^{-1} \mathbf{1}}{[\mathbf{1}^\top \mathbf{S}_{\tau, \widehat{\Omega}}^{-1} \mathbf{1}]^2} \\
= & c_{\Omega_1}(\tau) [\mathbf{1}^\top \Sigma^{-1} \mathbf{1}]^{-1} [1 + O(\|(\Omega - b\widehat{\Omega}) \mathbf{P}_V^\perp\|)] [1 + o_p(1)].
\end{aligned}$$

When  $N \gg T$ ,  $m_{\Omega_1}(-\tau) = O(N^{-1}T)$  and  $c_{\Omega_1}(\tau) = 1 + O(N^{-1}T)$ .

Then we can prove (S.1.17) and (S.1.18).

## S.9 Lemmas about Identifiability

**Lemma S.10** *For any  $r \times r$  matrix  $\mathbf{C}$  and any  $N \times N$  invertible matrix  $\mathbf{A}$  satisfying  $\mathbf{A} + \mathbf{V}\mathbf{C}\mathbf{V}^\top$  is invertible,*

$$[\mathbf{V}^\top(\mathbf{A} + \mathbf{V}\mathbf{C}\mathbf{V}^\top)^{-1}\mathbf{V}]^{-1} = \mathbf{C} + (\mathbf{V}^\top\mathbf{A}^{-1}\mathbf{V})^{-1} \quad (\text{S.9.1})$$

**Proof.**

$$\begin{aligned} & [\mathbf{V}^\top(\mathbf{A} + \mathbf{V}\mathbf{C}\mathbf{V}^\top)^{-1}\mathbf{V}][\mathbf{C} + (\mathbf{V}^\top\mathbf{A}^{-1}\mathbf{V})^{-1}] \\ = & \mathbf{V}^\top(\mathbf{A} + \mathbf{V}\mathbf{C}\mathbf{V}^\top)^{-1}\mathbf{V}\mathbf{C} + \mathbf{V}^\top(\mathbf{A} + \mathbf{V}\mathbf{C}\mathbf{V}^\top)^{-1}\mathbf{V}(\mathbf{V}^\top\mathbf{A}^{-1}\mathbf{V})^{-1} \\ = & \mathbf{V}^\top(\mathbf{A} + \mathbf{V}\mathbf{C}\mathbf{V}^\top)^{-1}\mathbf{V}\mathbf{C}\mathbf{V}^\top\mathbf{A}^{-1}\mathbf{V}(\mathbf{V}^\top\mathbf{A}^{-1}\mathbf{V})^{-1} \\ & + \mathbf{V}^\top(\mathbf{A} + \mathbf{V}\mathbf{C}\mathbf{V}^\top)^{-1}\mathbf{A}\mathbf{A}^{-1}\mathbf{V}(\mathbf{V}^\top\mathbf{A}^{-1}\mathbf{V})^{-1} \\ = & \mathbf{V}^\top(\mathbf{A} + \mathbf{V}\mathbf{C}\mathbf{V}^\top)^{-1}[\mathbf{V}\mathbf{C}\mathbf{V}^\top + \mathbf{A}]\mathbf{A}^{-1}\mathbf{V}(\mathbf{V}^\top\mathbf{A}^{-1}\mathbf{V})^{-1} \\ = & \mathbf{I}_r. \end{aligned}$$

**Lemma S.11** *For any  $r \times r$  symmetric matrix  $\mathbf{C}$  and any  $N \times N$  invertible symmetric matrix  $\mathbf{A}$  satisfying  $\mathbf{B}^2 = (\mathbf{A}^{-2} + \mathbf{V}\mathbf{C}\mathbf{V}^\top)^{-1}$  is invertible,*

$$\mathbf{B}(\mathbf{I}_N - \mathbf{P}_{\mathbf{B}\mathbf{V}})\mathbf{B} = \mathbf{A}(\mathbf{I}_N - \mathbf{P}_{\mathbf{A}\mathbf{V}})\mathbf{A}. \quad (\text{S.9.2})$$

**Proof.** Recall (S.8.2), it's easy to see

$$\begin{aligned} & \mathbf{B}(\mathbf{I}_N - \mathbf{P}_{\mathbf{B}\mathbf{V}})\mathbf{B} \\ = & \mathbf{P}_V^\perp \mathbf{B}(\mathbf{I}_N - \mathbf{P}_{\mathbf{B}\mathbf{V}})\mathbf{B}\mathbf{P}_V^\perp \end{aligned}$$

From (S.2.13)

$$\mathbf{B}^2 = (\mathbf{A}^{-2} + \mathbf{V}\mathbf{C}\mathbf{V}^\top)^{-1} = \mathbf{A}^2 - \mathbf{A}^2\mathbf{V}(\mathbf{C}^{-1} + \mathbf{V}^\top\mathbf{A}^2\mathbf{V})^{-1}\mathbf{V}^\top\mathbf{A}^2$$

$$\begin{aligned}
& \mathbf{P}_{\mathbf{B}\mathbf{V}} \\
&= \mathbf{B}\mathbf{V}[\mathbf{V}^\top \mathbf{B}^2 \mathbf{V}]^{-1} \mathbf{V}^\top \mathbf{B} \\
&= \mathbf{B}\mathbf{V}[\mathbf{V}^\top (\mathbf{A}^{-2} + \mathbf{V}\mathbf{C}\mathbf{V}^\top)^{-1} \mathbf{V}]^{-1} \mathbf{V}^\top \mathbf{B} \\
&= \mathbf{B}\mathbf{V}[\mathbf{C} + (\mathbf{V}^\top \mathbf{A}^2 \mathbf{V})^{-1}] \mathbf{V}^\top \mathbf{B}
\end{aligned}$$

The last equation is from (S.9.1).

$$\begin{aligned}
& \mathbf{I}_N - \mathbf{P}_{\mathbf{B}\mathbf{V}} \\
&= \mathbf{B}\{\mathbf{B}^{-2} - \mathbf{V}[\mathbf{C} + (\mathbf{V}^\top \mathbf{A}^2 \mathbf{V})^{-1}] \mathbf{V}^\top\} \mathbf{B} \\
&= \mathbf{B}\{\mathbf{A}^{-2} + \mathbf{V}\mathbf{C}\mathbf{V}^\top - \mathbf{V}[\mathbf{C} + (\mathbf{V}^\top \mathbf{A}^2 \mathbf{V})^{-1}] \mathbf{V}^\top\} \mathbf{B} \\
&= \mathbf{B}[\mathbf{A}^{-2} - \mathbf{V}(\mathbf{V}^\top \mathbf{A}^2 \mathbf{V})^{-1} \mathbf{V}^\top] \mathbf{B} \\
&= \mathbf{B}\mathbf{A}^{-1}(\mathbf{I}_N - \mathbf{P}_{\mathbf{A}\mathbf{V}})\mathbf{A}^{-1}\mathbf{B}
\end{aligned}$$

$$\begin{aligned}
& \mathbf{B}(\mathbf{I}_N - \mathbf{P}_{\mathbf{B}\mathbf{V}})\mathbf{B} \\
&= \mathbf{P}_V^\perp \mathbf{B}(\mathbf{I}_N - \mathbf{P}_{\mathbf{B}\mathbf{V}})\mathbf{B}\mathbf{P}_V^\perp \\
&= \mathbf{P}_V^\perp \mathbf{B}^2 \mathbf{A}^{-1}(\mathbf{I}_N - \mathbf{P}_{\mathbf{A}\mathbf{V}})\mathbf{A}^{-1} \mathbf{B}^2 \mathbf{P}_V^\perp \\
&= \mathbf{P}_V^\perp [\mathbf{A}^2 - \mathbf{A}^2 \mathbf{V}(\mathbf{C}^{-1} + \mathbf{V}^\top \mathbf{A}^2 \mathbf{V})^{-1} \mathbf{V}^\top \mathbf{A}^2] \mathbf{A}^{-1}(\mathbf{I}_N - \mathbf{P}_{\mathbf{A}\mathbf{V}})\mathbf{A}^{-1} \mathbf{B}^2 \mathbf{P}_V^\perp \\
&= \mathbf{P}_V^\perp [\mathbf{A} - \mathbf{A}^2 \mathbf{V}(\mathbf{C}^{-1} + \mathbf{V}^\top \mathbf{A}^2 \mathbf{V})^{-1} \mathbf{V}^\top \mathbf{A}] (\mathbf{I}_N - \mathbf{P}_{\mathbf{A}\mathbf{V}})\mathbf{A}^{-1} \mathbf{B}^2 \mathbf{P}_V^\perp \\
&= \mathbf{P}_V^\perp \mathbf{A}(\mathbf{I}_N - \mathbf{P}_{\mathbf{A}\mathbf{V}})\mathbf{A}^{-1} \mathbf{B}^2 \mathbf{P}_V^\perp \\
&= \mathbf{P}_V^\perp \mathbf{A}(\mathbf{I}_N - \mathbf{P}_{\mathbf{A}\mathbf{V}})\mathbf{A}^{-1} [\mathbf{A}^2 - \mathbf{A}^2 \mathbf{V}(\mathbf{C}^{-1} + \mathbf{V}^\top \mathbf{A}^2 \mathbf{V})^{-1} \mathbf{V}^\top \mathbf{A}^2] \mathbf{P}_V^\perp \\
&= \mathbf{P}_V^\perp \mathbf{A}(\mathbf{I}_N - \mathbf{P}_{\mathbf{A}\mathbf{V}})\mathbf{A} \mathbf{P}_V^\perp \\
&= \mathbf{A}(\mathbf{I}_N - \mathbf{P}_{\mathbf{A}\mathbf{V}})\mathbf{A}.
\end{aligned}$$

## S.10 Some Useful Calculations

**Lemma S.12** (*Stieltjes transform*) Under the conditions in Definition S.1, let  $\theta_i$  be the  $i$ -th largest eigenvalue of  $\Omega$

$$\frac{1}{m(z)} = -z + T^{-1} \sum_{i=1}^N \frac{\theta_i}{1 + m(z)\theta_i}. \quad (\text{S.10.1})$$

Lemma S.12 is a basic result in random matrix theory.

**Lemma S.13** *Under the conditions in Definition S.1 and Assumptions 1-2, let  $\theta_i$  be the  $i$ -th largest eigenvalue of  $\mathbf{\Omega} = \sigma^2 \mathbf{I}_N$ .*

*Then if  $N/T \rightarrow \gamma \in (1, \infty)$ ,*

$$m(-\tau) = \frac{T}{N-T} \sigma^{-2} [1 + o(1)] = \frac{\sigma^{-2}}{\gamma - 1} [1 + o(1)]. \quad (\text{S.10.2})$$

*Moreover, when  $N/T \rightarrow \gamma \in (1, \infty)$ ,*

$$\text{tr}[(T^{-1} \mathbf{Z}^\top \mathbf{Z})^{-1}] = \frac{T^2}{N-T} [1 + o_p(1)] = \frac{T}{\gamma - 1} [1 + o_p(1)]. \quad (\text{S.10.3})$$

*When  $N/T \rightarrow \gamma \in (0, 1)$*

$$\text{tr}[(T^{-1} \mathbf{Z} \mathbf{Z}^\top)^{-1}] = \frac{NT}{T-N} [1 + o_p(1)] = \frac{N}{1-\gamma} [1 + o_p(1)]. \quad (\text{S.10.4})$$

**Proof.** Since  $\mathbf{\Omega} = \sigma^2 \mathbf{I}_N$ ,  $\theta_i = \sigma^2$  for  $1 \leq i \leq N$ . From (S.10.1),

$$\begin{aligned} \frac{1}{m(-\tau)} &= \tau + T^{-1} \sum_{i=1}^N \frac{\sigma^2}{1 + m(-\tau)\sigma^2} \\ &= \tau + \frac{NT^{-1}\sigma^2}{1 + m(-\tau)\sigma^2} \end{aligned}$$

Thus, when  $N/T \rightarrow \gamma \in (1, \infty)$ ,

$$m(-\tau) = \frac{T}{N-T} \sigma^{-2} [1 + o(1)] = \frac{\sigma^{-2}}{\gamma - 1} [1 + o(1)].$$

Moreover, when  $N > T$ ,

$$\begin{aligned}
& \sigma^{-2} T^{-1} \text{tr}[(T^{-1} \mathbf{Z}^\top \mathbf{Z})^{-1}] \\
&= \sigma^{-2} T^{-1} \mathbb{E} \text{tr}[(T^{-1} \mathbf{Z}^\top \mathbf{Z})^{-1}] [1 + o_p(1)] \\
&= m(0) [1 + o_p(1)] = \frac{T}{N - T} \sigma^{-2}.
\end{aligned}$$

Then  $\text{tr}[(T^{-1} \mathbf{Z}^\top \mathbf{Z})^{-1}] = \frac{T^2}{N - T} [1 + o_p(1)]$ . It concludes (S.10.3). When  $T > N$ , we exchange  $N$  and  $T$  to get  $\text{tr}[(N^{-1} \mathbf{Z} \mathbf{Z}^\top)^{-1}] = \frac{N^2}{T - N} [1 + o_p(1)]$ . It concludes (S.10.4).

**Lemma S.14** *Under Assumptions 1-2, if  $N/T \rightarrow \gamma \in (0, 1)$ ,*

$$N^{-1} \text{tr}[(T^{-1} \mathbf{Z} \mathbf{Z}^\top)^{-2}] = \frac{T^3}{(T - N)^3} [1 + o_p(1)]. \quad (\text{S.10.5})$$

**Proof.** From the basic theoretical properties of linear spectral statistics, it follows that

$$N^{-1} \text{tr}[(T^{-1} \mathbf{Z} \mathbf{Z}^\top)^{-2}] - \mathbb{E} N^{-1} \text{tr}[(T^{-1} \mathbf{Z} \mathbf{Z}^\top)^{-2}] = O_p(T^{-1}).$$

We only need to calculate  $\mathbb{E} N^{-1} \text{tr}[(T^{-1} \mathbf{Z} \mathbf{Z}^\top)^{-2}]$ . Let  $\mathbf{z}_i$  be the  $i$ -th column of  $\mathbf{Z}$  for  $1 \leq i \leq T$ ,

$$\begin{aligned}
& \text{tr}[(T^{-1} \mathbf{Z} \mathbf{Z}^\top)^{-1}] = T^{-1} \text{tr}[\mathbf{Z}^\top (T^{-1} \mathbf{Z} \mathbf{Z}^\top)^{-2} \mathbf{Z}] \\
&= T^{-1} \sum_{i=1}^T \mathbf{z}_i^\top (T^{-1} \mathbf{Z} \mathbf{Z}^\top)^{-2} \mathbf{z}_i \\
&= \sum_{i=1}^T \frac{T^{-1} \mathbf{z}_i^\top (T^{-1} \mathbf{Z} \mathbf{Z}^\top - T^{-1} \mathbf{z}_i \mathbf{z}_i^\top)^{-2} \mathbf{z}_i}{[1 + T^{-1} \mathbf{z}_i^\top (T^{-1} \mathbf{Z} \mathbf{Z}^\top - T^{-1} \mathbf{z}_i \mathbf{z}_i^\top)^{-1} \mathbf{z}_i]^2}.
\end{aligned}$$

Note that  $\mathbf{z}_i$  and  $(T^{-1} \mathbf{Z} \mathbf{Z}^\top - T^{-1} \mathbf{z}_i \mathbf{z}_i^\top)^{-1}$  are independent. Thus,

$$\begin{aligned}
& \mathbb{E} T^{-1} \mathbf{z}_i^\top (T^{-1} \mathbf{Z} \mathbf{Z}^\top - T^{-1} \mathbf{z}_i \mathbf{z}_i^\top)^{-1} \mathbf{z}_i = T^{-1} \mathbb{E} \text{tr}[(T^{-1} \mathbf{Z} \mathbf{Z}^\top - T^{-1} \mathbf{z}_i \mathbf{z}_i^\top)^{-1}] \\
&= T^{-1} \mathbb{E} \text{tr}[(T^{-1} \mathbf{Z} \mathbf{Z}^\top)^{-1}] [1 + O(T^{-1})] \\
&= \frac{N}{T - N} [1 + o(1)].
\end{aligned}$$

$$\begin{aligned}
& \mathbb{E}T^{-1}\mathbf{z}_i^\top(T^{-1}\mathbf{Z}\mathbf{Z}^\top - T^{-1}\mathbf{z}_i\mathbf{z}_i^\top)^{-2}\mathbf{z}_i = T^{-1}\mathbb{E}\text{tr}[(T^{-1}\mathbf{Z}\mathbf{Z}^\top - T^{-1}\mathbf{z}_i\mathbf{z}_i^\top)^{-2}] \\
& = T^{-1}\mathbb{E}\text{tr}[(T^{-1}\mathbf{Z}\mathbf{Z}^\top)^{-2}][1 + O(T^{-1})].
\end{aligned}$$

Thus,

$$\mathbb{E}\text{tr}[(T^{-1}\mathbf{Z}\mathbf{Z}^\top)^{-1}] = \frac{\mathbb{E}\text{tr}[(T^{-1}\mathbf{Z}\mathbf{Z}^\top)^{-2}][1 + O(T^{-1})]}{\{1 + T^{-1}\mathbb{E}\text{tr}[(T^{-1}\mathbf{Z}\mathbf{Z}^\top)^{-1}][1 + O(T^{-1})]\}^2}.$$

(S.10.4) implies that

$$\begin{aligned}
& \mathbb{E}\text{tr}[(T^{-1}\mathbf{Z}\mathbf{Z}^\top)^{-2}] = \mathbb{E}\text{tr}[(T^{-1}\mathbf{Z}\mathbf{Z}^\top)^{-1}]\{1 + T^{-1}\mathbb{E}\text{tr}[(T^{-1}\mathbf{Z}\mathbf{Z}^\top)^{-1}]\}^2[1 + o(1)] \\
& = \frac{NT^3}{(T - N)^3}[1 + o(1)].
\end{aligned}$$

Then we conclude (S.10.5).

**Lemma S.15** (An equality about  $c(\tau)$ ) Under Assumptions 1-2, if  $N/T \rightarrow \gamma \in (1, \infty)$ ,

$$1 < \frac{1 + m(-\tau)\|\mathbf{\Omega}\|_{\min}}{1 + \tau m^2(-\tau)\|\mathbf{\Omega}\|_{\min}} \leq c(\tau) \leq 1 + m(-\tau)\|\mathbf{\Omega}\|. \quad (\text{S.10.6})$$

**Proof.** (S.1.5) implies that

$$c(\tau) = \left[1 - T^{-1} \sum_{i=1}^N \frac{m^2(-\tau)\theta_i^2}{[1 + m(-\tau)\theta_i]^2}\right]^{-1}$$

Here  $\theta_i$  be the  $i$ -th largest eigenvalue of  $\mathbf{\Omega}$ . Since

$$\frac{m(-\tau)\theta_N}{1 + m(-\tau)\theta_N} \leq \frac{m(-\tau)\theta_i}{1 + m(-\tau)\theta_i} \leq \frac{m(-\tau)\theta_1}{1 + m(-\tau)\theta_1},$$

we have

$$\left[1 - \frac{m(-\tau)\theta_N}{1 + m(-\tau)\theta_N} T^{-1} \sum_{i=1}^N \frac{m(-\tau)\theta_i}{1 + m(-\tau)\theta_i}\right]^{-1} \leq c(\tau)$$

and

$$c(\tau) \leq \left[ 1 - \frac{m(-\tau)\theta_1}{1 + m(-\tau)\theta_1} T^{-1} \sum_{i=1}^N \frac{m(-\tau)\theta_i}{1 + m(-\tau)\theta_i} \right]^{-1}.$$

Moreover (S.10.1) implies that

$$T^{-1} \sum_{i=1}^N \frac{m(-\tau)\theta_i}{1 + m(-\tau)\theta_i} = 1 - \tau m(-\tau).$$

Here we note that  $\tau = o(1)$  and  $m(-\tau) > 0$  is finite, thus  $0 < \tau m(-\tau) < 1$  and

$$0 < 1 - \tau m(-\tau) \leq 1.$$

Thus

$$\begin{aligned} c(\tau) &\leq \left[ 1 - \frac{m(-\tau)\theta_1}{1 + m(-\tau)\theta_1} T^{-1} \sum_{i=1}^N \frac{m(-\tau)\theta_i}{1 + m(-\tau)\theta_i} \right]^{-1} \\ &\leq \left[ 1 - \frac{m(-\tau)\theta_1}{1 + m(-\tau)\theta_1} \right]^{-1} \\ &= 1 + m(-\tau)\theta_1. \end{aligned}$$

$$\begin{aligned} c(\tau) &\geq \left[ 1 - \frac{m(-\tau)\theta_N}{1 + m(-\tau)\theta_N} T^{-1} \sum_{i=1}^N \frac{m(-\tau)\theta_i}{1 + m(-\tau)\theta_i} \right]^{-1} \\ &= \left[ 1 - \frac{m(-\tau)\theta_N}{1 + m(-\tau)\theta_N} \{1 - \tau m(-\tau)\} \right]^{-1} \\ &= \frac{1 + m(-\tau)\theta_N}{1 + \tau m^2(-\tau)\theta_N} \\ &> 1. \end{aligned}$$

The last inequality is from  $\tau m(-\tau) < 1$ .

## References

- Bai, Z., B. Miao, and G. Pan (2007). On the asymptotics of eigenvectors of large sample covariance matrix. *Annals of Probability* 35(4), 1532–1572.
- Ding, X. and F. Yang (2018). A necessary and sufficient condition for edge universality at the largest singular values of covariance matrices. *Annals of Applied Probability* 28, 1679–1738.
- Knowles, A. and J. Yin (2017). Anisotropic local laws for random matrices. *Probability Theory and Related Fields* 169, 257–352.
- Yang, F. (2019). Edge universality of separable covariance matrices. *Electronic Journal of Probability* 24, 57.
